# Supplementary material for: CreDes: Causal Reasoning Enhancement and Dual-End Searching for Solving Long-Range Reasoning Problems using LLMs
Source: arXiv:2410.01696 source file (2024-10-02)
Supplement: Supplementary file 1 [file appendix.tex]

\section{Attribution}\label{app:attribution}

We provide attribution for the icons used in \cref{fig:overview} here. The code icon was obtained from \href{https://www.flaticon.com/free-icon/code\_3573187?term=code&page=1&position=1&origin=search&related\_id=3573187}{flaticon.com} and created by Royyan Wijaya. The Chinese icon was obtained from \href{https://www.flaticon.com/free-icon/dragon\_3552304?term=chinese&page=1&position=29&origin=search&related\_id=3552304}{flaticon.com} and created by Freepik. The bot icon was obtained from \href{https://www.flaticon.com/free-icon/bot\_15107346?term=robot&page=1&position=31&origin=search&related\_id=15107346}{flaticon.com} and created by Nuriali. The math icon was obtained from \href{https://www.flaticon.com/free-icon/calculator\_15798843?term=math&page=1&position=7&origin=search&related\_id=15798843}{flaticon.com} and created by widphic. The length icon was obtained from \href{https://www.freepik.com/icon/measuring-tool\_7416244#fromView=search&page=1&position=20&uuid=37894940-a4bb-46c5-8113-bd195e33359d}{freepik.com} and created by Surang Lineal. Finally, the readability icon was obtained from \href{https://www.freepik.com/icon/guidelines\_8463884#fromView=search&page=1&position=0&uuid=4d763cb1-7646-41bd-90c7-7c422b5ab42e}{freepik.com} and created by Generic Detailed Outline.

\section{Alternative Rating Systems}\label{app:alternatives}

This section explores several alternatives to the exponential rating system that solves the MLE of the logistic loss function, as discussed in \cref{sec:background}. Specifically, we evaluate two extensions to the BT-model and one alternative inspired by the accuracy metric commonly used in benchmarks. We then compare these alternatives with the exponential rating system in terms of their predictive performance and demonstrate that their added complexity does not result in better predictions.

All models discussed here are compatible with \tool and can be used as substitutes for the MLE-based BT-model used in \cref{sec:experiments}.

\paragraph{Rao-Kupper Model} \citet{raokupper} extend the BT-model to explicitly account for the probability of a draw by introducing a parameter $\theta \in \mathbb{R}, \theta \geq 1$:

\begin{align*}
    P(i \succ j | \gamma_i, \gamma_j) &= \frac{\gamma_i}{\gamma_i + \theta \gamma_j} \\
    P(j \succ i | \gamma_i, \gamma_j) &= \frac{\gamma_j}{\gamma_j + \theta \gamma_i} \\
    P(i \simeq j | \gamma_i, \gamma_j) &= \frac{\gamma_i \gamma_j (\theta^2 - 1)}{(\gamma_j + \theta \gamma_i)(\gamma_i + \theta \gamma_j)}\\
\end{align*}

It can be shown that this model follows from the hypothesis that a judge cannot tell the difference between two answers if the quality of the answers is close to each other. 

\paragraph{Davidson-Model} \citet{davidson1970on} propose a similar modification to include draws, using a parameter $\theta \in \mathbb{R}, \theta \geq 0$:

\begin{align*}
    P(i \succ j | \gamma_i, \gamma_j) &= \frac{\gamma_i}{\gamma_i + \gamma_j + \theta \sqrt{\gamma_i \gamma_j}} \\
    P(j \succ i | \gamma_i, \gamma_j) &= \frac{\gamma_j}{\gamma_i + \gamma_j + \theta \sqrt{\gamma_i \gamma_j}}\\
    P(i \simeq j | \gamma_i, \gamma_j) &= \frac{\theta \sqrt{\gamma_i \gamma_j}}{\gamma_i + \gamma_j + \theta \sqrt{\gamma_i \gamma_j}} \\
\end{align*}

\paragraph{Accuracy-Based Model} Both extensions to the BT-model presented above still model ratings using an exponential function. However, for LLMs, it could be beneficial to use ratings directly comparable to standard benchmark accuracies. Benchmarks can be viewed as a series of games where, for a given question $Q$, model $m_1$ defeats model $m_2$ if $m_1$ answers correctly and $m_2$ does not. A draw occurs if both answer correctly or incorrectly and otherwise $m_2$ wins. 

Let $\text{Acc}_D$ denote the accuracy function on benchmark $D$. If we model draws as $0.5$ points for each model, the win rates can be expressed as:
\begin{align*}
    P(i \succ j | m_i, m_j) &= \frac{1}{2} \Big(1 + \text{Acc}_D(m_1) - \text{Acc}_D(m_2)\Big)\\
    P(j \succ i | m_i, m_j) &= \frac{1}{2} \Big(1 + \text{Acc}_D(m_2) - \text{Acc}_D(m_1)\Big).\\
\end{align*}
To adapt the BT-model to this accuracy-based approach, we modify it as follows:
\begin{align*}
    P(i \succ j | R_i, R_j) &= \min\left(1, \max\left(0, \frac{1}{2} (1 + R_i - R_j)\right)\right)\\
    P(j \succ i | R_i, R_j) &= \min\left(1, \max\left(0, \frac{1}{2} (1 + R_j - R_i)\right)\right),\\
\end{align*}
where the $\min$ and $\max$ functions ensure probabilities remain within the $[0,1]$ range. Fitting this model on a standard accuracy-based benchmark by minimizing the logistic loss from \cref{eq:logistic-loss} would exactly recover the benchmark accuracies (up to a constant shift). In contrast, the exponential used in the standard BT-model would ensure the benchmark would not exactly recover the accuracies. Thus, the ratings obtained with this model would be more directly comparable with accuracies from standard benchmarks.

\paragraph{Comparison} Comparing these models is challenging because the Rao-Kupper and Davidson models include an additional draw prediction. For predictive purposes, we are only interested in the logistic loss $\mathcal{L}$ from \cref{eq:logistic-loss} to determine whether the additional complexity of the Rao-Kupper and Davidson models reduces the value of $\mathcal{L}$ on an unknown test set. Using data from the Chatbot Arena \citep{chatbot_arena}, we compute $\mathcal{L}$ for various training set sizes. For the Davidson and Rao-Kupper models, we add $0.5P(i \simeq j | \gamma_i, \gamma_j)$ to both $P(i \succ j | \gamma_i, \gamma_j)$ and $P(j \succ i | \gamma_i, \gamma_j)$.

Results are shown in \cref{fig:alternatives}. The Roa-Kupper model performs the worst, while the accuracy-based model is only slightly worse than the remaining two. Finally, both the Davidson and BT-model perform almost identically. Due to the extra complexity of the Davidson model and the more frequent use of the BT-model for LLMs, we decided to use the BT-model as a default for \tool.

\begin{figure}[t]
    \centering
    \includegraphics[width=0.6\textwidth]{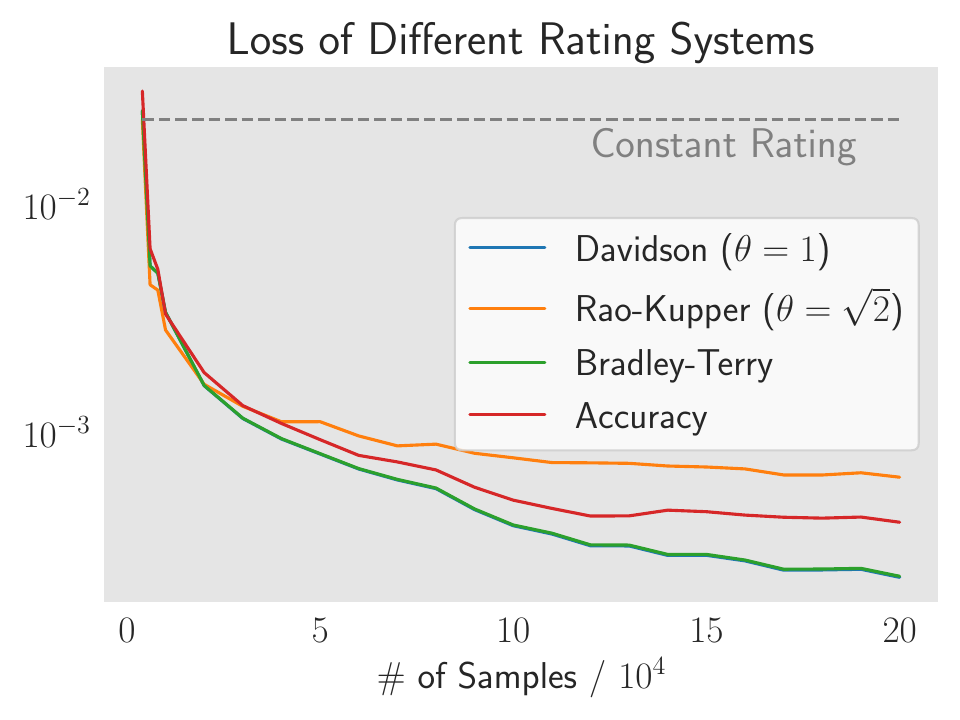}
    \caption{Logistic loss for all four alternatives on the Chatbot Arena dataset for various sizes of the training set.}
    \label{fig:alternatives}
\end{figure}
\newpage
\section{Proofs}\label{app:proofs}

We provide the proofs for the theorems mentioned in the main text here.

We first prove the convexity of the optimization objective in \cref{eq:multi-logistic-loss}.

\begin{theorem}[Convexity of the Optimization Objective]\label{thm:convexity}
    The optimization objective in \cref{eq:multi-logistic-loss} is convex and twice differentiable.
\end{theorem}
\begin{proof}
 Twice differentiability follows immediately from the twice differentiability of the logistic loss and the squared penalty term. To show convexity, we make use of the following well-known facts about convex functions:
    \begin{itemize}
        \item The sum of two convex functions is convex.
        \item The composition of a convex function with an affine function is convex.
    \end{itemize}
Since the logistic loss $f(x) = -\log(1 + \exp(x))$ is convex, and since \tool relies on a linear combination of parameters in the loss function, the logistic loss is convex in these parameters. The squared penalty term is also convex, as it is a sum of squared terms with a positive quadratic coefficient. The sum of two convex functions is convex, so the optimization objective is convex.
\end{proof}

Further, we show the optimality of \tool by showing it converges to the same optimal rating as the univariate approach when fitted on multiple tasks at the same time.

For this purpose, suppose we have a task for which we want to obtain a separate rating. Specifically, let $D$ be a dataset of games between models. Let $D_{\neg \text{task}} \subset D$, resp. $D_{\text{task}}\subset D$, be the set of games not belonging to, resp. belonging to, the task of interest. We show that as $|D| \rightarrow \infty$, the rating obtained by individually fitting the tasks is equivalent to the rating obtained by fitting all tasks simultaneously using \tool. Intuitively, the extra prior term in \tool will be of less importance as the number of games in the task of interest increases, and the ratings will converge to the same optimal rating. 

\begin{theorem} [Equivalence of Ratings]\label{thm:equivalence}
    Let $D$ be a set of i.i.d. games between models $m_0, \dots, m_{k-1}$. Let $D_{\text{task}} \subset D$ and $D_{\neg \text{task}} \subset D$ be as defined above. Let $\mathbf{R}_{\text{task}}$, resp. $\mathbf{R}_{\neg \text{task}}$, be the rating obtained by fitting the games in $D_{\text{task}}$, resp. $D_{\neg \text{task}}$, using the optimal univariate rating system. Let $\mathbf{R'}$ be the rating obtained by fitting all games in $D$ simultaneously using \tool with the formula $R'^{m}(g) = R'^{m}_{\neg \text{task}} + \beta^{m}_{1} \iverson{g \in D_{\text{task}}}$ and define $R'^{m}_{\text{task}} = R'^{m}_{\neg \text{task}} + \beta^{m}_{1}$. Finally, let the priors on respectively $R'^{m}_{\neg \text{task}}$ and $\beta^{m}_{1}$ be $\mathcal{N}(0, \sigma_{\neg \text{task}}^2)$ and $\mathcal{N}(0, \sigma_{1}^2)$. Then, as $|D_{\neg \text{task}}| \rightarrow \infty$ and $|D_{\text{task}}| \rightarrow \infty$, $\mathbf{R}_{\text{task}}$ and $\mathbf{R'}_{\text{task}}$ will, up to a constant difference, converge to the same optimal rating $\mathbf{R}_{\text{task}}^*$  if all optimal ratings are finite. Similarly, $\mathbf{R}_{\neg \text{task}}$ and $\mathbf{R'}_{\neg \text{task}}$ will, up to a constant difference, converge to the same optimal rating $\mathbf{R}_{\neg \text{task}}^*$  if all optimal ratings are finite.
\end{theorem}

To prove the theorem, we first need several lemmas.

\begin{lemma}[Shift-Invarance of Optimal Ratings]\label{lem:shift-invariance}
    Let $D$ be a set of games between models $m_0, \dots, m_{k-1}$ where there exists one model that has played all other models at least once. If $\mathbf{R}_1$ and $\mathbf{R}_2$ both minimize the logistic loss $\mathcal{L}(D, \mathbf{R})$ for $D$, then $\mathbf{R}_1 - \mathbf{R}_2$ is a constant vector.
\end{lemma}

\begin{proof}
    Without loss of generality, we can assume that the first model is the model that has played all other models at least once. We first note that for any constant $c \in \mathbb{R}$, it holds that $\mathcal{L}(D, \mathbf{R} + c) = \mathcal{L}(D, \mathbf{R})$. Therefore, we can assume that the first element of each vector, namely $\mathbf{R}_1^{0}$ and $\mathbf{R}_2^{0}$, are both zero by applying a constant shift to both. We now show that $\mathbf{R}_1=\mathbf{R}_2$. 
    
    We do so by proving that the function $F(x_1, \dots x_{k-1}) = \mathcal{L}(D, (0, x_1, ..., x_{k-1}))$ is strictly convex. Since strictly convex functions have a unique minimum, this implies that $\mathbf{R}_1 = \mathbf{R}_2$. We show strict convexity by computing the Hessian and showing that it is diagonally dominant with strictly positive diagonal elements. By Gershgorin circle theorem, this implies that the Hessian cannot have eigenvalues equal to zero, and is therefore positive definite. Since the Hessian is positive definite, the function is strictly convex, and the result follows.

    We compute the diagonal terms of the Hessian of $F$. We denote by $D_{\{i, j\}}$ all games where one model is $m_i$ and the other model is $m_j$. We slightly change the notation such that the game result $g_r \in D_{\{i, j\}}$ indicates whether $m_i$ won or lost, no matter the order of the models. We define $x_0 = 0$ and drop the division by $400$ for convenience. We have:

    \begin{equation*}
        F(x_1, \dots x_{k-1}) = \sum_{i=0}^{k-1}\sum_{j=0}^{k-1} \sum_{g \in D_{\{i, j\}}} g_r \log(1 + \exp(x_j - x_i))
    \end{equation*}

    Thus,

    \begin{align*}
        \frac{\partial^2 F}{\partial x_i^2} &= \sum_{j=0}^{k - 1}\sum_{g \in D_{\{i, j\}}} g_r \frac{\exp(x_j - x_i)}{(1 + \exp(x_j - x_i))^2}  + (1 - g_r) \frac{\exp(x_i - x_j)}{(1 + \exp(x_i - x_j))^2} \\
        &= \sum_{g \in D_{\{i, 0\}}} g_r \frac{\exp(-x_i)}{(1 + \exp(-x_i))^2}  + (1 - g_r) \frac{\exp(x_i)}{(1 + \exp( x_i))^2} + \sum_{j=1}^{k - 1} -\frac{\partial^2 F}{\partial x_i \partial x_j}\\
    \end{align*}
    Since all terms in the sum are positive, the diagonal terms of the Hessian are strictly positive. Furthermore, the Hessian is diagonally dominant as the last sum is the sum over all off-diagonal terms in the same column and the first sum is strictly positive since $m_i$ has played at least one game against $m_0$. Thus, the Hessian is positive definite, and the function is strictly convex.
\end{proof}

\begin{lemma}[Limit Exists and Is Finite]\label{lem:limit}
    Let $D$ be a set of i.i.d. games between models $m_0, \dots, m_{k-1}$. Furthermore, assume all ratings are bounded. Then,
    \begin{equation}\label{eq:limit:1}
        \lim_{|D| \rightarrow \infty} \frac{1}{|D|} \min_{\mathbf{R}} \mathcal{L}(D, \mathbf{R})
    \end{equation} 
    almost surely uniformly converges to $\mathbb{E}_g(\mathcal{L}(g, \mathbf{R}))$. Furthermore,
    \begin{equation}\label{eq:limit:2}
        \lim_{|D| \rightarrow \infty} \argmin_{\mathbf{R}, \mathbf{R}_0 = 0} \mathcal{L}(D, \mathbf{R})
    \end{equation} 
    almost surely exists and converges to the optimal rating.
\end{lemma}
\begin{proof}
    Let $D_n$ be the first $n$ games in $D$. We show that the functions $\mathcal{L}_n : \mathbb{R}^{k} \rightarrow \mathbb{R}$ defined by $\mathcal{L}_n(\mathbf{R}) = \frac{1}{n} \mathcal{L}(D_n, \mathbf{R})$ converge uniformly to $\mathbb{E}_g(\mathcal{L}(g, \mathbf{R}))$.

    Thus, for any given $\epsilon > 0$ we need to prove the existence of an $N$ such that for all $n > N$ and all $\mathbf{R}$, $|\mathcal{L}_n(\mathbf{R}) - \mathbb{E}_g(\mathcal{L}(g, \mathbf{R}))| < \epsilon$. Let $\epsilon > 0$ be chosen arbitrarily. We can group games with the same models together in the notation for $\mathcal{L}_n$. More specifically, let $w_{i, j}^{(n)}$ denote the weight of the coefficient associated with $\log(1 + \exp(-R_{i}^{m} + R_{j}^{m}))$. Then we can write:
    \begin{equation*}
        \frac{\mathcal{L}_n(\mathbf{R})}{n} = \sum_{i=1}^{k}\sum_{j=1}^{k} \frac{w_{i, j}^{(n)}}{n} \log(1 + \exp(-R_{i}^{m} + R_{j}^{m}))
    \end{equation*}
    Furthermore, we can write the expected value of the loss as:
    \begin{align*}
        \mathbb{E}_g(\mathcal{L}(g, \mathbf{R})) &= \sum_{i=1}^{k}\sum_{j=1}^{k} \left(P(i \succ j) + 0.5 \cdot P(i\simeq j)\right) \cdot P(g \in D_{\{i, j\}}) \log(1 + \exp(-R_{i}^{m} + R_{j}^{m}))\\
        &:= \sum_{i=1}^{k}\sum_{j=1}^{k} P_{i, j}\log(1 + \exp(-R_{i}^{m} + R_{j}^{m}))
    \end{align*}
    where $\simeq$ denotes a draw.

    Thus, we obtain:
    \begin{align*}
        \frac{\mathcal{L}_n(\mathbf{R})}{n} - \mathbb{E}_g(\mathcal{L}(g, \mathbf{R})) = \sum_{i=1}^{k}\sum_{j=1}^{k} & \left(\frac{w_{i, j}^{(n)}}{n} - P_{i, j}\right) \cdot \log(1 + \exp(-R_{i}^{m} + R_{j}^{m}))
    \end{align*}
    By the strong law of large numbers, the weights $w_{i, j}^{(n)} / n$ converge almost surely to the expected value of the weights, i.e. $P_{i, j}$. Furthermore, since the ratings are finite, $\log(1 + \exp(-R_{i}^{m} + R_{j}^{m}))$ can be bounded by a constant $B$. Thus, for any $\epsilon > 0$, there exists an $N$ such that for all $n > N$, $|\frac{w_{i, j}^{(n)}}{n} - P_{i, j}| < \frac{\epsilon}{Bk^2}$ for all $i, j$. Then, almost surely,
    \begin{align*}
        \left|\frac{\mathcal{L}_n(\mathbf{R})}{n} - \mathbb{E}_g(\mathcal{L}(g, \mathbf{R}))\right| &\leqslant \sum_{i=1}^{k}\sum_{j=1}^{k} \left|\frac{w_{i, j}^{(n)}}{n} - P_{i, j}\right| B \\
        &\leqslant  \frac{\epsilon}{Bk^2} \cdot Bk^2 = \epsilon,
    \end{align*}
    proving the first part of the lemma.

    For the second part, we note that \cref{lem:shift-invariance} implies that $\argmin_{\mathbf{R}, \mathbf{R}_0 = 0} \mathcal{L}_n(\mathbf{R})$ has a unique solution. By uniform convergence on a compact domain of continuous functions $\mathcal{L}_n$, we thus have that the limit of the minimizers of $\mathcal{L}_n$ is the minimizer of the expected loss, and the result follows.
\end{proof}

Now, we can prove \cref{thm:equivalence}.

\begin{proof}
We prove that $\mathbf{R}_{\text{task}}$ and $\mathbf{R'}_{\text{task}}$ will converge to the same optimal rating $\mathbf{R}_{\text{task}}^*$ assuming that $\mathbf{R}_{\text{task}, 0} = \mathbf{R'}_{\text{task}, 0} = \mathbf{R}_{\text{task}, 0}^{*} = 0$ which can be assumed due to shift-invariance. The other implication is proven equivalently.

Let $D_\text{task}^{(n)}$ denote the first $n$ elements of $D_\text{task}$ and $\mathbf{R}_{\text{task}}^{(n)}$ the optimal solutions found when fitting using $D_\text{task}^{(n)}$. Note that we leave the size of $D_{\neg \text{task}}$ in the sequence unspecified since it does not matter for this part of the proof. We note that \tool optimizes the loss
\begin{equation}\label{eq:multi-logistic-loss:proof}
    \mathcal{L}^{(n)}_{\text{full}}(D^{(n)}, \mathbf{R'}) = \frac{1}{n}\mathcal{L}(D_{\neg \text{task}}, \mathbf{R'}_{\neg \text{task}}) + \frac{1}{n}\mathcal{L}(D_\text{task}^{(n)}, \mathbf{R'}_{\text{task}}) + \frac{1}{n}\sum_{j=0}^{d} \frac{\mathbf{R'}_{\neg \text{task}, j}^2}{2 \sigma_{\neg \text{task}}^2} + \frac{1}{n} \sum_{j=0}^{d} \frac{\beta_{1, j}^2}{2 \sigma_{1}^2}
\end{equation}
with optimal solution $\mathbf{R'}^{(n)}$. Suppose now that $\mathbf{R'}^{(n)}_{\text{task}}$ does not converge to $\mathbf{R}_{\text{task}}^*$. Then there exists a subsequence $n_i$ and a $\delta > 0$ such that $||\mathbf{R'}_{\text{task}}^{(n_i)} - \mathbf{R}_{\text{task}}^*|| > \delta$. Without loss of generalization, we can assume this subsequence is the full sequence.

By \cref{lem:limit}, we know that $\frac{1}{n}\mathcal{L}(D^{(n)}_{\text{task}}, \mathbf{R})$ uniformly converges to the function $\mathcal{L}^*(\mathbf{R}) := \mathbb{E}_{g_{\text{task}}}(\mathcal{L}(g_{\text{task}}, \mathbf{R}))$ which has $\mathbf{R}_{\text{task}}^*$ as minimizer. By \cref{lem:shift-invariance}, $\mathcal{L}^*$ is continuous and has a unique minimum that satisfies $\mathbf{R}_{\text{task}, 0}^* = 0$. Therefore, there exists an $\epsilon > 0$ such that for all ratings $\mathbf{R}$ with $\mathbf{R}_0 = 0$ the following is true:
\begin{equation}\label{eq:proof:epsilon}
||\mathbf{R} - \mathbf{R}_{\text{task}}^*|| > \delta \Rightarrow \mathcal{L}^*(\mathbf{R}) - \mathcal{L}^*(\mathbf{R}_{\text{task}}^*) > \epsilon.
\end{equation}

Since $\mathbf{R}_{\text{task}}^{(n)}$ converges to $\mathbf{R}_{\text{task}}^*$ by \cref{lem:limit}, we know there is an $n_0 > 0$ such that for each $n > n_0$, 
\begin{equation}\label{eq:proof:epsilon2}
    \mathcal{L}^*(\mathbf{R}_{\text{task}}^{(n)}) - \mathcal{L}^*(\mathbf{R}_{\text{task}}^*) < \frac{\epsilon}{4}. 
\end{equation}

Furthermore, due to the uniform convergence of the loss, there exists an $n_1 > 0$ such that for all $n > n_1$ and all $\mathbf{R}$, 
\begin{equation}\label{eq:proof:uniform}
    \left|\frac{1}{n}\mathcal{L}(D_\text{task}^{(n)}, \mathbf{R}) - \mathcal{L}^*(\mathbf{R})\right| < \frac{\epsilon}{4}.
\end{equation}
Finally, there exists an $n_2 > 0$ such that for all $n > n_2$, 
\begin{equation}\label{eq:proof:epsilon3}
    \left|\frac{d+1}{n}\frac{B^2}{2 \sigma_{\neg \text{task}}^2} + \frac{d+1}{n} \frac{4B^2}{2 \sigma_{1}^2}\right| < \frac{\epsilon}{4}
\end{equation}
where $B$ is the upper bound for all ratings. 

However, we can now define $\mathbf{R''}^{(n)}_{\neg \text{task}} = \mathbf{R'}^{(n)}_{\neg \text{task}}$ and $\beta''^{(n)} = \mathbf{R}_{\text{task}}^{(n)} - \mathbf{R'}^{(n)}_{\neg \text{task}}$. The inequalities above imply that for all $n > \max(n_0, n_1, n_2)$, $\mathcal{L}_{\text{full}}^{(n)}(D^{(n)}, \mathbf{R''}^{(n)}) < \mathcal{L}_{\text{full}}^{(n)}(D^{(n)}, \mathbf{R'}^{(n)})$, since

\begin{align*}
    \frac{1}{n}\mathcal{L}(D_\text{task}^{(n)}, \mathbf{R'}_{\text{task}})  - \frac{1}{n}\mathcal{L}(D_\text{task}^{(n)}, \mathbf{R}_{\text{task}})
    &> \mathcal{L}^*(\mathbf{R'}_{\text{task}}) - \frac{\epsilon}{4} - \mathcal{L}^*(\mathbf{R}_{\text{task}}) - \frac{\epsilon}{4} \\
    &=  \mathcal{L}^*(\mathbf{R'}_{\text{task}})- \mathcal{L}^*(\mathbf{R}^*_{\text{task}}) + \mathcal{L}^*(\mathbf{R}^*_{\text{task}}) - \mathcal{L}^*(\mathbf{R}_{\text{task}})  - \frac{\epsilon}{2} \\
    &> \epsilon - \frac{\epsilon}{4} - \frac{\epsilon}{2} = \frac{\epsilon}{4}
\end{align*}
where the first inequality follows from \cref{eq:proof:uniform} and the last from \cref{eq:proof:epsilon} and \cref{eq:proof:epsilon2}. Since \cref{eq:proof:epsilon3} ensures that the difference in the bias term can at most differ by $\epsilon / 4$, we find $\mathcal{L}_{\text{full}}^{(n)}(D^{(n)}, \mathbf{R''}^{(n)}) < \mathcal{L}_{\text{full}}^{(n)}(D^{(n)}, \mathbf{R'}^{(n)})$. Therefore, $\mathbf{R'}^{(n)}_{\text{task}}$ cannot be the optimal solution, which is a contradiction to the optimality of $\mathbf{R'}^{(n)}$. Therefore, $\mathbf{R'}_{\text{task}}$ must converge to $\mathbf{R}_{\text{task}}^*$.

\end{proof}
\section{Experimental Details}\label{app:details}
In this section, we provide detailed descriptions of the biases and tasks used in our experiments. In \cref{tab:biases:description} we describe the biases used in \cref{sec:experiments:bias} in more detail. In \cref{tab:categories:description} we describe the tasks used in \cref{sec:experiments} in more detail.

We also briefly explain how we adjust the win rates of traditional benchmarks to improve sample efficiency of human evaluation, as discussed in \cref{sec:experiments:convergence}. As detailed in the accuracy-based model in \cref{app:alternatives}, the win rate of $m_1$ over $m_2$ in a traditional benchmark can be written as 
\begin{align*}
    P(i \succ j | m_i, m_j) &= \frac{1}{2} \Big(1 + \text{Acc}_D(m_1) - \text{Acc}_D(m_2)\Big)\\
    P(j \succ i | m_i, m_j) &= \frac{1}{2} \Big(1 + \text{Acc}_D(m_2) - \text{Acc}_D(m_1)\Big).\\
\end{align*}
where $\text{Acc}_D$ is the accuracy function. 

Benchmarks often exhibit significant variation in accuracy differences between models. For instance, in some benchmarks, models may have closely aligned accuracies, while in others, the differences may be substantial. This variation affects the win rate estimates between models. To address this, we introduce a parameter $\mathcal{W}$, which allows us to adjust the scale of win rates. The adjusted win rates are modeled as:
\begin{align*}
    P(i \succ j | m_i, m_j) &= \min\left(1, \frac{\mathcal{W}}{2} \Big(1 + \text{Acc}_D(m_1) - \text{Acc}_D(m_2)\Big)\right)\\
    P(j \succ i | m_i, m_j) &= 1 - P(i \succ j | m_i, m_j).\\
\end{align*}
This adjustment ensures that we can control the scale of win rates, mitigating the issue of varying accuracy differences. We optimize the hyperparameter $\mathcal{W}$ using human evaluations from the training data. Specifically, we fit a univariate rating model using win rates for a given $\mathcal{W}$ on the classical benchmark and evaluate the logistic loss of the resulting ratings on the training data. The parameter with the lowest logistic loss is selected. Importantly, we do not use any unknown test data during this optimization process, ensuring that our approach can be applied in practical scenarios without compromising the integrity of the evaluation.

\begin{table}[t]
    \centering
    \footnotesize
    \caption{Overview of all biases used in \cref{sec:experiments:bias}. The table contains a description of the bias and a functional form of the bias. Scaling constant were introduced in these functional forms to ensure that all biases output values within the same order of magnitude.}
    \label{tab:biases:description}
    \begin{tabular}{>{\raggedright}p{0.11\textwidth} >{\raggedright\arraybackslash}p{0.4\textwidth} >{\raggedright\arraybackslash}p{0.4\textwidth}}
        \toprule
        \textbf{Bias} & \textbf{Description} & \textbf{Functional Form} \\
        \midrule
        Length & Measures the length of a model answer for a given question. & $
        f(g, i) = \log_{10}(\text{length}(g_{m_i}(g_{p})))$\\
        Position & Computes the order of the model in the game. & $f(g, i) = \iverson{i = 1}$\\
        Formality & Computes the formality of an answer computed by a popular formality classifier \citep{formality}.\footnotemark[1] & $f(g, i) = \mathcal{M}(g_{m_i}(g_{p}))_1$ \\
        Sentiment & Computes the sentiment of an answer computed by a popular sentiment classifier \citep{sentiment}.\footnotemark[2] & $f(g, i) = \mathcal{M}(g_{m_i}(g_{p}))_2$\\
        Repetitiveness & Computes the repetitiveness of the answer by computing the percentage of non-unique words in the answer. & $f(g, i) = 5 \cdot \frac{\text{\# of repeated words in }g_{m_i}(g_{p})}{\text{\# of words in }g_{m_i}(g_{p})}$ \\
        Readability & Computes the Flesch Reading Ease score \citep{kincaid1975derivation} of an answer. & $f(g, i) = \min(1, \max(0, \frac{\text{Flesch}(g_{m_i}(g_{p}))}{100}))$\\
        \bottomrule
    \end{tabular}
\end{table}
\footnotetext[1]{{\href{https://huggingface.co/s-nlp/roberta-base-formality-ranker}{https://huggingface.co/s-nlp/roberta-base-formality-ranker}}}
\footnotetext[2]{{\href{https://huggingface.co/cardiffnlp/twitter-roberta-base-sentiment-latest}{https://huggingface.co/cardiffnlp/twitter-roberta-base-sentiment-latest}}}

\begin{table}[t]
    \centering
    \footnotesize
    \caption{Overview of all tasks used in \cref{sec:experiments}. For each task, we use the same data as the actual Chatbot Arena \citep{chatbot_arena}}
    \label{tab:categories:description}
    \begin{tabular}{>{\raggedright}p{0.15\textwidth} >{\raggedright\arraybackslash}p{0.75\textwidth}}
        \toprule
        \textbf{Task} & \textbf{Description} \\
        \midrule
        English & Questions that are in English. \\
        Chinese & Questions that are in Chinese. \\
        Hardness & Questions that are considered hard by the Chatbot Arena. These are questions that are classified as being in at least six of the following seven categories: specific, requires domain knowledge, is complex, requires problem-solving, requires creative thinking, requires technical accuracy, is a real-world question. \\
        Code & Questions that require code to be answered. \\
        LLM & Whether the judge is a language model. \\
        \bottomrule
    \end{tabular}
\end{table}

\newpage
\begin{table}[!ht]
    \centering
    \footnotesize
    \caption{Fitted coefficients for the biases and their average influence on the ratings of the models for both human and LLM-based evaluation. The functional form of $f_{\text{bias}}$ used for each bias can be found in \cref{app:details}. The influence is computed as $\mathbb{E}_g(\alpha_{\text{bias}} \cdot |f_{\text{bias}}(g, 0) - f_{\text{bias}}(g, 1)|)$ and indicates the average influence the bias has on the rating of models for specific games. Errors shown are $95\%$ pivot intervals computed using bootstrapping.}
    \label{tab:biases-full}
    \begin{subtable}[t]{0.48\textwidth}
        \centering
        \caption{Human Evaluation}
        \label{tab:biases:human-full}
        {
        
        \begin{tabular}{lll}
            \toprule
            Bias & {Coefficient $(\alpha)$} & {Influence $(\mathbb{E})$} \\
            \midrule
            
            Length & $\phantom{-}130.74_{-7.3}^{+7.9}$ & $\phantom{-}40.84_{-2.3}^{+2.5}$ \\
            Position & $\phantom{-00}2.70_{-2.4}^{+2.3}$ & $\phantom{-0}2.70_{-2.4}^{+2.3}$ \\
            Formality & $-119.89_{-11.4}^{+11.6}$
 & $-15.17_{-1.4}^{+1.5}$ \\
            Sentiment & $\phantom{-0}57.42_{-10.9}^{+10.1}$ & $\phantom{-0}7.90_{-1.5}^{+1.4}$ \\
            Repetitiveness & $- \phantom{0} 22.10_{-8.4}^{+8.5}$ & $-\phantom{0}4.64_{-1.8}^{+1.8}$ \\
            Readability & $\phantom{-0}72.93_{-11.6}^{+11.0}$ & $\phantom{-}10.75_{-1.7}^{+1.6}$ \\
            
            \bottomrule
        \end{tabular}
        }
    \end{subtable}
    \hfill
    \begin{subtable}[t]{0.48\textwidth}
        \centering
        \caption{LLM-based Evaluation}
        \label{tab:biases:llm-full}
        {
        
        \begin{tabular}{lll}
            \toprule
            Bias & {Coefficient $(\alpha)$} & {Influence $(\mathbb{E})$} \\
            \midrule
            Length & $\phantom{-}251.87_{-6.8}^{+7.3}$ & $\phantom{-}48.48_{-1.3}^{+1.4}$ \\
            Position & $\phantom{-0}37.53_{-1.2}^{+1.1}$ & $\phantom{-}37.53_{-1.2}^{+1.1}$ \\
            Formality & $-\phantom{0}37.56_{-7.2}^{+6.7}$ & $-\phantom{0}4.31_{-0.8}^{+0.8}$ \\
            Sentiment & $\phantom{-00}4.31_{-6.7}^{+6.1}$ & $\phantom{-0}0.43_{-0.7}^{+0.6}$ \\
            Repetitiveness &  $\phantom{-0}75.04_{-7.3}^{+8.8}$ & $\phantom{-0}9.12_{-0.9}^{+1.1}$ \\
            Readability & $-\phantom{0}32.56_{-7.9}^{+8.1}$ & $-\phantom{0}3.92_{-0.9}^{+1.0}$ \\
            \bottomrule
        \end{tabular}
        }
        
    \end{subtable}
    
\end{table}
\newpage
\section{Detailed Results}\label{app:results}

In \cref{tab:biases-full}, we show \cref{tab:biases} with the adjusted confidence intervals computed using pivot intervals instead of $2\sigma$ intervals.

The full multidimensional leaderboard fitted using \tool on Chatbot Arena data \citep{chatbot_arena} can be found in \cref{tab:leaderboard}. The full leaderboard fitted using a unidimensional approach can be found in \cref{tab:leaderboard-single}.

\begin{footnotesize}
    {
    
    \begin{longtable}[t]{lllllll}
        \caption{Leaderboard of human evaluation with modifiers fitted with \tool. Indicated deviations are $95\%$ pivot intervals determined using bootstrapping.} \label{tab:leaderboard} \\
        
        \toprule
        Rank & Model Name & Rating & English & Chinese & Hardness & Code \\
        \midrule
        \endfirsthead
    
        \caption[]{(continued)} \\
        \toprule
        Rank & Model Name & Rating & English & Chinese & Hardness & Code \\
        \midrule
        \endhead
    
        \bottomrule
        \endfoot
    
        \bottomrule
        \endlastfoot
    
        1 & gpt-4o-2024-05-13 & $1297_{-4.2}^{+4.5} $ & $-13_{-10.3}^{+4.3} $ & $-\phantom{00}3_{-8.2}^{+8.8} $ & $\phantom{-} 13_{-4.8}^{+10.0} $ & $\phantom{-} 15_{-5.7}^{+10.4} $ \\
        2 & claude-3-5-sonnet-20240620 & $1286_{-7.4}^{+6.7} $ & $-29_{-13.9}^{+8.2} $ & $-\phantom{0}19_{-12.9}^{+15.0} $ & $\phantom{-} 14_{-8.5}^{+13.6} $ & $\phantom{-} 44_{-10.6}^{+14.9} $ \\
        3 & gemini-advanced-0514 & $1285_{-5.1}^{+4.5} $ & $-26_{-10.7}^{+4.5} $ & $\phantom{-} \phantom{00}8_{-9.4}^{+9.2} $ & $\phantom{-} \phantom{0}3_{-5.6}^{+10.3} $ & $\phantom{-} \phantom{0}2_{-6.9}^{+11.2} $ \\
        4 & gemini-1.5-pro-api-0514 & $1273_{-4.5}^{+4.8} $ & $-20_{-10.5}^{+4.8} $ & $\phantom{-} \phantom{0}19_{-8.6}^{+10.0} $ & $\phantom{-} 15_{-4.8}^{+10.0} $ & $\phantom{-} 11_{-5.8}^{+11.3} $ \\
        5 & claude-3-opus-20240229 & $1273_{-2.7}^{+3.0} $ & $-39_{-9.2}^{+2.5} $ & $\phantom{-} \phantom{00}1_{-5.1}^{+6.0} $ & $\phantom{-} 15_{-2.9}^{+8.4} $ & $\phantom{-} 12_{-3.7}^{+8.4} $ \\
        6 & bard-jan-24-gemini-pro & $1271_{-12.6}^{+12.4} $ & $-48_{-16.9}^{+11.7} $ & $-\phantom{0}25_{-25.8}^{+25.6} $ & $-45_{-11.7}^{+16.9} $ & $-11_{-13.4}^{+19.0} $ \\
        7 & gpt-4-1106-preview & $1265_{-4.0}^{+3.7} $ & $-11_{-9.7}^{+3.5} $ & $-\phantom{00}3_{-7.2}^{+8.0} $ & $\phantom{-} \phantom{0}9_{-3.5}^{+8.7} $ & $\phantom{-} 11_{-4.8}^{+9.3} $ \\
        8 & gemini-1.5-pro-api-0409-preview & $1264_{-4.4}^{+4.6} $ & $-\phantom{0}2_{-10.1}^{+4.1} $ & $\phantom{-} \phantom{00}5_{-8.5}^{+7.9} $ & $-\phantom{0}4_{-4.8}^{+9.8} $ & $-12_{-5.5}^{+10.8} $ \\
        9 & gpt-4-turbo-2024-04-09 & $1258_{-3.4}^{+3.8} $ & $\phantom{-} \phantom{0}3_{-9.8}^{+3.6} $ & $\phantom{-} \phantom{00}4_{-6.6}^{+7.4} $ & $\phantom{-} 11_{-3.8}^{+8.9} $ & $\phantom{-} 15_{-4.9}^{+9.6} $ \\
        10 & gpt-4-0125-preview & $1255_{-3.6}^{+3.6} $ & $-\phantom{0}5_{-9.6}^{+3.5} $ & $\phantom{-} \phantom{00}1_{-6.1}^{+7.3} $ & $\phantom{-} 14_{-3.9}^{+9.0} $ & $\phantom{-} \phantom{0}2_{-4.7}^{+9.5} $ \\
        11 & gemini-1.5-flash-api-0514 & $1243_{-4.5}^{+4.7} $ & $-21_{-10.5}^{+4.5} $ & $\phantom{-} \phantom{00}8_{-9.7}^{+9.5} $ & $\phantom{-} \phantom{0}9_{-5.5}^{+10.4} $ & $\phantom{-} 15_{-6.7}^{+10.8} $ \\
        12 & yi-large-preview & $1237_{-4.4}^{+4.4} $ & $-\phantom{0}4_{-10.6}^{+4.1} $ & $\phantom{-} \phantom{0}37_{-8.6}^{+8.8} $ & $\phantom{-} 17_{-4.8}^{+10.5} $ & $\phantom{-} 11_{-5.8}^{+11.0} $ \\
        13 & gemma-2-27b-it & $1232_{-11.4}^{+11.7} $ & $-10_{-17.6}^{+12.2} $ & $-\phantom{00}1_{-19.6}^{+23.2} $ & $-15_{-13.6}^{+18.0} $ & $\phantom{-} \phantom{0}7_{-15.7}^{+19.9} $ \\
        14 & yi-large & $1222_{-7.7}^{+8.8} $ & $-\phantom{0}3_{-15.5}^{+8.5} $ & $\phantom{-} \phantom{00}9_{-16.5}^{+17.9} $ & $\phantom{-} 11_{-10.4}^{+15.4} $ & $\phantom{-} 21_{-12.5}^{+18.2} $ \\
        15 & nemotron-4-340b-instruct & $1222_{-7.2}^{+6.5} $ & $-13_{-13.1}^{+7.6} $ & $\phantom{-} \phantom{00}7_{-12.4}^{+13.9} $ & $\phantom{-} \phantom{0}9_{-8.5}^{+13.2} $ & $-\phantom{0}6_{-9.4}^{+14.7} $ \\
        16 & claude-3-sonnet-20240229 & $1220_{-3.2}^{+3.3} $ & $-26_{-9.4}^{+2.8} $ & $-\phantom{0}15_{-5.5}^{+5.9} $ & $\phantom{-} \phantom{0}6_{-3.6}^{+8.3} $ & $\phantom{-} 26_{-3.7}^{+9.2} $ \\
        17 & command-r-plus & $1214_{-3.5}^{+3.9} $ & $-18_{-9.4}^{+3.4} $ & $\phantom{-} \phantom{00}6_{-6.4}^{+6.7} $ & $-\phantom{0}7_{-3.7}^{+9.0} $ & $-14_{-4.4}^{+9.3} $ \\
        18 & gpt-4-0314 & $1213_{-4.5}^{+4.5} $ & $-29_{-10.4}^{+4.3} $ & $-\phantom{0}13_{-7.9}^{+8.7} $ & $\phantom{-} 23_{-4.6}^{+9.7} $ & $\phantom{-} \phantom{0}9_{-4.9}^{+10.5} $ \\
        19 & reka-core-20240501 & $1212_{-3.9}^{+3.6} $ & $-11_{-9.8}^{+3.7} $ & $\phantom{-} \phantom{00}9_{-7.6}^{+8.1} $ & $\phantom{-} \phantom{0}6_{-4.7}^{+9.3} $ & $-\phantom{0}2_{-4.6}^{+10.4} $ \\
        20 & claude-3-haiku-20240307 & $1209_{-3.4}^{+3.5} $ & $-30_{-9.2}^{+3.2} $ & $-\phantom{0}36_{-5.2}^{+6.0} $ & $\phantom{-} 10_{-3.4}^{+8.4} $ & $\phantom{-} 16_{-3.6}^{+9.0} $ \\
        21 & gemma-2-9b-it & $1204_{-10.7}^{+11.0} $ & $-17_{-17.5}^{+12.6} $ & $-\phantom{00}1_{-22.1}^{+21.4} $ & $\phantom{-} \phantom{0}3_{-12.6}^{+18.6} $ & $-14_{-16.3}^{+20.3} $ \\
        22 & glm-4-0520 & $1202_{-9.6}^{+10.0} $ & $\phantom{-} \phantom{0}8_{-15.8}^{+10.8} $ & $\phantom{-} \phantom{0}49_{-17.7}^{+17.8} $ & $\phantom{-} 19_{-11.1}^{+15.7} $ & $\phantom{-} 12_{-12.5}^{+17.4} $ \\
        23 & gpt-4-0613 & $1191_{-3.7}^{+3.8} $ & $-22_{-9.5}^{+3.6} $ & $-\phantom{0}41_{-6.5}^{+7.6} $ & $\phantom{-} 18_{-3.7}^{+8.5} $ & $\phantom{-} \phantom{0}1_{-4.2}^{+9.5} $ \\
        24 & claude-1 & $1190_{-8.2}^{+8.3} $ & $-30_{-14.5}^{+7.9} $ & $-\phantom{0}18_{-17.0}^{+16.9} $ & $-19_{-7.6}^{+13.3} $ & $\phantom{-} \phantom{0}4_{-9.4}^{+14.8} $ \\
        25 & reka-flash-preview-20240611 & $1188_{-7.6}^{+7.7} $ & $-15_{-13.8}^{+7.3} $ & $-\phantom{00}5_{-15.0}^{+14.1} $ & $-10_{-9.0}^{+13.8} $ & $\phantom{-} \phantom{0}7_{-10.6}^{+15.4} $ \\
        26 & llama-3-70b-instruct & $1187_{-2.7}^{+3.0} $ & $\phantom{-} 67_{-9.0}^{+2.3} $ & $-\phantom{0}51_{-5.0}^{+5.7} $ & $-\phantom{0}1_{-2.5}^{+7.8} $ & $-10_{-3.3}^{+8.6} $ \\
        27 & qwen-max-0428 & $1187_{-5.1}^{+5.4} $ & $\phantom{-} \phantom{0}3_{-11.6}^{+5.4} $ & $\phantom{-} \phantom{0}62_{-11.3}^{+12.9} $ & $\phantom{-} 11_{-7.1}^{+11.2} $ & $\phantom{-} \phantom{0}8_{-7.9}^{+12.3} $ \\
        28 & qwen2-72b-instruct & $1182_{-6.0}^{+6.0} $ & $\phantom{-} \phantom{0}9_{-12.9}^{+5.4} $ & $\phantom{-} \phantom{0}68_{-11.0}^{+11.9} $ & $\phantom{-} 13_{-6.8}^{+11.6} $ & $-\phantom{0}3_{-7.6}^{+13.4} $ \\
        29 & gemini-pro-dev-api & $1182_{-7.2}^{+8.1} $ & $-38_{-13.6}^{+7.2} $ & $-\phantom{0}23_{-14.0}^{+15.1} $ & $-11_{-8.7}^{+13.3} $ & $-23_{-9.2}^{+14.3} $ \\
        30 & deepseek-coder-v2 & $1181_{-9.3}^{+9.4} $ & $-34_{-15.6}^{+9.6} $ & $\phantom{-} \phantom{0}16_{-17.5}^{+17.3} $ & $\phantom{-} 43_{-11.0}^{+15.5} $ & $\phantom{-} 64_{-11.5}^{+18.1} $ \\
        31 & reka-flash-21b-20240226-online & $1176_{-7.1}^{+6.9} $ & $-12_{-13.3}^{+6.9} $ & $-\phantom{0}10_{-12.1}^{+13.3} $ & $-\phantom{0}2_{-8.1}^{+13.0} $ & $\phantom{-} \phantom{0}1_{-9.4}^{+13.4} $ \\
        32 & command-r & $1175_{-3.9}^{+4.2} $ & $-15_{-9.9}^{+3.9} $ & $\phantom{-} \phantom{0}12_{-6.8}^{+7.5} $ & $-23_{-4.6}^{+9.3} $ & $-\phantom{0}9_{-5.3}^{+10.6} $ \\
        33 & reka-flash-21b-20240226 & $1170_{-5.2}^{+5.6} $ & $-16_{-11.7}^{+5.2} $ & $-\phantom{0}12_{-11.7}^{+10.1} $ & $-\phantom{0}6_{-6.4}^{+11.7} $ & $\phantom{-} \phantom{0}5_{-7.2}^{+11.5} $ \\
        34 & claude-2.0 & $1164_{-10.4}^{+10.8} $ & $-26_{-15.8}^{+9.9} $ & $-\phantom{00}8_{-23.1}^{+24.1} $ & $\phantom{-} \phantom{0}3_{-10.9}^{+15.1} $ & $\phantom{-} 12_{-13.0}^{+17.6} $ \\
        35 & mistral-large-2402 & $1163_{-4.2}^{+4.0} $ & $\phantom{-} \phantom{0}2_{-10.0}^{+3.8} $ & $-\phantom{0}32_{-7.1}^{+7.7} $ & $\phantom{-} 20_{-4.2}^{+9.0} $ & $\phantom{-} 10_{-5.3}^{+9.9} $ \\
        36 & gpt-3.5-turbo-0314 & $1162_{-21.0}^{+19.5} $ & $-56_{-25.0}^{+19.3} $ & $\phantom{-} \phantom{00}9_{-32.4}^{+31.9} $ & $\phantom{-} 22_{-18.2}^{+22.7} $ & $\phantom{-} 14_{-21.9}^{+27.5} $ \\
        37 & qwen1.5-110b-chat & $1161_{-5.0}^{+4.9} $ & $\phantom{-} 12_{-11.0}^{+4.9} $ & $\phantom{-} \phantom{0}58_{-10.5}^{+11.1} $ & $\phantom{-} 10_{-7.2}^{+10.8} $ & $\phantom{-} 11_{-7.8}^{+12.5} $ \\
        38 & gpt-3.5-turbo-0613 & $1161_{-6.3}^{+6.2} $ & $-41_{-11.3}^{+4.9} $ & $-\phantom{0}37_{-14.5}^{+16.2} $ & $\phantom{-} 13_{-6.0}^{+10.5} $ & $\phantom{-} 21_{-7.9}^{+12.1} $ \\
        39 & claude-2.1 & $1156_{-5.7}^{+6.3} $ & $-40_{-11.6}^{+5.3} $ & $-\phantom{0}45_{-11.8}^{+12.2} $ & $\phantom{-} 10_{-5.3}^{+10.8} $ & $\phantom{-} 22_{-6.9}^{+11.8} $ \\
        40 & mistral-next & $1153_{-10.6}^{+11.0} $ & $-20_{-15.2}^{+9.7} $ & $-\phantom{0}50_{-19.4}^{+20.2} $ & $\phantom{-} 14_{-10.4}^{+14.9} $ & $\phantom{-} \phantom{0}8_{-13.2}^{+17.7} $ \\
        41 & mistral-medium & $1153_{-6.0}^{+6.1} $ & $\phantom{-} \phantom{0}9_{-11.4}^{+5.2} $ & $-\phantom{0}24_{-10.7}^{+11.1} $ & $\phantom{-} \phantom{0}5_{-5.8}^{+11.4} $ & $\phantom{-} 11_{-7.2}^{+13.2} $ \\
        42 & mixtral-8x22b-instruct-v0.1 & $1152_{-4.5}^{+4.9} $ & $\phantom{-} \phantom{0}5_{-10.3}^{+4.3} $ & $-\phantom{00}7_{-9.0}^{+8.6} $ & $\phantom{-} 12_{-4.6}^{+10.3} $ & $\phantom{-} \phantom{0}8_{-5.9}^{+10.9} $ \\
        43 & llama-3-8b-instruct & $1150_{-3.4}^{+3.5} $ & $\phantom{-} 48_{-9.3}^{+3.3} $ & $-\phantom{0}41_{-6.0}^{+6.9} $ & $-16_{-3.4}^{+8.5} $ & $-\phantom{0}4_{-4.1}^{+8.7} $ \\
        44 & glm-4-0116 & $1149_{-10.7}^{+9.2} $ & $\phantom{-} 45_{-15.8}^{+10.5} $ & $\phantom{-} \phantom{0}76_{-18.7}^{+19.5} $ & $\phantom{-} 21_{-11.6}^{+17.4} $ & $\phantom{-} 12_{-14.0}^{+18.5} $ \\
        45 & qwen1.5-72b-chat & $1148_{-4.6}^{+5.4} $ & $\phantom{-} 11_{-10.6}^{+4.7} $ & $\phantom{-} \phantom{0}58_{-9.2}^{+9.0} $ & $-\phantom{0}1_{-4.7}^{+10.2} $ & $\phantom{-} 19_{-6.3}^{+11.5} $ \\
        46 & gpt-3.5-turbo-0125 & $1147_{-3.8}^{+4.1} $ & $-38_{-10.1}^{+3.5} $ & $-\phantom{0}46_{-7.1}^{+7.3} $ & $\phantom{-} 11_{-4.4}^{+9.2} $ & $\phantom{-} 19_{-4.5}^{+10.2} $ \\
        47 & zephyr-orpo-141b-A35b-v0.1 & $1143_{-12.2}^{+11.7} $ & $\phantom{-} \phantom{0}4_{-19.4}^{+12.2} $ & $-\phantom{0}27_{-22.2}^{+21.3} $ & $-\phantom{0}2_{-16.2}^{+21.5} $ & $-\phantom{0}1_{-18.9}^{+22.5} $ \\
        48 & gemini-pro & $1139_{-14.6}^{+14.4} $ & $-\phantom{0}7_{-20.4}^{+14.6} $ & $\phantom{-} \phantom{00}2_{-29.5}^{+29.9} $ & $-23_{-14.0}^{+18.7} $ & $-\phantom{0}7_{-17.3}^{+22.2} $ \\
        49 & claude-instant-1 & $1134_{-8.7}^{+8.1} $ & $-13_{-14.0}^{+8.1} $ & $-\phantom{0}15_{-19.0}^{+18.8} $ & $\phantom{-} \phantom{0}7_{-7.8}^{+13.3} $ & $\phantom{-} \phantom{0}3_{-10.7}^{+14.7} $ \\
        50 & wizardlm-70b & $1129_{-13.0}^{+12.7} $ & $\phantom{-} \phantom{0}5_{-17.3}^{+12.8} $ & $-\phantom{0}30_{-28.0}^{+30.0} $ & $-19_{-13.6}^{+17.7} $ & $-26_{-16.3}^{+20.1} $ \\
        51 & snowflake-arctic-instruct & $1126_{-5.0}^{+5.3} $ & $-13_{-11.1}^{+5.2} $ & $-\phantom{00}3_{-9.4}^{+9.8} $ & $-13_{-5.7}^{+10.7} $ & $-11_{-6.7}^{+12.1} $ \\
        52 & qwen1.5-32b-chat & $1126_{-6.0}^{+5.8} $ & $\phantom{-} \phantom{0}5_{-11.7}^{+5.8} $ & $\phantom{-} \phantom{0}69_{-10.4}^{+11.1} $ & $\phantom{-} \phantom{0}8_{-7.1}^{+11.7} $ & $\phantom{-} 22_{-8.9}^{+13.3} $ \\
        53 & yi-1.5-34b-chat & $1126_{-5.9}^{+6.4} $ & $\phantom{-} 63_{-12.2}^{+6.9} $ & $\phantom{-} 103_{-11.4}^{+12.1} $ & $\phantom{-} \phantom{0}5_{-7.6}^{+12.6} $ & $\phantom{-} \phantom{0}1_{-8.9}^{+13.5} $ \\
        54 & phi-3-medium-4k-instruct & $1126_{-7.4}^{+7.3} $ & $\phantom{-} 12_{-13.8}^{+7.9} $ & $-\phantom{00}7_{-13.0}^{+13.0} $ & $\phantom{-} 21_{-8.6}^{+13.5} $ & $\phantom{-} \phantom{0}5_{-11.1}^{+15.2} $ \\
        55 & tulu-2-dpo-70b & $1122_{-13.7}^{+13.4} $ & $-\phantom{0}4_{-19.0}^{+12.4} $ & $-\phantom{0}72_{-28.7}^{+29.7} $ & $\phantom{-} \phantom{0}8_{-12.9}^{+18.6} $ & $-\phantom{0}6_{-16.3}^{+21.1} $ \\
        56 & mixtral-8x7b-instruct-v0.1 & $1114_{-3.8}^{+4.1} $ & $\phantom{-} 25_{-10.2}^{+3.4} $ & $-\phantom{0}37_{-6.9}^{+7.4} $ & $\phantom{-} 10_{-4.0}^{+9.3} $ & $-\phantom{0}4_{-4.8}^{+10.2} $ \\
        57 & openchat-3.5-0106 & $1114_{-8.4}^{+8.7} $ & $-\phantom{0}3_{-14.5}^{+8.5} $ & $-\phantom{00}3_{-14.4}^{+17.0} $ & $-11_{-9.4}^{+14.0} $ & $\phantom{-} 17_{-11.5}^{+15.9} $ \\
        58 & qwen1.5-14b-chat & $1112_{-6.5}^{+6.4} $ & $\phantom{-} 10_{-12.5}^{+6.6} $ & $\phantom{-} \phantom{0}57_{-10.3}^{+11.2} $ & $\phantom{-} \phantom{0}8_{-8.1}^{+12.4} $ & $\phantom{-} 11_{-9.0}^{+14.2} $ \\
        59 & llama2-70b-steerlm-chat & $1111_{-20.2}^{+20.6} $ & $-\phantom{0}3_{-25.7}^{+19.4} $ & $-\phantom{0}28_{-33.8}^{+36.7} $ & $-13_{-19.7}^{+25.0} $ & $-52_{-21.6}^{+25.8} $ \\
        60 & starling-lm-7b-beta & $1111_{-7.1}^{+7.7} $ & $\phantom{-} 19_{-14.1}^{+7.6} $ & $\phantom{-} \phantom{0}35_{-11.3}^{+12.7} $ & $\phantom{-} \phantom{0}1_{-7.7}^{+13.0} $ & $\phantom{-} 18_{-10.5}^{+13.7} $ \\
        61 & llama-2-70b-chat & $1108_{-4.9}^{+5.8} $ & $\phantom{-} 24_{-10.3}^{+4.7} $ & $-\phantom{0}78_{-10.4}^{+10.8} $ & $-18_{-5.8}^{+10.3} $ & $-15_{-7.0}^{+11.1} $ \\
        62 & gpt-3.5-turbo-1106 & $1106_{-8.8}^{+8.7} $ & $-36_{-14.7}^{+8.6} $ & $-\phantom{0}62_{-21.8}^{+22.6} $ & $\phantom{-} 33_{-8.4}^{+14.7} $ & $\phantom{-} 20_{-11.5}^{+15.3} $ \\
        63 & vicuna-33b & $1105_{-7.9}^{+8.2} $ & $\phantom{-} 17_{-12.9}^{+6.6} $ & $-\phantom{0}27_{-14.4}^{+16.3} $ & $-18_{-7.8}^{+12.6} $ & $-18_{-8.9}^{+14.1} $ \\
        64 & phi-3-small-8k-instruct & $1103_{-6.7}^{+7.0} $ & $\phantom{-} 27_{-12.6}^{+7.6} $ & $-\phantom{0}16_{-12.0}^{+12.9} $ & $\phantom{-} 13_{-8.0}^{+13.5} $ & $-\phantom{0}5_{-9.4}^{+15.1} $ \\
        65 & openchat-3.5 & $1101_{-12.9}^{+13.2} $ & $-\phantom{0}5_{-18.3}^{+12.1} $ & $\phantom{-} \phantom{00}2_{-28.3}^{+26.4} $ & $\phantom{-} \phantom{0}2_{-11.6}^{+17.2} $ & $-23_{-16.2}^{+20.5} $ \\
        66 & dbrx-instruct-preview & $1101_{-5.3}^{+5.3} $ & $\phantom{-} 25_{-10.8}^{+4.9} $ & $-\phantom{00}4_{-9.4}^{+9.6} $ & $\phantom{-} \phantom{0}5_{-5.4}^{+10.5} $ & $\phantom{-} 17_{-6.8}^{+12.4} $ \\
        67 & yi-34b-chat & $1101_{-7.9}^{+8.1} $ & $\phantom{-} 36_{-14.4}^{+7.5} $ & $\phantom{-} \phantom{0}94_{-16.5}^{+16.5} $ & $-\phantom{0}6_{-9.8}^{+14.0} $ & $-\phantom{0}6_{-10.0}^{+14.5} $ \\
        68 & starling-lm-7b-alpha & $1099_{-10.4}^{+11.0} $ & $\phantom{-} 17_{-15.8}^{+10.5} $ & $-\phantom{0}17_{-19.9}^{+20.0} $ & $-12_{-11.9}^{+16.3} $ & $-\phantom{0}3_{-12.6}^{+18.1} $ \\
        69 & gemma-1.1-7b-it & $1097_{-6.0}^{+6.0} $ & $\phantom{-} 14_{-11.4}^{+5.9} $ & $-\phantom{00}2_{-10.2}^{+10.4} $ & $-\phantom{0}9_{-6.5}^{+12.2} $ & $\phantom{-} \phantom{0}3_{-8.5}^{+12.7} $ \\
        70 & pplx-70b-online & $1095_{-15.4}^{+12.8} $ & $\phantom{-} 11_{-19.4}^{+15.2} $ & $\phantom{-} \phantom{0}13_{-29.1}^{+31.4} $ & $-39_{-13.8}^{+20.3} $ & $-32_{-16.0}^{+19.9} $ \\
        71 & deepseek-llm-67b-chat & $1092_{-17.2}^{+15.8} $ & $\phantom{-} \phantom{0}0_{-21.6}^{+16.4} $ & $\phantom{-} \phantom{0}46_{-30.4}^{+34.4} $ & $-10_{-16.0}^{+23.9} $ & $\phantom{-} 10_{-20.2}^{+22.9} $ \\
        72 & nous-hermes-2-mixtral-8x7b-dpo & $1090_{-18.6}^{+20.2} $ & $\phantom{-} 25_{-24.8}^{+18.3} $ & $-\phantom{0}26_{-37.1}^{+35.4} $ & $-42_{-16.5}^{+21.5} $ & $\phantom{-} 17_{-21.5}^{+23.0} $ \\
        73 & qwen1.5-7b-chat & $1086_{-13.7}^{+13.4} $ & $-\phantom{0}4_{-19.7}^{+13.7} $ & $\phantom{-} \phantom{0}72_{-22.7}^{+26.1} $ & $-\phantom{0}8_{-15.3}^{+19.6} $ & $\phantom{-} 24_{-18.0}^{+22.5} $ \\
        74 & wizardlm-13b & $1083_{-14.1}^{+14.8} $ & $\phantom{-} \phantom{0}5_{-19.6}^{+12.4} $ & $-\phantom{0}10_{-27.5}^{+26.1} $ & $-41_{-15.9}^{+19.6} $ & $-13_{-19.1}^{+23.0} $ \\
        75 & llama-2-13b-chat & $1081_{-7.9}^{+7.3} $ & $\phantom{-} 12_{-12.7}^{+7.3} $ & $-\phantom{0}58_{-15.9}^{+17.3} $ & $-10_{-7.7}^{+12.9} $ & $-\phantom{0}9_{-10.4}^{+15.0} $ \\
        76 & qwen-14b-chat & $1081_{-16.1}^{+15.3} $ & $-35_{-20.3}^{+16.2} $ & $\phantom{-} \phantom{0}11_{-31.7}^{+35.3} $ & $-17_{-17.9}^{+22.0} $ & $\phantom{-} 33_{-20.4}^{+25.2} $ \\
        77 & vicuna-13b & $1077_{-8.9}^{+8.7} $ & $-15_{-12.9}^{+8.2} $ & $\phantom{-} \phantom{00}7_{-16.9}^{+16.5} $ & $-15_{-9.1}^{+13.8} $ & $\phantom{-} \phantom{0}1_{-10.7}^{+15.2} $ \\
        78 & openhermes-2.5-mistral-7b & $1075_{-14.8}^{+15.1} $ & $\phantom{-} 28_{-20.9}^{+14.7} $ & $-\phantom{0}13_{-29.5}^{+31.0} $ & $\phantom{-} \phantom{0}3_{-16.8}^{+19.7} $ & $-17_{-18.4}^{+23.8} $ \\
        79 & phi-3-mini-128k-instruct & $1072_{-6.3}^{+6.2} $ & $\phantom{-} \phantom{0}0_{-11.9}^{+6.4} $ & $-\phantom{00}2_{-11.6}^{+12.1} $ & $\phantom{-} \phantom{0}0_{-6.9}^{+12.7} $ & $-23_{-8.7}^{+13.4} $ \\
        80 & codellama-34b-instruct & $1070_{-13.1}^{+12.0} $ & $-\phantom{0}5_{-19.1}^{+12.3} $ & $-\phantom{0}57_{-30.6}^{+29.8} $ & $-13_{-13.2}^{+19.3} $ & $\phantom{-} \phantom{0}5_{-17.3}^{+22.4} $ \\
        81 & phi-3-mini-4k-instruct & $1068_{-5.7}^{+6.2} $ & $\phantom{-} 28_{-12.5}^{+6.2} $ & $-\phantom{0}24_{-13.0}^{+13.5} $ & $\phantom{-} 15_{-7.5}^{+12.2} $ & $\phantom{-} 10_{-8.0}^{+13.5} $ \\
        82 & solar-10.7b-instruct-v1.0 & $1064_{-17.8}^{+18.2} $ & $\phantom{-} 27_{-22.0}^{+17.9} $ & $-\phantom{0}23_{-33.3}^{+33.4} $ & $\phantom{-} \phantom{0}2_{-17.3}^{+22.4} $ & $-15_{-21.3}^{+27.7} $ \\
        83 & dolphin-2.2.1-mistral-7b & $1060_{-24.5}^{+25.1} $ & $\phantom{-} 30_{-29.4}^{+24.6} $ & $\phantom{-} \phantom{0}15_{-37.3}^{+37.1} $ & $\phantom{-} \phantom{0}0_{-23.2}^{+29.8} $ & $-31_{-28.0}^{+33.5} $ \\
        84 & vicuna-7b & $1058_{-16.7}^{+16.1} $ & $-36_{-21.5}^{+15.7} $ & $-\phantom{0}37_{-27.6}^{+28.8} $ & $-\phantom{0}3_{-14.6}^{+19.3} $ & $-18_{-18.8}^{+21.4} $ \\
        85 & falcon-180b-chat & $1056_{-29.4}^{+29.7} $ & $\phantom{-} \phantom{0}3_{-34.2}^{+26.8} $ & $-\phantom{0}22_{-34.5}^{+35.1} $ & $-25_{-28.4}^{+32.1} $ & $-\phantom{0}4_{-34.0}^{+40.6} $ \\
        86 & mistral-7b-instruct-v0.2 & $1054_{-7.4}^{+7.9} $ & $\phantom{-} 55_{-12.6}^{+7.4} $ & $-\phantom{00}6_{-12.7}^{+14.3} $ & $-\phantom{0}3_{-8.3}^{+12.4} $ & $\phantom{-} \phantom{0}0_{-9.0}^{+14.1} $ \\
        87 & zephyr-7b-alpha & $1051_{-26.8}^{+24.4} $ & $\phantom{-} 22_{-28.7}^{+26.7} $ & $-\phantom{0}14_{-37.1}^{+39.1} $ & $-18_{-25.8}^{+34.8} $ & $-\phantom{0}2_{-30.5}^{+33.6} $ \\
        88 & zephyr-7b-beta & $1049_{-11.0}^{+11.4} $ & $\phantom{-} 39_{-16.5}^{+10.7} $ & $-\phantom{0}42_{-24.8}^{+25.7} $ & $-22_{-11.5}^{+15.8} $ & $-13_{-12.9}^{+18.7} $ \\
        89 & gemma-1.1-2b-it & $1044_{-8.6}^{+9.0} $ & $\phantom{-} \phantom{0}2_{-15.2}^{+8.4} $ & $\phantom{-} \phantom{00}9_{-16.0}^{+16.3} $ & $-19_{-11.0}^{+16.0} $ & $\phantom{-} 25_{-12.3}^{+16.4} $ \\
        90 & mpt-30b-chat & $1041_{-21.3}^{+20.5} $ & $\phantom{-} 31_{-27.2}^{+20.8} $ & $-\phantom{0}14_{-37.3}^{+38.9} $ & $\phantom{-} 12_{-22.5}^{+29.1} $ & $-20_{-30.0}^{+31.8} $ \\
        91 & codellama-70b-instruct & $1039_{-23.2}^{+24.2} $ & $\phantom{-} 29_{-30.3}^{+26.1} $ & $\phantom{-} \phantom{0}25_{-34.2}^{+36.5} $ & $\phantom{-} \phantom{0}8_{-28.6}^{+33.3} $ & $-\phantom{0}1_{-28.9}^{+36.0} $ \\
        92 & pplx-7b-online & $1038_{-14.6}^{+15.2} $ & $\phantom{-} 35_{-21.0}^{+15.6} $ & $\phantom{-} \phantom{0}21_{-27.8}^{+32.7} $ & $-17_{-15.4}^{+21.6} $ & $-21_{-18.3}^{+22.7} $ \\
        93 & llama-2-7b-chat & $1036_{-8.6}^{+9.3} $ & $\phantom{-} 45_{-15.3}^{+7.9} $ & $-\phantom{0}28_{-19.2}^{+19.0} $ & $-22_{-9.6}^{+14.4} $ & $-31_{-12.3}^{+16.4} $ \\
        94 & guanaco-33b & $1035_{-21.6}^{+20.7} $ & $\phantom{-} 30_{-25.9}^{+21.7} $ & $-\phantom{0}17_{-31.7}^{+33.1} $ & $-12_{-21.4}^{+25.7} $ & $-53_{-27.0}^{+28.1} $ \\
        95 & gemma-7b-it & $1029_{-11.0}^{+11.3} $ & $\phantom{-} 28_{-16.5}^{+10.3} $ & $\phantom{-} \phantom{0}38_{-16.5}^{+18.7} $ & $\phantom{-} 11_{-11.6}^{+17.5} $ & $\phantom{-} \phantom{0}7_{-13.6}^{+16.7} $ \\
        96 & stripedhyena-nous-7b & $1028_{-13.6}^{+15.3} $ & $\phantom{-} 21_{-20.5}^{+14.1} $ & $-\phantom{0}16_{-32.9}^{+35.2} $ & $-19_{-16.2}^{+19.2} $ & $-10_{-18.6}^{+24.2} $ \\
        97 & qwen1.5-4b-chat & $1026_{-10.7}^{+13.0} $ & $-23_{-18.2}^{+11.9} $ & $\phantom{-} \phantom{0}36_{-19.0}^{+19.6} $ & $-13_{-13.2}^{+17.2} $ & $\phantom{-} \phantom{0}4_{-15.4}^{+19.3} $ \\
        98 & mistral-7b-instruct & $1008_{-12.6}^{+11.9} $ & $\phantom{-} 32_{-18.0}^{+11.5} $ & $-\phantom{0}26_{-27.6}^{+26.9} $ & $-\phantom{0}4_{-11.6}^{+18.1} $ & $\phantom{-} \phantom{0}0_{-16.8}^{+19.2} $ \\
        99 & palm-2 & $\phantom{0}997_{-14.4}^{+14.6} $ & $\phantom{-} 43_{-18.9}^{+14.4} $ & $-\phantom{0}69_{-29.6}^{+29.4} $ & $\phantom{-} \phantom{0}0_{-13.2}^{+17.9} $ & $-18_{-16.6}^{+21.7} $ \\
        100 & gemma-2b-it & $\phantom{0}995_{-14.7}^{+13.9} $ & $\phantom{-} 20_{-20.9}^{+15.2} $ & $\phantom{-} \phantom{0}33_{-24.6}^{+26.1} $ & $-\phantom{0}7_{-17.1}^{+19.9} $ & $\phantom{-} \phantom{0}7_{-19.7}^{+25.0} $ \\
        101 & olmo-7b-instruct & $\phantom{0}995_{-13.3}^{+13.4} $ & $\phantom{-} 59_{-18.3}^{+12.6} $ & $\phantom{-} \phantom{0}54_{-21.8}^{+23.7} $ & $-30_{-14.0}^{+18.8} $ & $\phantom{-} \phantom{0}8_{-18.7}^{+21.9} $ \\
        102 & RWKV-4-Raven-14B & $\phantom{0}971_{-19.5}^{+17.6} $ & $-30_{-23.4}^{+17.5} $ & $-\phantom{0}28_{-29.6}^{+30.0} $ & $-23_{-17.6}^{+23.6} $ & $-\phantom{0}7_{-21.3}^{+24.5} $ \\
        103 & koala-13b & $\phantom{0}967_{-17.4}^{+16.6} $ & $\phantom{-} 31_{-22.0}^{+16.6} $ & $-\phantom{0}44_{-24.0}^{+25.5} $ & $-36_{-15.0}^{+19.5} $ & $-\phantom{0}5_{-18.9}^{+21.8} $ \\
        104 & alpaca-13b & $\phantom{0}955_{-17.7}^{+19.8} $ & $-11_{-24.9}^{+18.2} $ & $-\phantom{0}96_{-28.4}^{+28.1} $ & $-62_{-15.3}^{+21.3} $ & $-78_{-21.8}^{+27.9} $ \\
        105 & chatglm3-6b & $\phantom{0}946_{-17.0}^{+16.3} $ & $\phantom{-} 33_{-22.0}^{+17.3} $ & $\phantom{-} 113_{-32.1}^{+30.0} $ & $\phantom{-} \phantom{0}4_{-17.8}^{+21.8} $ & $-\phantom{0}7_{-21.6}^{+25.3} $ \\
        106 & mpt-7b-chat & $\phantom{0}944_{-20.3}^{+20.8} $ & $\phantom{-} \phantom{0}8_{-25.7}^{+20.6} $ & $\phantom{-} \phantom{0}37_{-30.1}^{+30.5} $ & $-25_{-22.6}^{+24.7} $ & $-\phantom{0}7_{-26.0}^{+31.2} $ \\
        107 & chatglm2-6b & $\phantom{0}930_{-19.2}^{+20.7} $ & $\phantom{-} 30_{-25.2}^{+21.2} $ & $\phantom{-} \phantom{0}67_{-37.8}^{+42.2} $ & $-\phantom{0}2_{-24.8}^{+30.3} $ & $-38_{-27.1}^{+31.0} $ \\
        108 & gpt4all-13b-snoozy & $\phantom{0}924_{-27.3}^{+25.1} $ & $\phantom{-} 39_{-29.2}^{+26.6} $ & $-\phantom{00}8_{-31.9}^{+31.0} $ & $\phantom{-} 10_{-24.2}^{+28.9} $ & $-21_{-32.2}^{+33.1} $ \\
        109 & oasst-pythia-12b & $\phantom{0}912_{-18.1}^{+17.6} $ & $\phantom{-} 10_{-21.2}^{+16.6} $ & $-\phantom{0}63_{-25.1}^{+26.3} $ & $-\phantom{0}4_{-18.4}^{+21.3} $ & $-12_{-20.0}^{+26.1} $ \\
        110 & fastchat-t5-3b & $\phantom{0}879_{-19.6}^{+20.8} $ & $\phantom{-} 42_{-24.8}^{+18.6} $ & $-108_{-26.6}^{+28.6} $ & $-36_{-18.6}^{+23.6} $ & $-90_{-24.5}^{+28.8} $ \\
        111 & chatglm-6b & $\phantom{0}874_{-19.1}^{+19.3} $ & $\phantom{-} 11_{-24.3}^{+18.1} $ & $\phantom{-} 199_{-28.7}^{+29.8} $ & $\phantom{-} 18_{-19.5}^{+22.4} $ & $\phantom{-} 11_{-23.1}^{+24.4} $ \\
        112 & dolly-v2-12b & $\phantom{0}856_{-24.2}^{+22.7} $ & $-15_{-27.6}^{+21.9} $ & $\phantom{-} \phantom{00}8_{-30.9}^{+31.1} $ & $\phantom{-} \phantom{0}4_{-22.0}^{+26.2} $ & $-58_{-24.2}^{+30.8} $ \\
        113 & llama-13b & $\phantom{0}853_{-25.8}^{+24.0} $ & $-26_{-28.6}^{+24.4} $ & $-\phantom{00}8_{-27.7}^{+33.2} $ & $-36_{-27.0}^{+28.9} $ & $-89_{-25.1}^{+32.6} $ \\
        114 & stablelm-tuned-alpha-7b & $\phantom{0}843_{-22.2}^{+19.6} $ & $\phantom{-} 19_{-24.7}^{+22.2} $ & $\phantom{-} \phantom{0}30_{-28.5}^{+29.1} $ & $-13_{-20.5}^{+24.0} $ & $\phantom{-} 32_{-23.9}^{+27.9} $ \\
    
    \end{longtable}
    }
    
    \end{footnotesize}

\begin{footnotesize}
    {
    
\begin{longtable}[t]{lllllll}
    \caption{Leaderboard of human evaluation with modifiers when all fitted separately using a unidimensional approach. For the four tasks, modifiers are shown to indicate the deviation from the main rating to make comparison with \tool easier. Indicated deviations are $95\%$ confidence intervals determined using bootstrapping.} \label{tab:leaderboard-single} \\
    
    \toprule
    Rank & Model Name & Rating & English & Chinese & Hardness & Code \\
    \midrule
    \endfirsthead

    \caption[]{(continued)} \\
    \toprule
    Rank & Model Name & Rating & English & Chinese & Hardness & Code \\
    \midrule
    \endhead

    \bottomrule
    \endfoot

    \bottomrule
    \endlastfoot

    1 & gpt-4o-2024-05-13 & $1283_{-2.8}^{+2.7} $ & $-19_{-4.4}^{+4.3} $ & $\phantom{-} \phantom{0}52_{-9.2}^{+9.0} $ & $\phantom{-} \phantom{0}5_{-5.4}^{+5.6} $ & $\phantom{-} 13_{-6.7}^{+6.3} $ \\
2 & claude-3-5-sonnet-20240620 & $1267_{-4.2}^{+4.1} $ & $-23_{-6.9}^{+6.9} $ & $\phantom{-} \phantom{0}45_{-12.1}^{+12.1} $ & $\phantom{-} 11_{-8.8}^{+8.5} $ & $\phantom{-} 35_{-10.0}^{+9.1} $ \\
3 & gemini-advanced-0514 & $1261_{-2.9}^{+2.8} $ & $-28_{-5.1}^{+4.8} $ & $\phantom{-} \phantom{0}69_{-8.9}^{+8.7} $ & $-\phantom{0}8_{-6.1}^{+6.2} $ & $-\phantom{0}4_{-7.5}^{+7.0} $ \\
4 & gemini-1.5-pro-api-0514 & $1259_{-2.9}^{+2.7} $ & $-25_{-4.9}^{+4.8} $ & $\phantom{-} \phantom{0}76_{-8.7}^{+8.5} $ & $\phantom{-} \phantom{0}5_{-5.8}^{+6.1} $ & $\phantom{-} \phantom{0}8_{-7.0}^{+6.8} $ \\
5 & gpt-4-turbo-2024-04-09 & $1252_{-2.3}^{+2.3} $ & $-12_{-4.0}^{+3.7} $ & $\phantom{-} \phantom{0}50_{-7.1}^{+7.4} $ & $\phantom{-} \phantom{0}5_{-4.7}^{+5.1} $ & $\phantom{-} 14_{-5.8}^{+6.0} $ \\
6 & gpt-4-1106-preview & $1248_{-2.3}^{+2.3} $ & $-17_{-3.9}^{+3.4} $ & $\phantom{-} \phantom{0}52_{-7.9}^{+7.5} $ & $\phantom{-} \phantom{0}0_{-5.2}^{+4.9} $ & $\phantom{-} \phantom{0}8_{-5.9}^{+5.6} $ \\
7 & gemini-1.5-pro-api-0409-preview & $1247_{-2.6}^{+2.6} $ & $-16_{-4.0}^{+4.3} $ & $\phantom{-} \phantom{0}55_{-8.5}^{+8.3} $ & $-15_{-5.8}^{+5.5} $ & $-15_{-6.0}^{+6.3} $ \\
8 & claude-3-opus-20240229 & $1245_{-2.1}^{+2.1} $ & $-31_{-3.4}^{+3.4} $ & $\phantom{-} \phantom{0}70_{-6.6}^{+6.6} $ & $\phantom{-} \phantom{0}3_{-4.3}^{+4.3} $ & $\phantom{-} \phantom{0}6_{-5.3}^{+5.1} $ \\
9 & gpt-4-0125-preview & $1243_{-2.4}^{+2.2} $ & $-16_{-3.6}^{+3.7} $ & $\phantom{-} \phantom{0}53_{-7.4}^{+7.2} $ & $\phantom{-} \phantom{0}2_{-5.0}^{+5.1} $ & $\phantom{-} \phantom{0}3_{-6.2}^{+6.0} $ \\
10 & yi-large-preview & $1233_{-2.8}^{+2.8} $ & $-19_{-4.4}^{+4.7} $ & $\phantom{-} \phantom{0}84_{-8.8}^{+8.9} $ & $\phantom{-} \phantom{0}7_{-6.0}^{+6.1} $ & $\phantom{-} 11_{-7.1}^{+6.7} $ \\
11 & gemini-1.5-flash-api-0514 & $1226_{-3.0}^{+3.0} $ & $-25_{-4.7}^{+5.0} $ & $\phantom{-} \phantom{0}66_{-9.3}^{+9.4} $ & $\phantom{-} \phantom{0}1_{-6.3}^{+6.0} $ & $\phantom{-} \phantom{0}9_{-7.3}^{+7.3} $ \\
12 & yi-large & $1215_{-4.5}^{+4.4} $ & $-16_{-8.2}^{+8.3} $ & $\phantom{-} \phantom{0}58_{-15.1}^{+15.3} $ & $\phantom{-} \phantom{0}6_{-10.2}^{+10.2} $ & $\phantom{-} 18_{-11.9}^{+11.9} $ \\
13 & gemma-2-27b-it & $1210_{-6.0}^{+5.9} $ & $-20_{-11.0}^{+10.1} $ & $\phantom{-} \phantom{0}54_{-20.1}^{+20.1} $ & $-18_{-12.5}^{+11.7} $ & $-\phantom{0}5_{-14.0}^{+14.6} $ \\
14 & bard-jan-24-gemini-pro & $1207_{-4.5}^{+4.7} $ & $-25_{-7.0}^{+7.0} $ & $\phantom{-} \phantom{0}59_{-22.5}^{+24.1} $ & $-51_{-10.6}^{+10.6} $ & $-35_{-13.3}^{+13.1} $ \\
15 & glm-4-0520 & $1206_{-5.1}^{+5.0} $ & $-15_{-8.7}^{+8.2} $ & $\phantom{-} \phantom{0}90_{-16.0}^{+17.2} $ & $\phantom{-} 10_{-10.9}^{+10.7} $ & $\phantom{-} 13_{-12.4}^{+12.7} $ \\
16 & nemotron-4-340b-instruct & $1204_{-3.9}^{+3.6} $ & $-22_{-6.4}^{+6.4} $ & $\phantom{-} \phantom{0}62_{-12.4}^{+12.3} $ & $-\phantom{0}4_{-8.2}^{+8.3} $ & $-\phantom{0}7_{-9.9}^{+11.2} $ \\
17 & llama-3-70b-instruct & $1202_{-2.1}^{+2.1} $ & $\phantom{-} 22_{-3.4}^{+3.3} $ & $-\phantom{0}32_{-6.6}^{+6.5} $ & $-\phantom{0}5_{-4.5}^{+4.5} $ & $\phantom{-} \phantom{0}0_{-5.3}^{+5.3} $ \\
18 & claude-3-sonnet-20240229 & $1198_{-2.2}^{+2.2} $ & $-23_{-3.4}^{+3.5} $ & $\phantom{-} \phantom{0}48_{-6.6}^{+6.1} $ & $\phantom{-} \phantom{0}1_{-4.7}^{+4.4} $ & $\phantom{-} 17_{-5.1}^{+5.4} $ \\
19 & reka-core-20240501 & $1194_{-2.4}^{+2.4} $ & $-20_{-4.3}^{+4.0} $ & $\phantom{-} \phantom{0}63_{-8.5}^{+8.3} $ & $-\phantom{0}6_{-5.8}^{+5.2} $ & $-\phantom{0}4_{-5.9}^{+6.2} $ \\
20 & command-r-plus & $1188_{-2.3}^{+2.2} $ & $-25_{-3.7}^{+3.6} $ & $\phantom{-} \phantom{0}63_{-7.0}^{+6.9} $ & $-20_{-4.8}^{+5.1} $ & $-21_{-5.9}^{+5.9} $ \\
21 & gpt-4-0314 & $1188_{-2.6}^{+2.5} $ & $-23_{-4.1}^{+4.2} $ & $\phantom{-} \phantom{0}54_{-8.3}^{+8.3} $ & $\phantom{-} \phantom{0}9_{-5.6}^{+5.5} $ & $\phantom{-} 10_{-6.7}^{+6.5} $ \\
22 & qwen-max-0428 & $1185_{-2.9}^{+2.7} $ & $-17_{-4.9}^{+5.1} $ & $\phantom{-} 105_{-11.4}^{+11.3} $ & $\phantom{-} \phantom{0}3_{-7.1}^{+7.1} $ & $\phantom{-} \phantom{0}7_{-8.3}^{+7.8} $ \\
23 & qwen2-72b-instruct & $1184_{-3.2}^{+3.3} $ & $-17_{-5.3}^{+5.5} $ & $\phantom{-} 106_{-10.4}^{+10.6} $ & $\phantom{-} \phantom{0}1_{-6.9}^{+7.2} $ & $-\phantom{0}1_{-8.6}^{+8.6} $ \\
24 & claude-3-haiku-20240307 & $1181_{-2.2}^{+2.2} $ & $-23_{-3.8}^{+3.6} $ & $\phantom{-} \phantom{0}33_{-7.0}^{+6.4} $ & $\phantom{-} \phantom{0}1_{-4.6}^{+4.7} $ & $\phantom{-} 10_{-5.7}^{+5.6} $ \\
25 & gemma-2-9b-it & $1180_{-6.0}^{+6.0} $ & $-24_{-10.1}^{+10.5} $ & $\phantom{-} \phantom{0}56_{-19.5}^{+19.9} $ & $-10_{-13.3}^{+12.7} $ & $-17_{-15.1}^{+14.8} $ \\
26 & deepseek-coder-v2 & $1177_{-4.9}^{+4.6} $ & $-28_{-8.1}^{+8.3} $ & $\phantom{-} \phantom{0}80_{-16.2}^{+16.2} $ & $\phantom{-} 37_{-10.8}^{+10.3} $ & $\phantom{-} 61_{-11.8}^{+11.4} $ \\
27 & glm-4-0116 & $1173_{-5.3}^{+5.1} $ & $\phantom{-} \phantom{0}2_{-9.1}^{+9.0} $ & $\phantom{-} \phantom{0}99_{-17.9}^{+18.5} $ & $\phantom{-} 14_{-11.3}^{+10.6} $ & $\phantom{-} 19_{-13.0}^{+12.7} $ \\
28 & qwen1.5-110b-chat & $1165_{-3.1}^{+3.1} $ & $-13_{-5.1}^{+4.8} $ & $\phantom{-} \phantom{0}96_{-10.1}^{+10.4} $ & $\phantom{-} \phantom{0}4_{-6.4}^{+6.3} $ & $\phantom{-} 10_{-7.9}^{+8.1} $ \\
29 & gpt-4-0613 & $1165_{-2.4}^{+2.2} $ & $-18_{-3.8}^{+3.5} $ & $\phantom{-} \phantom{0}25_{-7.8}^{+7.6} $ & $\phantom{-} \phantom{0}3_{-5.0}^{+4.8} $ & $\phantom{-} \phantom{0}3_{-6.0}^{+5.7} $ \\
30 & reka-flash-preview-20240611 & $1164_{-4.1}^{+4.3} $ & $-22_{-7.7}^{+7.7} $ & $\phantom{-} \phantom{0}52_{-13.5}^{+13.4} $ & $-14_{-8.5}^{+8.6} $ & $-\phantom{0}3_{-9.8}^{+10.1} $ \\
31 & yi-1.5-34b-chat & $1158_{-3.4}^{+3.3} $ & $\phantom{-} \phantom{0}5_{-5.8}^{+5.7} $ & $\phantom{-} 110_{-11.1}^{+11.0} $ & $\phantom{-} \phantom{0}2_{-8.0}^{+7.0} $ & $\phantom{-} \phantom{0}6_{-9.0}^{+8.7} $ \\
32 & reka-flash-21b-20240226-online & $1155_{-3.7}^{+3.6} $ & $-19_{-6.7}^{+6.1} $ & $\phantom{-} \phantom{0}46_{-10.9}^{+11.0} $ & $-12_{-8.8}^{+8.5} $ & $-\phantom{0}6_{-8.9}^{+8.4} $ \\
33 & mistral-large-2402 & $1155_{-2.4}^{+2.5} $ & $-\phantom{0}9_{-4.2}^{+4.0} $ & $\phantom{-} \phantom{0}18_{-7.8}^{+7.9} $ & $\phantom{-} 10_{-5.3}^{+5.5} $ & $\phantom{-} 14_{-6.2}^{+6.2} $ \\
34 & llama-3-8b-instruct & $1154_{-2.3}^{+2.2} $ & $\phantom{-} 11_{-3.7}^{+3.6} $ & $-\phantom{0}15_{-6.8}^{+6.7} $ & $-16_{-4.6}^{+4.6} $ & $-\phantom{0}6_{-5.5}^{+5.8} $ \\
35 & qwen1.5-72b-chat & $1151_{-2.6}^{+2.4} $ & $-16_{-4.3}^{+4.3} $ & $\phantom{-} \phantom{0}94_{-9.1}^{+9.0} $ & $-\phantom{0}4_{-5.9}^{+5.8} $ & $\phantom{-} 11_{-7.4}^{+6.8} $ \\
36 & claude-1 & $1150_{-3.8}^{+3.7} $ & $-21_{-5.8}^{+5.8} $ & $\phantom{-} \phantom{0}49_{-13.7}^{+14.4} $ & $-25_{-8.5}^{+7.9} $ & $-12_{-10.4}^{+10.5} $ \\
37 & command-r & $1149_{-2.5}^{+2.5} $ & $-26_{-4.3}^{+4.2} $ & $\phantom{-} \phantom{0}66_{-7.5}^{+7.2} $ & $-30_{-5.6}^{+5.5} $ & $-23_{-6.0}^{+6.4} $ \\
38 & reka-flash-21b-20240226 & $1147_{-3.3}^{+3.1} $ & $-20_{-5.1}^{+5.1} $ & $\phantom{-} \phantom{0}46_{-9.9}^{+10.2} $ & $-13_{-6.3}^{+7.1} $ & $-\phantom{0}4_{-8.1}^{+7.3} $ \\
39 & mistral-medium & $1146_{-2.8}^{+2.9} $ & $-\phantom{0}9_{-4.9}^{+4.7} $ & $\phantom{-} \phantom{0}20_{-10.4}^{+9.9} $ & $-\phantom{0}1_{-6.3}^{+6.0} $ & $\phantom{-} \phantom{0}8_{-7.2}^{+7.6} $ \\
40 & mixtral-8x22b-instruct-v0.1 & $1146_{-2.7}^{+2.7} $ & $-10_{-4.2}^{+4.4} $ & $\phantom{-} \phantom{0}40_{-9.0}^{+8.5} $ & $\phantom{-} \phantom{0}3_{-6.2}^{+5.9} $ & $\phantom{-} \phantom{0}9_{-6.9}^{+6.4} $ \\
41 & gemini-pro-dev-api & $1136_{-3.7}^{+3.6} $ & $-26_{-5.8}^{+6.3} $ & $\phantom{-} \phantom{0}51_{-12.6}^{+12.6} $ & $-27_{-8.9}^{+8.8} $ & $-31_{-10.0}^{+10.0} $ \\
42 & claude-2.0 & $1133_{-4.5}^{+4.7} $ & $-19_{-6.8}^{+6.9} $ & $\phantom{-} \phantom{0}58_{-21.0}^{+21.8} $ & $-\phantom{0}5_{-10.1}^{+10.6} $ & $\phantom{-} \phantom{0}4_{-13.1}^{+13.5} $ \\
43 & qwen1.5-32b-chat & $1132_{-3.4}^{+3.3} $ & $-21_{-5.2}^{+5.5} $ & $\phantom{-} 104_{-9.8}^{+9.6} $ & $\phantom{-} \phantom{0}4_{-7.4}^{+7.5} $ & $\phantom{-} 16_{-8.7}^{+8.6} $ \\
44 & zephyr-orpo-141b-A35b-v0.1 & $1128_{-6.0}^{+6.3} $ & $-\phantom{0}9_{-10.6}^{+11.4} $ & $\phantom{-} \phantom{0}22_{-18.1}^{+18.8} $ & $-11_{-15.1}^{+14.5} $ & $-\phantom{0}5_{-17.2}^{+16.6} $ \\
45 & mistral-next & $1127_{-4.5}^{+4.5} $ & $-16_{-6.9}^{+6.5} $ & $\phantom{-} \phantom{0}12_{-17.8}^{+17.2} $ & $\phantom{-} \phantom{0}3_{-9.1}^{+9.8} $ & $\phantom{-} \phantom{0}7_{-11.8}^{+12.1} $ \\
46 & phi-3-medium-4k-instruct & $1125_{-4.1}^{+4.1} $ & $-\phantom{0}7_{-6.6}^{+7.0} $ & $\phantom{-} \phantom{0}36_{-11.9}^{+12.2} $ & $\phantom{-} \phantom{0}9_{-9.0}^{+8.8} $ & $\phantom{-} 10_{-9.2}^{+9.9} $ \\
47 & gpt-3.5-turbo-0613 & $1120_{-2.9}^{+2.9} $ & $-21_{-4.5}^{+4.5} $ & $\phantom{-} \phantom{0}40_{-13.3}^{+13.5} $ & $\phantom{-} \phantom{0}4_{-6.6}^{+6.8} $ & $\phantom{-} 16_{-8.3}^{+8.6} $ \\
48 & qwen1.5-14b-chat & $1119_{-3.7}^{+3.4} $ & $-19_{-6.1}^{+6.0} $ & $\phantom{-} \phantom{0}89_{-9.7}^{+9.8} $ & $\phantom{-} \phantom{0}1_{-7.4}^{+7.4} $ & $\phantom{-} \phantom{0}9_{-9.1}^{+8.8} $ \\
49 & starling-lm-7b-beta & $1119_{-4.0}^{+3.7} $ & $-12_{-6.3}^{+6.4} $ & $\phantom{-} \phantom{0}66_{-10.3}^{+10.5} $ & $-\phantom{0}1_{-8.1}^{+7.8} $ & $\phantom{-} 13_{-9.2}^{+9.1} $ \\
50 & claude-2.1 & $1118_{-2.9}^{+3.0} $ & $-22_{-4.5}^{+4.6} $ & $\phantom{-} \phantom{0}32_{-11.8}^{+10.9} $ & $\phantom{-} \phantom{0}2_{-6.5}^{+6.4} $ & $\phantom{-} 15_{-8.7}^{+8.0} $ \\
51 & yi-34b-chat & $1116_{-3.8}^{+3.9} $ & $-\phantom{0}9_{-6.3}^{+6.5} $ & $\phantom{-} 116_{-14.3}^{+14.7} $ & $-12_{-9.2}^{+8.8} $ & $-\phantom{0}9_{-10.7}^{+10.5} $ \\
52 & gemini-pro & $1115_{-6.1}^{+6.2} $ & $-16_{-9.4}^{+9.6} $ & $\phantom{-} \phantom{0}52_{-30.2}^{+29.4} $ & $-30_{-13.5}^{+14.4} $ & $-19_{-19.3}^{+17.3} $ \\
53 & mixtral-8x7b-instruct-v0.1 & $1114_{0.0}^{+0.0} $ & $\phantom{-} \phantom{0}0_{0.0}^{+0.0} $ & $\phantom{-} \phantom{00}0_{0.0}^{+0.0} $ & $\phantom{-} \phantom{0}0_{0.0}^{+0.0} $ & $\phantom{-} \phantom{0}0_{0.0}^{+0.0} $ \\
54 & gpt-3.5-turbo-0125 & $1113_{-2.2}^{+2.4} $ & $-24_{-4.0}^{+4.0} $ & $\phantom{-} \phantom{0}29_{-7.7}^{+7.6} $ & $\phantom{-} \phantom{0}1_{-5.1}^{+5.4} $ & $\phantom{-} 12_{-6.5}^{+6.1} $ \\
55 & claude-instant-1 & $1112_{-3.9}^{+3.9} $ & $-16_{-5.8}^{+6.1} $ & $\phantom{-} \phantom{0}38_{-17.2}^{+17.5} $ & $-\phantom{0}4_{-8.7}^{+8.7} $ & $-\phantom{0}2_{-10.8}^{+11.3} $ \\
56 & wizardlm-70b & $1110_{-5.6}^{+5.4} $ & $-11_{-8.7}^{+8.2} $ & $\phantom{-} \phantom{0}10_{-27.7}^{+27.5} $ & $-31_{-12.2}^{+12.9} $ & $-38_{-15.3}^{+15.7} $ \\
57 & gpt-3.5-turbo-0314 & $1110_{-7.2}^{+7.3} $ & $-26_{-11.8}^{+11.2} $ & $\phantom{-} \phantom{0}95_{-30.5}^{+30.4} $ & $\phantom{-} \phantom{0}9_{-20.6}^{+18.4} $ & $\phantom{-} \phantom{0}8_{-24.1}^{+24.3} $ \\
58 & dbrx-instruct-preview & $1106_{-3.1}^{+2.8} $ & $-\phantom{0}2_{-4.7}^{+4.7} $ & $\phantom{-} \phantom{0}30_{-8.5}^{+8.2} $ & $\phantom{-} \phantom{0}2_{-6.4}^{+6.2} $ & $\phantom{-} 15_{-7.4}^{+7.4} $ \\
59 & phi-3-small-8k-instruct & $1104_{-3.8}^{+3.9} $ & $\phantom{-} \phantom{0}2_{-6.7}^{+6.9} $ & $\phantom{-} \phantom{0}21_{-11.6}^{+11.7} $ & $\phantom{-} \phantom{0}3_{-8.1}^{+8.6} $ & $\phantom{-} \phantom{0}3_{-10.0}^{+9.4} $ \\
60 & tulu-2-dpo-70b & $1103_{-6.1}^{+6.2} $ & $-11_{-9.3}^{+8.5} $ & $-\phantom{0}33_{-31.3}^{+29.0} $ & $-\phantom{0}5_{-13.9}^{+14.3} $ & $-\phantom{0}8_{-18.0}^{+17.0} $ \\
61 & snowflake-arctic-instruct & $1099_{-2.8}^{+2.9} $ & $-20_{-4.6}^{+4.7} $ & $\phantom{-} \phantom{0}53_{-9.6}^{+9.2} $ & $-23_{-6.1}^{+6.2} $ & $-19_{-8.1}^{+7.3} $ \\
62 & openchat-3.5-0106 & $1099_{-4.1}^{+4.2} $ & $-15_{-6.7}^{+6.3} $ & $\phantom{-} \phantom{0}48_{-13.0}^{+14.0} $ & $-13_{-8.5}^{+8.7} $ & $\phantom{-} \phantom{0}6_{-11.4}^{+11.5} $ \\
63 & llama-2-70b-chat & $1097_{-2.8}^{+2.7} $ & $\phantom{-} \phantom{0}1_{-4.7}^{+4.4} $ & $-\phantom{0}39_{-9.4}^{+9.5} $ & $-25_{-5.8}^{+6.0} $ & $-22_{-7.7}^{+7.7} $ \\
64 & vicuna-33b & $1095_{-3.4}^{+3.6} $ & $-\phantom{0}7_{-5.5}^{+5.2} $ & $\phantom{-} \phantom{00}9_{-12.9}^{+13.1} $ & $-27_{-8.2}^{+7.8} $ & $-28_{-9.7}^{+9.8} $ \\
65 & starling-lm-7b-alpha & $1093_{-4.7}^{+4.9} $ & $-\phantom{0}7_{-7.8}^{+7.4} $ & $\phantom{-} \phantom{0}20_{-17.1}^{+17.5} $ & $-17_{-10.6}^{+10.8} $ & $-10_{-12.9}^{+12.6} $ \\
66 & gemma-1.1-7b-it & $1090_{-3.3}^{+3.3} $ & $-\phantom{0}8_{-5.4}^{+5.4} $ & $\phantom{-} \phantom{0}39_{-9.8}^{+9.9} $ & $-13_{-7.1}^{+7.2} $ & $-\phantom{0}3_{-8.0}^{+7.8} $ \\
67 & nous-hermes-2-mixtral-8x7b-dpo & $1087_{-6.8}^{+7.6} $ & $-\phantom{0}9_{-11.4}^{+11.4} $ & $-\phantom{00}9_{-48.2}^{+47.6} $ & $-35_{-15.5}^{+15.8} $ & $-\phantom{0}4_{-19.9}^{+18.7} $ \\
68 & llama2-70b-steerlm-chat & $1083_{-8.5}^{+7.9} $ & $-14_{-12.6}^{+12.9} $ & $\phantom{-} \phantom{0}14_{-35.5}^{+37.5} $ & $-35_{-20.0}^{+19.9} $ & $-59_{-23.0}^{+23.2} $ \\
69 & openchat-3.5 & $1080_{-5.3}^{+5.4} $ & $-14_{-8.7}^{+7.8} $ & $\phantom{-} \phantom{0}53_{-25.7}^{+26.8} $ & $-14_{-12.7}^{+12.1} $ & $-24_{-16.3}^{+15.4} $ \\
70 & deepseek-llm-67b-chat & $1080_{-7.0}^{+7.0} $ & $-15_{-10.8}^{+10.3} $ & $\phantom{-} 103_{-33.8}^{+34.8} $ & $-14_{-15.5}^{+15.3} $ & $\phantom{-} \phantom{0}2_{-19.7}^{+20.1} $ \\
71 & openhermes-2.5-mistral-7b & $1080_{-6.3}^{+6.4} $ & $-\phantom{0}6_{-9.9}^{+9.4} $ & $\phantom{-} \phantom{00}8_{-33.3}^{+34.6} $ & $-10_{-14.8}^{+15.1} $ & $-18_{-19.9}^{+20.2} $ \\
72 & qwen1.5-7b-chat & $1079_{-6.3}^{+6.3} $ & $-22_{-10.1}^{+10.1} $ & $\phantom{-} 122_{-23.3}^{+22.7} $ & $-10_{-13.7}^{+12.9} $ & $\phantom{-} 13_{-17.7}^{+18.0} $ \\
73 & pplx-70b-online & $1077_{-6.1}^{+5.9} $ & $-12_{-9.4}^{+9.2} $ & $\phantom{-} \phantom{0}54_{-30.5}^{+29.6} $ & $-49_{-13.7}^{+13.4} $ & $-49_{-15.5}^{+16.0} $ \\
74 & mistral-7b-instruct-v0.2 & $1075_{-3.5}^{+3.7} $ & $\phantom{-} \phantom{0}7_{-5.7}^{+5.7} $ & $\phantom{-} \phantom{00}8_{-10.7}^{+11.2} $ & $-\phantom{0}6_{-7.4}^{+7.9} $ & $\phantom{-} \phantom{0}0_{-9.6}^{+9.2} $ \\
75 & gpt-3.5-turbo-1106 & $1073_{-3.8}^{+3.9} $ & $-18_{-5.9}^{+6.2} $ & $\phantom{-} \phantom{0}10_{-19.0}^{+17.8} $ & $\phantom{-} 20_{-9.3}^{+9.0} $ & $\phantom{-} 25_{-10.3}^{+10.8} $ \\
76 & phi-3-mini-4k-instruct & $1072_{-3.7}^{+3.7} $ & $\phantom{-} \phantom{0}3_{-6.1}^{+6.1} $ & $\phantom{-} \phantom{0}12_{-11.5}^{+12.0} $ & $\phantom{-} \phantom{0}8_{-7.1}^{+7.1} $ & $\phantom{-} 16_{-8.7}^{+8.4} $ \\
77 & llama-2-13b-chat & $1068_{-3.8}^{+4.0} $ & $-\phantom{0}6_{-6.3}^{+5.8} $ & $-\phantom{0}17_{-15.4}^{+15.5} $ & $-19_{-8.7}^{+9.0} $ & $-16_{-10.8}^{+10.5} $ \\
78 & solar-10.7b-instruct-v1.0 & $1067_{-7.2}^{+7.2} $ & $-\phantom{0}5_{-11.1}^{+10.4} $ & $\phantom{-} \phantom{00}0_{-35.9}^{+37.2} $ & $-\phantom{0}9_{-16.7}^{+17.0} $ & $-16_{-21.1}^{+19.8} $ \\
79 & dolphin-2.2.1-mistral-7b & $1066_{-11.3}^{+11.4} $ & $-\phantom{0}5_{-17.2}^{+16.6} $ & $\phantom{-} \phantom{0}44_{-54.6}^{+56.3} $ & $-15_{-26.6}^{+27.3} $ & $-40_{-34.6}^{+34.2} $ \\
80 & wizardlm-13b & $1063_{-5.6}^{+6.0} $ & $-12_{-8.7}^{+8.9} $ & $\phantom{-} \phantom{0}28_{-26.0}^{+26.1} $ & $-49_{-14.3}^{+15.0} $ & $-37_{-17.3}^{+18.8} $ \\
81 & zephyr-7b-beta & $1057_{-5.0}^{+5.2} $ & $-\phantom{0}2_{-7.1}^{+7.6} $ & $-\phantom{0}31_{-24.3}^{+24.9} $ & $-29_{-11.5}^{+11.9} $ & $-24_{-13.8}^{+14.2} $ \\
82 & phi-3-mini-128k-instruct & $1054_{-3.4}^{+3.6} $ & $-15_{-5.4}^{+5.7} $ & $\phantom{-} \phantom{0}47_{-11.4}^{+11.1} $ & $-15_{-7.4}^{+7.6} $ & $-23_{-9.2}^{+8.7} $ \\
83 & vicuna-13b & $1050_{-3.9}^{+4.2} $ & $-19_{-6.2}^{+6.2} $ & $\phantom{-} \phantom{0}63_{-16.3}^{+15.5} $ & $-23_{-8.9}^{+9.2} $ & $-15_{-11.8}^{+11.6} $ \\
84 & mpt-30b-chat & $1050_{-9.4}^{+9.4} $ & $-\phantom{0}5_{-15.1}^{+14.0} $ & $-\phantom{00}3_{-48.3}^{+48.4} $ & $-\phantom{0}2_{-25.0}^{+25.1} $ & $-21_{-30.3}^{+28.5} $ \\
85 & codellama-34b-instruct & $1049_{-5.7}^{+6.0} $ & $-13_{-8.5}^{+8.5} $ & $-\phantom{0}17_{-29.4}^{+31.5} $ & $-19_{-13.2}^{+14.5} $ & $-\phantom{0}8_{-17.2}^{+16.9} $ \\
86 & zephyr-7b-alpha & $1048_{-10.9}^{+10.7} $ & $-\phantom{0}6_{-16.4}^{+16.1} $ & $\phantom{-} \phantom{00}1_{-68.4}^{+68.5} $ & $-27_{-28.5}^{+28.2} $ & $-14_{-32.8}^{+31.9} $ \\
87 & codellama-70b-instruct & $1047_{-13.5}^{+14.6} $ & $-\phantom{0}3_{-22.0}^{+22.8} $ & $\phantom{-} \phantom{0}62_{-37.2}^{+39.8} $ & $\phantom{-} \phantom{0}3_{-28.6}^{+29.9} $ & $\phantom{-} \phantom{0}2_{-36.9}^{+34.8} $ \\
88 & pplx-7b-online & $1045_{-6.6}^{+6.4} $ & $-\phantom{0}6_{-9.6}^{+10.2} $ & $\phantom{-} \phantom{0}47_{-31.8}^{+33.3} $ & $-28_{-14.4}^{+14.7} $ & $-30_{-17.1}^{+17.8} $ \\
89 & gemma-7b-it & $1043_{-5.2}^{+5.3} $ & $-\phantom{0}8_{-8.0}^{+8.3} $ & $\phantom{-} \phantom{0}64_{-15.6}^{+16.0} $ & $\phantom{-} \phantom{0}4_{-11.4}^{+11.8} $ & $\phantom{-} \phantom{0}7_{-12.8}^{+13.7} $ \\
90 & llama-2-7b-chat & $1043_{-4.1}^{+4.1} $ & $\phantom{-} \phantom{0}1_{-6.5}^{+6.3} $ & $-\phantom{0}11_{-15.6}^{+15.9} $ & $-32_{-9.2}^{+9.8} $ & $-38_{-11.7}^{+11.3} $ \\
91 & qwen-14b-chat & $1041_{-6.4}^{+6.8} $ & $-21_{-10.6}^{+10.3} $ & $\phantom{-} \phantom{0}94_{-36.5}^{+34.7} $ & $-16_{-16.8}^{+16.3} $ & $\phantom{-} 16_{-20.5}^{+19.6} $ \\
92 & falcon-180b-chat & $1039_{-13.3}^{+14.1} $ & $-12_{-21.2}^{+20.6} $ & $-\phantom{00}6_{-103.1}^{+79.9} $ & $-38_{-31.7}^{+32.2} $ & $-22_{-43.5}^{+42.0} $ \\
93 & guanaco-33b & $1037_{-9.4}^{+9.1} $ & $-\phantom{0}7_{-13.7}^{+13.0} $ & $-\phantom{00}8_{-37.8}^{+37.5} $ & $-35_{-23.0}^{+23.6} $ & $-69_{-27.9}^{+28.3} $ \\
94 & gemma-1.1-2b-it & $1034_{-4.7}^{+4.5} $ & $-15_{-8.0}^{+8.0} $ & $\phantom{-} \phantom{0}54_{-13.8}^{+13.9} $ & $-15_{-10.6}^{+10.2} $ & $\phantom{-} \phantom{0}8_{-11.1}^{+11.5} $ \\
95 & stripedhyena-nous-7b & $1024_{-6.8}^{+6.8} $ & $-\phantom{0}8_{-9.9}^{+9.9} $ & $\phantom{-} \phantom{0}11_{-36.7}^{+36.3} $ & $-26_{-14.3}^{+14.5} $ & $-21_{-17.9}^{+18.8} $ \\
96 & olmo-7b-instruct & $1021_{-6.0}^{+6.1} $ & $\phantom{-} \phantom{0}0_{-9.7}^{+9.9} $ & $\phantom{-} \phantom{0}62_{-18.5}^{+18.4} $ & $-26_{-13.2}^{+12.5} $ & $-\phantom{0}5_{-16.3}^{+17.3} $ \\
97 & mistral-7b-instruct & $1016_{-5.3}^{+5.6} $ & $-\phantom{0}4_{-8.4}^{+8.1} $ & $-\phantom{00}8_{-25.7}^{+26.1} $ & $-10_{-12.6}^{+11.6} $ & $-\phantom{0}5_{-14.5}^{+15.3} $ \\
98 & palm-2 & $1012_{-5.9}^{+5.7} $ & $-\phantom{0}1_{-8.2}^{+8.7} $ & $-\phantom{0}69_{-32.4}^{+30.6} $ & $-12_{-13.9}^{+14.4} $ & $-22_{-16.6}^{+16.5} $ \\
99 & vicuna-7b & $1012_{-6.2}^{+6.2} $ & $-20_{-9.2}^{+9.4} $ & $\phantom{-} \phantom{0}30_{-27.8}^{+25.6} $ & $-20_{-15.3}^{+15.6} $ & $-27_{-17.3}^{+17.8} $ \\
100 & qwen1.5-4b-chat & $1003_{-5.3}^{+5.5} $ & $-30_{-9.0}^{+9.2} $ & $\phantom{-} \phantom{0}92_{-16.5}^{+15.8} $ & $-21_{-11.5}^{+11.8} $ & $-11_{-14.3}^{+15.6} $ \\
101 & gemma-2b-it & $1000_{-6.8}^{+6.7} $ & $-11_{-11.2}^{+10.7} $ & $\phantom{-} \phantom{0}67_{-21.3}^{+20.8} $ & $-12_{-14.9}^{+14.8} $ & $\phantom{-} \phantom{0}0_{-18.4}^{+18.2} $ \\
102 & koala-13b & $\phantom{0}971_{-6.6}^{+6.5} $ & $-\phantom{0}6_{-9.5}^{+9.9} $ & $-\phantom{0}34_{-25.7}^{+25.9} $ & $-43_{-16.4}^{+16.8} $ & $-30_{-18.9}^{+18.7} $ \\
103 & chatglm3-6b & $\phantom{0}962_{-7.7}^{+7.9} $ & $-11_{-11.2}^{+11.6} $ & $\phantom{-} 159_{-35.2}^{+33.1} $ & $-\phantom{0}7_{-17.0}^{+17.2} $ & $-\phantom{0}9_{-22.3}^{+22.6} $ \\
104 & gpt4all-13b-snoozy & $\phantom{0}941_{-12.2}^{+11.6} $ & $-\phantom{0}4_{-17.0}^{+18.2} $ & $-\phantom{00}6_{-44.9}^{+48.8} $ & $-\phantom{0}6_{-28.5}^{+28.2} $ & $-28_{-37.5}^{+35.3} $ \\
105 & chatglm2-6b & $\phantom{0}936_{-9.8}^{+9.9} $ & $-\phantom{0}7_{-15.0}^{+14.9} $ & $\phantom{-} 120_{-46.3}^{+47.3} $ & $-19_{-23.1}^{+25.1} $ & $-43_{-30.5}^{+29.9} $ \\
106 & mpt-7b-chat & $\phantom{0}935_{-8.2}^{+8.0} $ & $-15_{-11.9}^{+11.4} $ & $\phantom{-} \phantom{0}73_{-32.0}^{+34.0} $ & $-36_{-18.5}^{+20.6} $ & $-28_{-24.7}^{+26.1} $ \\
107 & RWKV-4-Raven-14B & $\phantom{0}929_{-7.7}^{+8.0} $ & $-19_{-11.5}^{+11.4} $ & $\phantom{-} \phantom{0}29_{-30.9}^{+31.6} $ & $-36_{-18.2}^{+18.2} $ & $-30_{-22.2}^{+23.7} $ \\
108 & alpaca-13b & $\phantom{0}911_{-7.2}^{+7.0} $ & $-13_{-10.1}^{+10.3} $ & $-\phantom{0}65_{-30.9}^{+30.4} $ & $-88_{-17.7}^{+18.0} $ & $-117_{-24.0}^{+22.7} $ \\
109 & oasst-pythia-12b & $\phantom{0}902_{-6.8}^{+7.0} $ & $-\phantom{0}9_{-10.9}^{+11.5} $ & $-\phantom{0}41_{-26.6}^{+26.8} $ & $-18_{-16.4}^{+18.1} $ & $-26_{-21.6}^{+22.4} $ \\
110 & chatglm-6b & $\phantom{0}889_{-7.5}^{+7.9} $ & $-25_{-11.6}^{+10.8} $ & $\phantom{-} 252_{-30.3}^{+30.0} $ & $\phantom{-} \phantom{0}9_{-19.4}^{+19.0} $ & $\phantom{-} \phantom{0}1_{-23.3}^{+22.5} $ \\
111 & fastchat-t5-3b & $\phantom{0}879_{-7.9}^{+7.9} $ & $-\phantom{0}1_{-12.0}^{+11.7} $ & $\phantom{-} \phantom{0}22_{-250.3}^{+172.3} $ & $-66_{-19.0}^{+18.6} $ & $-117_{-25.2}^{+25.8} $ \\
112 & stablelm-tuned-alpha-7b & $\phantom{0}851_{-9.2}^{+9.7} $ & $-13_{-14.1}^{+13.3} $ & $\phantom{-} \phantom{0}52_{-31.8}^{+35.9} $ & $-17_{-22.6}^{+23.8} $ & $\phantom{-} 10_{-26.3}^{+27.3} $ \\
113 & dolly-v2-12b & $\phantom{0}828_{-9.3}^{+9.2} $ & $-20_{-13.5}^{+14.0} $ & $\phantom{-} \phantom{0}53_{-35.2}^{+35.2} $ & $-27_{-22.3}^{+23.2} $ & $-78_{-28.5}^{+27.3} $ \\
114 & llama-13b & $\phantom{0}806_{-10.6}^{+10.2} $ & $-23_{-16.7}^{+16.6} $ & $\phantom{-} \phantom{0}47_{-36.2}^{+35.7} $ & $-79_{-27.8}^{+28.7} $ & $-134_{-35.6}^{+35.4} $ \\

\end{longtable}
    }

\end{footnotesize}
