# Supplementary material for: CreDes: Causal Reasoning Enhancement and Dual-End Searching for Solving Long-Range Reasoning Problems using LLMs
Source: arXiv:2410.01696 source file (2024-10-02)
Supplement: Supplementary file 2 [file appendix-alternatives.tex]

\section{Alternative Rating Systems}\label{app:alternatives}

This section explores several alternatives to the exponential rating system that solves the MLE of the logistic loss function, as discussed in \cref{sec:background}. Specifically, we evaluate two extensions to the BT-model and one alternative inspired by the accuracy metric commonly used in benchmarks. We then compare these alternatives with the exponential rating system in terms of their predictive performance and demonstrate that their added complexity does not result in better predictions.

All models discussed here are compatible with \tool and can be used as substitutes for the MLE-based BT-model used in \cref{sec:experiments}.

\paragraph{Rao-Kupper Model} \citet{raokupper} extend the BT-model to explicitly account for the probability of a draw by introducing a parameter $\theta \in \mathbb{R}, \theta \geq 1$:

\begin{align*}
    P(i \succ j | \gamma_i, \gamma_j) &= \frac{\gamma_i}{\gamma_i + \theta \gamma_j} \\
    P(j \succ i | \gamma_i, \gamma_j) &= \frac{\gamma_j}{\gamma_j + \theta \gamma_i} \\
    P(i \simeq j | \gamma_i, \gamma_j) &= \frac{\gamma_i \gamma_j (\theta^2 - 1)}{(\gamma_j + \theta \gamma_i)(\gamma_i + \theta \gamma_j)}\\
\end{align*}

It can be shown that this model follows from the hypothesis that a judge cannot tell the difference between two answers if the quality of the answers is close to each other. 

\paragraph{Davidson-Model} \citet{davidson1970on} propose a similar modification to include draws, using a parameter $\theta \in \mathbb{R}, \theta \geq 0$:

\begin{align*}
    P(i \succ j | \gamma_i, \gamma_j) &= \frac{\gamma_i}{\gamma_i + \gamma_j + \theta \sqrt{\gamma_i \gamma_j}} \\
    P(j \succ i | \gamma_i, \gamma_j) &= \frac{\gamma_j}{\gamma_i + \gamma_j + \theta \sqrt{\gamma_i \gamma_j}}\\
    P(i \simeq j | \gamma_i, \gamma_j) &= \frac{\theta \sqrt{\gamma_i \gamma_j}}{\gamma_i + \gamma_j + \theta \sqrt{\gamma_i \gamma_j}} \\
\end{align*}

\paragraph{Accuracy-Based Model} Both extensions to the BT-model presented above still model ratings using an exponential function. However, for LLMs, it could be beneficial to use ratings directly comparable to standard benchmark accuracies. Benchmarks can be viewed as a series of games where, for a given question $Q$, model $m_1$ defeats model $m_2$ if $m_1$ answers correctly and $m_2$ does not. A draw occurs if both answer correctly or incorrectly and otherwise $m_2$ wins. 

Let $\text{Acc}_D$ denote the accuracy function on benchmark $D$. If we model draws as $0.5$ points for each model, the win rates can be expressed as:
\begin{align*}
    P(i \succ j | m_i, m_j) &= \frac{1}{2} \Big(1 + \text{Acc}_D(m_1) - \text{Acc}_D(m_2)\Big)\\
    P(j \succ i | m_i, m_j) &= \frac{1}{2} \Big(1 + \text{Acc}_D(m_2) - \text{Acc}_D(m_1)\Big).\\
\end{align*}
To adapt the BT-model to this accuracy-based approach, we modify it as follows:
\begin{align*}
    P(i \succ j | R_i, R_j) &= \min\left(1, \max\left(0, \frac{1}{2} (1 + R_i - R_j)\right)\right)\\
    P(j \succ i | R_i, R_j) &= \min\left(1, \max\left(0, \frac{1}{2} (1 + R_j - R_i)\right)\right),\\
\end{align*}
where the $\min$ and $\max$ functions ensure probabilities remain within the $[0,1]$ range. Fitting this model on a standard accuracy-based benchmark by minimizing the logistic loss from \cref{eq:logistic-loss} would exactly recover the benchmark accuracies (up to a constant shift). In contrast, the exponential used in the standard BT-model would ensure the benchmark would not exactly recover the accuracies. Thus, the ratings obtained with this model would be more directly comparable with accuracies from standard benchmarks.

\paragraph{Comparison} Comparing these models is challenging because the Rao-Kupper and Davidson models include an additional draw prediction. For predictive purposes, we are only interested in the logistic loss $\mathcal{L}$ from \cref{eq:logistic-loss} to determine whether the additional complexity of the Rao-Kupper and Davidson models reduces the value of $\mathcal{L}$ on an unknown test set. Using data from the Chatbot Arena \citep{chatbot_arena}, we compute $\mathcal{L}$ for various training set sizes. For the Davidson and Rao-Kupper models, we add $0.5P(i \simeq j | \gamma_i, \gamma_j)$ to both $P(i \succ j | \gamma_i, \gamma_j)$ and $P(j \succ i | \gamma_i, \gamma_j)$.

Results are shown in \cref{fig:alternatives}. The Roa-Kupper model performs the worst, while the accuracy-based model is only slightly worse than the remaining two. Finally, both the Davidson and BT-model perform almost identically. Due to the extra complexity of the Davidson model and the more frequent use of the BT-model for LLMs, we decided to use the BT-model as a default for \tool.

\begin{figure}[t]
    \centering
    \includegraphics[width=0.6\textwidth]{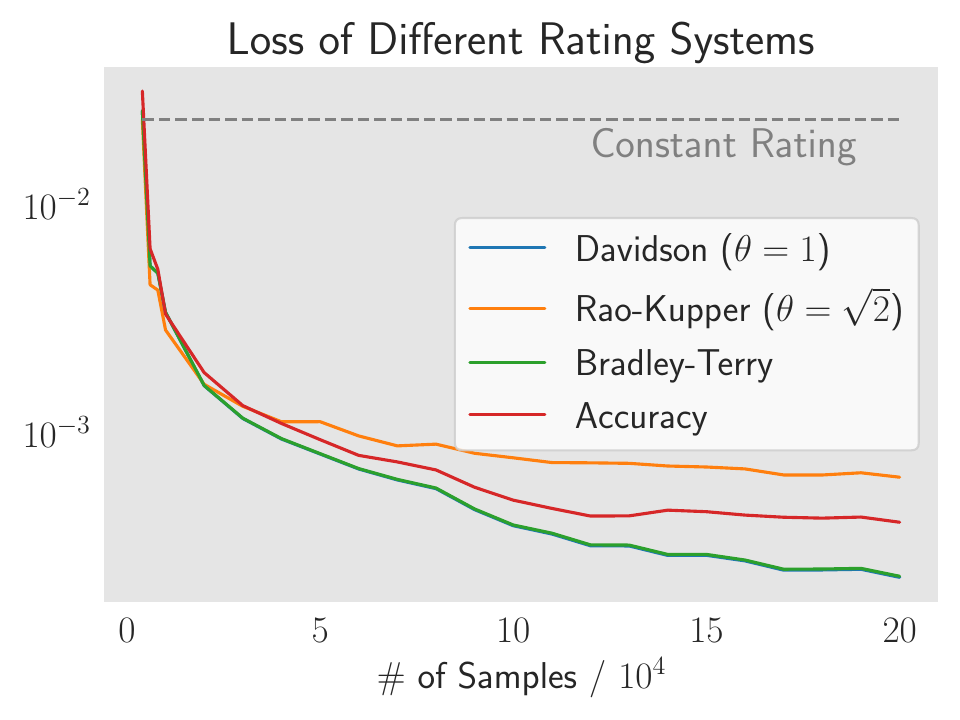}
    \caption{Logistic loss for all four alternatives on the Chatbot Arena dataset for various sizes of the training set.}
    \label{fig:alternatives}
\end{figure}
