# Supplementary material for: CreDes: Causal Reasoning Enhancement and Dual-End Searching for Solving Long-Range Reasoning Problems using LLMs
Source: arXiv:2410.01696 source file (2024-10-02)
Supplement: Supplementary file 3 [file appendix-attribution.tex]

\section{Attribution}\label{app:attribution}

We provide attribution for the icons used in \cref{fig:overview} here. The code icon was obtained from \href{https://www.flaticon.com/free-icon/code\_3573187?term=code&page=1&position=1&origin=search&related\_id=3573187}{flaticon.com} and created by Royyan Wijaya. The Chinese icon was obtained from \href{https://www.flaticon.com/free-icon/dragon\_3552304?term=chinese&page=1&position=29&origin=search&related\_id=3552304}{flaticon.com} and created by Freepik. The bot icon was obtained from \href{https://www.flaticon.com/free-icon/bot\_15107346?term=robot&page=1&position=31&origin=search&related\_id=15107346}{flaticon.com} and created by Nuriali. The math icon was obtained from \href{https://www.flaticon.com/free-icon/calculator\_15798843?term=math&page=1&position=7&origin=search&related\_id=15798843}{flaticon.com} and created by widphic. The length icon was obtained from \href{https://www.freepik.com/icon/measuring-tool\_7416244#fromView=search&page=1&position=20&uuid=37894940-a4bb-46c5-8113-bd195e33359d}{freepik.com} and created by Surang Lineal. Finally, the readability icon was obtained from \href{https://www.freepik.com/icon/guidelines\_8463884#fromView=search&page=1&position=0&uuid=4d763cb1-7646-41bd-90c7-7c422b5ab42e}{freepik.com} and created by Generic Detailed Outline.
