# Supplementary material for: CreDes: Causal Reasoning Enhancement and Dual-End Searching for Solving Long-Range Reasoning Problems using LLMs
Source: arXiv:2410.01696 source file (2024-10-02)
Supplement: Supplementary file 4 [file appendix-details.tex]

\section{Experimental Details}\label{app:details}
In this section, we provide detailed descriptions of the biases and tasks used in our experiments. In \cref{tab:biases:description} we describe the biases used in \cref{sec:experiments:bias} in more detail. In \cref{tab:categories:description} we describe the tasks used in \cref{sec:experiments} in more detail.

We also briefly explain how we adjust the win rates of traditional benchmarks to improve sample efficiency of human evaluation, as discussed in \cref{sec:experiments:convergence}. As detailed in the accuracy-based model in \cref{app:alternatives}, the win rate of $m_1$ over $m_2$ in a traditional benchmark can be written as 
\begin{align*}
    P(i \succ j | m_i, m_j) &= \frac{1}{2} \Big(1 + \text{Acc}_D(m_1) - \text{Acc}_D(m_2)\Big)\\
    P(j \succ i | m_i, m_j) &= \frac{1}{2} \Big(1 + \text{Acc}_D(m_2) - \text{Acc}_D(m_1)\Big).\\
\end{align*}
where $\text{Acc}_D$ is the accuracy function. 

Benchmarks often exhibit significant variation in accuracy differences between models. For instance, in some benchmarks, models may have closely aligned accuracies, while in others, the differences may be substantial. This variation affects the win rate estimates between models. To address this, we introduce a parameter $\mathcal{W}$, which allows us to adjust the scale of win rates. The adjusted win rates are modeled as:
\begin{align*}
    P(i \succ j | m_i, m_j) &= \min\left(1, \frac{\mathcal{W}}{2} \Big(1 + \text{Acc}_D(m_1) - \text{Acc}_D(m_2)\Big)\right)\\
    P(j \succ i | m_i, m_j) &= 1 - P(i \succ j | m_i, m_j).\\
\end{align*}
This adjustment ensures that we can control the scale of win rates, mitigating the issue of varying accuracy differences. We optimize the hyperparameter $\mathcal{W}$ using human evaluations from the training data. Specifically, we fit a univariate rating model using win rates for a given $\mathcal{W}$ on the classical benchmark and evaluate the logistic loss of the resulting ratings on the training data. The parameter with the lowest logistic loss is selected. Importantly, we do not use any unknown test data during this optimization process, ensuring that our approach can be applied in practical scenarios without compromising the integrity of the evaluation.

\begin{table}[t]
    \centering
    \footnotesize
    \caption{Overview of all biases used in \cref{sec:experiments:bias}. The table contains a description of the bias and a functional form of the bias. Scaling constant were introduced in these functional forms to ensure that all biases output values within the same order of magnitude.}
    \label{tab:biases:description}
    \begin{tabular}{>{\raggedright}p{0.11\textwidth} >{\raggedright\arraybackslash}p{0.4\textwidth} >{\raggedright\arraybackslash}p{0.4\textwidth}}
        \toprule
        \textbf{Bias} & \textbf{Description} & \textbf{Functional Form} \\
        \midrule
        Length & Measures the length of a model answer for a given question. & $
        f(g, i) = \log_{10}(\text{length}(g_{m_i}(g_{p})))$\\
        Position & Computes the order of the model in the game. & $f(g, i) = \iverson{i = 1}$\\
        Formality & Computes the formality of an answer computed by a popular formality classifier \citep{formality}.\footnotemark[1] & $f(g, i) = \mathcal{M}(g_{m_i}(g_{p}))_1$ \\
        Sentiment & Computes the sentiment of an answer computed by a popular sentiment classifier \citep{sentiment}.\footnotemark[2] & $f(g, i) = \mathcal{M}(g_{m_i}(g_{p}))_2$\\
        Repetitiveness & Computes the repetitiveness of the answer by computing the percentage of non-unique words in the answer. & $f(g, i) = 5 \cdot \frac{\text{\# of repeated words in }g_{m_i}(g_{p})}{\text{\# of words in }g_{m_i}(g_{p})}$ \\
        Readability & Computes the Flesch Reading Ease score \citep{kincaid1975derivation} of an answer. & $f(g, i) = \min(1, \max(0, \frac{\text{Flesch}(g_{m_i}(g_{p}))}{100}))$\\
        \bottomrule
    \end{tabular}
\end{table}
\footnotetext[1]{{\href{https://huggingface.co/s-nlp/roberta-base-formality-ranker}{https://huggingface.co/s-nlp/roberta-base-formality-ranker}}}
\footnotetext[2]{{\href{https://huggingface.co/cardiffnlp/twitter-roberta-base-sentiment-latest}{https://huggingface.co/cardiffnlp/twitter-roberta-base-sentiment-latest}}}

\begin{table}[t]
    \centering
    \footnotesize
    \caption{Overview of all tasks used in \cref{sec:experiments}. For each task, we use the same data as the actual Chatbot Arena \citep{chatbot_arena}}
    \label{tab:categories:description}
    \begin{tabular}{>{\raggedright}p{0.15\textwidth} >{\raggedright\arraybackslash}p{0.75\textwidth}}
        \toprule
        \textbf{Task} & \textbf{Description} \\
        \midrule
        English & Questions that are in English. \\
        Chinese & Questions that are in Chinese. \\
        Hardness & Questions that are considered hard by the Chatbot Arena. These are questions that are classified as being in at least six of the following seven categories: specific, requires domain knowledge, is complex, requires problem-solving, requires creative thinking, requires technical accuracy, is a real-world question. \\
        Code & Questions that require code to be answered. \\
        LLM & Whether the judge is a language model. \\
        \bottomrule
    \end{tabular}
\end{table}
