# Supplementary material for: CreDes: Causal Reasoning Enhancement and Dual-End Searching for Solving Long-Range Reasoning Problems using LLMs
Source: arXiv:2410.01696 source file (2024-10-02)
Supplement: Supplementary file 5 [file appendix-proofs.tex]

\newpage
\section{Proofs}\label{app:proofs}

We provide the proofs for the theorems mentioned in the main text here.

We first prove the convexity of the optimization objective in \cref{eq:multi-logistic-loss}.

\begin{theorem}[Convexity of the Optimization Objective]\label{thm:convexity}
    The optimization objective in \cref{eq:multi-logistic-loss} is convex and twice differentiable.
\end{theorem}
\begin{proof}
 Twice differentiability follows immediately from the twice differentiability of the logistic loss and the squared penalty term. To show convexity, we make use of the following well-known facts about convex functions:
    \begin{itemize}
        \item The sum of two convex functions is convex.
        \item The composition of a convex function with an affine function is convex.
    \end{itemize}
Since the logistic loss $f(x) = -\log(1 + \exp(x))$ is convex, and since \tool relies on a linear combination of parameters in the loss function, the logistic loss is convex in these parameters. The squared penalty term is also convex, as it is a sum of squared terms with a positive quadratic coefficient. The sum of two convex functions is convex, so the optimization objective is convex.
\end{proof}

Further, we show the optimality of \tool by showing it converges to the same optimal rating as the univariate approach when fitted on multiple tasks at the same time.

For this purpose, suppose we have a task for which we want to obtain a separate rating. Specifically, let $D$ be a dataset of games between models. Let $D_{\neg \text{task}} \subset D$, resp. $D_{\text{task}}\subset D$, be the set of games not belonging to, resp. belonging to, the task of interest. We show that as $|D| \rightarrow \infty$, the rating obtained by individually fitting the tasks is equivalent to the rating obtained by fitting all tasks simultaneously using \tool. Intuitively, the extra prior term in \tool will be of less importance as the number of games in the task of interest increases, and the ratings will converge to the same optimal rating. 

\begin{theorem} [Equivalence of Ratings]\label{thm:equivalence}
    Let $D$ be a set of i.i.d. games between models $m_0, \dots, m_{k-1}$. Let $D_{\text{task}} \subset D$ and $D_{\neg \text{task}} \subset D$ be as defined above. Let $\mathbf{R}_{\text{task}}$, resp. $\mathbf{R}_{\neg \text{task}}$, be the rating obtained by fitting the games in $D_{\text{task}}$, resp. $D_{\neg \text{task}}$, using the optimal univariate rating system. Let $\mathbf{R'}$ be the rating obtained by fitting all games in $D$ simultaneously using \tool with the formula $R'^{m}(g) = R'^{m}_{\neg \text{task}} + \beta^{m}_{1} \iverson{g \in D_{\text{task}}}$ and define $R'^{m}_{\text{task}} = R'^{m}_{\neg \text{task}} + \beta^{m}_{1}$. Finally, let the priors on respectively $R'^{m}_{\neg \text{task}}$ and $\beta^{m}_{1}$ be $\mathcal{N}(0, \sigma_{\neg \text{task}}^2)$ and $\mathcal{N}(0, \sigma_{1}^2)$. Then, as $|D_{\neg \text{task}}| \rightarrow \infty$ and $|D_{\text{task}}| \rightarrow \infty$, $\mathbf{R}_{\text{task}}$ and $\mathbf{R'}_{\text{task}}$ will, up to a constant difference, converge to the same optimal rating $\mathbf{R}_{\text{task}}^*$  if all optimal ratings are finite. Similarly, $\mathbf{R}_{\neg \text{task}}$ and $\mathbf{R'}_{\neg \text{task}}$ will, up to a constant difference, converge to the same optimal rating $\mathbf{R}_{\neg \text{task}}^*$  if all optimal ratings are finite.
\end{theorem}

To prove the theorem, we first need several lemmas.

\begin{lemma}[Shift-Invarance of Optimal Ratings]\label{lem:shift-invariance}
    Let $D$ be a set of games between models $m_0, \dots, m_{k-1}$ where there exists one model that has played all other models at least once. If $\mathbf{R}_1$ and $\mathbf{R}_2$ both minimize the logistic loss $\mathcal{L}(D, \mathbf{R})$ for $D$, then $\mathbf{R}_1 - \mathbf{R}_2$ is a constant vector.
\end{lemma}

\begin{proof}
    Without loss of generality, we can assume that the first model is the model that has played all other models at least once. We first note that for any constant $c \in \mathbb{R}$, it holds that $\mathcal{L}(D, \mathbf{R} + c) = \mathcal{L}(D, \mathbf{R})$. Therefore, we can assume that the first element of each vector, namely $\mathbf{R}_1^{0}$ and $\mathbf{R}_2^{0}$, are both zero by applying a constant shift to both. We now show that $\mathbf{R}_1=\mathbf{R}_2$. 
    
    We do so by proving that the function $F(x_1, \dots x_{k-1}) = \mathcal{L}(D, (0, x_1, ..., x_{k-1}))$ is strictly convex. Since strictly convex functions have a unique minimum, this implies that $\mathbf{R}_1 = \mathbf{R}_2$. We show strict convexity by computing the Hessian and showing that it is diagonally dominant with strictly positive diagonal elements. By Gershgorin circle theorem, this implies that the Hessian cannot have eigenvalues equal to zero, and is therefore positive definite. Since the Hessian is positive definite, the function is strictly convex, and the result follows.

    We compute the diagonal terms of the Hessian of $F$. We denote by $D_{\{i, j\}}$ all games where one model is $m_i$ and the other model is $m_j$. We slightly change the notation such that the game result $g_r \in D_{\{i, j\}}$ indicates whether $m_i$ won or lost, no matter the order of the models. We define $x_0 = 0$ and drop the division by $400$ for convenience. We have:

    \begin{equation*}
        F(x_1, \dots x_{k-1}) = \sum_{i=0}^{k-1}\sum_{j=0}^{k-1} \sum_{g \in D_{\{i, j\}}} g_r \log(1 + \exp(x_j - x_i))
    \end{equation*}

    Thus,

    \begin{align*}
        \frac{\partial^2 F}{\partial x_i^2} &= \sum_{j=0}^{k - 1}\sum_{g \in D_{\{i, j\}}} g_r \frac{\exp(x_j - x_i)}{(1 + \exp(x_j - x_i))^2}  + (1 - g_r) \frac{\exp(x_i - x_j)}{(1 + \exp(x_i - x_j))^2} \\
        &= \sum_{g \in D_{\{i, 0\}}} g_r \frac{\exp(-x_i)}{(1 + \exp(-x_i))^2}  + (1 - g_r) \frac{\exp(x_i)}{(1 + \exp( x_i))^2} + \sum_{j=1}^{k - 1} -\frac{\partial^2 F}{\partial x_i \partial x_j}\\
    \end{align*}
    Since all terms in the sum are positive, the diagonal terms of the Hessian are strictly positive. Furthermore, the Hessian is diagonally dominant as the last sum is the sum over all off-diagonal terms in the same column and the first sum is strictly positive since $m_i$ has played at least one game against $m_0$. Thus, the Hessian is positive definite, and the function is strictly convex.
\end{proof}

\begin{lemma}[Limit Exists and Is Finite]\label{lem:limit}
    Let $D$ be a set of i.i.d. games between models $m_0, \dots, m_{k-1}$. Furthermore, assume all ratings are bounded. Then,
    \begin{equation}\label{eq:limit:1}
        \lim_{|D| \rightarrow \infty} \frac{1}{|D|} \min_{\mathbf{R}} \mathcal{L}(D, \mathbf{R})
    \end{equation} 
    almost surely uniformly converges to $\mathbb{E}_g(\mathcal{L}(g, \mathbf{R}))$. Furthermore,
    \begin{equation}\label{eq:limit:2}
        \lim_{|D| \rightarrow \infty} \argmin_{\mathbf{R}, \mathbf{R}_0 = 0} \mathcal{L}(D, \mathbf{R})
    \end{equation} 
    almost surely exists and converges to the optimal rating.
\end{lemma}
\begin{proof}
    Let $D_n$ be the first $n$ games in $D$. We show that the functions $\mathcal{L}_n : \mathbb{R}^{k} \rightarrow \mathbb{R}$ defined by $\mathcal{L}_n(\mathbf{R}) = \frac{1}{n} \mathcal{L}(D_n, \mathbf{R})$ converge uniformly to $\mathbb{E}_g(\mathcal{L}(g, \mathbf{R}))$.

    Thus, for any given $\epsilon > 0$ we need to prove the existence of an $N$ such that for all $n > N$ and all $\mathbf{R}$, $|\mathcal{L}_n(\mathbf{R}) - \mathbb{E}_g(\mathcal{L}(g, \mathbf{R}))| < \epsilon$. Let $\epsilon > 0$ be chosen arbitrarily. We can group games with the same models together in the notation for $\mathcal{L}_n$. More specifically, let $w_{i, j}^{(n)}$ denote the weight of the coefficient associated with $\log(1 + \exp(-R_{i}^{m} + R_{j}^{m}))$. Then we can write:
    \begin{equation*}
        \frac{\mathcal{L}_n(\mathbf{R})}{n} = \sum_{i=1}^{k}\sum_{j=1}^{k} \frac{w_{i, j}^{(n)}}{n} \log(1 + \exp(-R_{i}^{m} + R_{j}^{m}))
    \end{equation*}
    Furthermore, we can write the expected value of the loss as:
    \begin{align*}
        \mathbb{E}_g(\mathcal{L}(g, \mathbf{R})) &= \sum_{i=1}^{k}\sum_{j=1}^{k} \left(P(i \succ j) + 0.5 \cdot P(i\simeq j)\right) \cdot P(g \in D_{\{i, j\}}) \log(1 + \exp(-R_{i}^{m} + R_{j}^{m}))\\
        &:= \sum_{i=1}^{k}\sum_{j=1}^{k} P_{i, j}\log(1 + \exp(-R_{i}^{m} + R_{j}^{m}))
    \end{align*}
    where $\simeq$ denotes a draw.

    Thus, we obtain:
    \begin{align*}
        \frac{\mathcal{L}_n(\mathbf{R})}{n} - \mathbb{E}_g(\mathcal{L}(g, \mathbf{R})) = \sum_{i=1}^{k}\sum_{j=1}^{k} & \left(\frac{w_{i, j}^{(n)}}{n} - P_{i, j}\right) \cdot \log(1 + \exp(-R_{i}^{m} + R_{j}^{m}))
    \end{align*}
    By the strong law of large numbers, the weights $w_{i, j}^{(n)} / n$ converge almost surely to the expected value of the weights, i.e. $P_{i, j}$. Furthermore, since the ratings are finite, $\log(1 + \exp(-R_{i}^{m} + R_{j}^{m}))$ can be bounded by a constant $B$. Thus, for any $\epsilon > 0$, there exists an $N$ such that for all $n > N$, $|\frac{w_{i, j}^{(n)}}{n} - P_{i, j}| < \frac{\epsilon}{Bk^2}$ for all $i, j$. Then, almost surely,
    \begin{align*}
        \left|\frac{\mathcal{L}_n(\mathbf{R})}{n} - \mathbb{E}_g(\mathcal{L}(g, \mathbf{R}))\right| &\leqslant \sum_{i=1}^{k}\sum_{j=1}^{k} \left|\frac{w_{i, j}^{(n)}}{n} - P_{i, j}\right| B \\
        &\leqslant  \frac{\epsilon}{Bk^2} \cdot Bk^2 = \epsilon,
    \end{align*}
    proving the first part of the lemma.

    For the second part, we note that \cref{lem:shift-invariance} implies that $\argmin_{\mathbf{R}, \mathbf{R}_0 = 0} \mathcal{L}_n(\mathbf{R})$ has a unique solution. By uniform convergence on a compact domain of continuous functions $\mathcal{L}_n$, we thus have that the limit of the minimizers of $\mathcal{L}_n$ is the minimizer of the expected loss, and the result follows.
\end{proof}

Now, we can prove \cref{thm:equivalence}.

\begin{proof}
We prove that $\mathbf{R}_{\text{task}}$ and $\mathbf{R'}_{\text{task}}$ will converge to the same optimal rating $\mathbf{R}_{\text{task}}^*$ assuming that $\mathbf{R}_{\text{task}, 0} = \mathbf{R'}_{\text{task}, 0} = \mathbf{R}_{\text{task}, 0}^{*} = 0$ which can be assumed due to shift-invariance. The other implication is proven equivalently.

Let $D_\text{task}^{(n)}$ denote the first $n$ elements of $D_\text{task}$ and $\mathbf{R}_{\text{task}}^{(n)}$ the optimal solutions found when fitting using $D_\text{task}^{(n)}$. Note that we leave the size of $D_{\neg \text{task}}$ in the sequence unspecified since it does not matter for this part of the proof. We note that \tool optimizes the loss
\begin{equation}\label{eq:multi-logistic-loss:proof}
    \mathcal{L}^{(n)}_{\text{full}}(D^{(n)}, \mathbf{R'}) = \frac{1}{n}\mathcal{L}(D_{\neg \text{task}}, \mathbf{R'}_{\neg \text{task}}) + \frac{1}{n}\mathcal{L}(D_\text{task}^{(n)}, \mathbf{R'}_{\text{task}}) + \frac{1}{n}\sum_{j=0}^{d} \frac{\mathbf{R'}_{\neg \text{task}, j}^2}{2 \sigma_{\neg \text{task}}^2} + \frac{1}{n} \sum_{j=0}^{d} \frac{\beta_{1, j}^2}{2 \sigma_{1}^2}
\end{equation}
with optimal solution $\mathbf{R'}^{(n)}$. Suppose now that $\mathbf{R'}^{(n)}_{\text{task}}$ does not converge to $\mathbf{R}_{\text{task}}^*$. Then there exists a subsequence $n_i$ and a $\delta > 0$ such that $||\mathbf{R'}_{\text{task}}^{(n_i)} - \mathbf{R}_{\text{task}}^*|| > \delta$. Without loss of generalization, we can assume this subsequence is the full sequence.

By \cref{lem:limit}, we know that $\frac{1}{n}\mathcal{L}(D^{(n)}_{\text{task}}, \mathbf{R})$ uniformly converges to the function $\mathcal{L}^*(\mathbf{R}) := \mathbb{E}_{g_{\text{task}}}(\mathcal{L}(g_{\text{task}}, \mathbf{R}))$ which has $\mathbf{R}_{\text{task}}^*$ as minimizer. By \cref{lem:shift-invariance}, $\mathcal{L}^*$ is continuous and has a unique minimum that satisfies $\mathbf{R}_{\text{task}, 0}^* = 0$. Therefore, there exists an $\epsilon > 0$ such that for all ratings $\mathbf{R}$ with $\mathbf{R}_0 = 0$ the following is true:
\begin{equation}\label{eq:proof:epsilon}
||\mathbf{R} - \mathbf{R}_{\text{task}}^*|| > \delta \Rightarrow \mathcal{L}^*(\mathbf{R}) - \mathcal{L}^*(\mathbf{R}_{\text{task}}^*) > \epsilon.
\end{equation}

Since $\mathbf{R}_{\text{task}}^{(n)}$ converges to $\mathbf{R}_{\text{task}}^*$ by \cref{lem:limit}, we know there is an $n_0 > 0$ such that for each $n > n_0$, 
\begin{equation}\label{eq:proof:epsilon2}
    \mathcal{L}^*(\mathbf{R}_{\text{task}}^{(n)}) - \mathcal{L}^*(\mathbf{R}_{\text{task}}^*) < \frac{\epsilon}{4}. 
\end{equation}

Furthermore, due to the uniform convergence of the loss, there exists an $n_1 > 0$ such that for all $n > n_1$ and all $\mathbf{R}$, 
\begin{equation}\label{eq:proof:uniform}
    \left|\frac{1}{n}\mathcal{L}(D_\text{task}^{(n)}, \mathbf{R}) - \mathcal{L}^*(\mathbf{R})\right| < \frac{\epsilon}{4}.
\end{equation}
Finally, there exists an $n_2 > 0$ such that for all $n > n_2$, 
\begin{equation}\label{eq:proof:epsilon3}
    \left|\frac{d+1}{n}\frac{B^2}{2 \sigma_{\neg \text{task}}^2} + \frac{d+1}{n} \frac{4B^2}{2 \sigma_{1}^2}\right| < \frac{\epsilon}{4}
\end{equation}
where $B$ is the upper bound for all ratings. 

However, we can now define $\mathbf{R''}^{(n)}_{\neg \text{task}} = \mathbf{R'}^{(n)}_{\neg \text{task}}$ and $\beta''^{(n)} = \mathbf{R}_{\text{task}}^{(n)} - \mathbf{R'}^{(n)}_{\neg \text{task}}$. The inequalities above imply that for all $n > \max(n_0, n_1, n_2)$, $\mathcal{L}_{\text{full}}^{(n)}(D^{(n)}, \mathbf{R''}^{(n)}) < \mathcal{L}_{\text{full}}^{(n)}(D^{(n)}, \mathbf{R'}^{(n)})$, since

\begin{align*}
    \frac{1}{n}\mathcal{L}(D_\text{task}^{(n)}, \mathbf{R'}_{\text{task}})  - \frac{1}{n}\mathcal{L}(D_\text{task}^{(n)}, \mathbf{R}_{\text{task}})
    &> \mathcal{L}^*(\mathbf{R'}_{\text{task}}) - \frac{\epsilon}{4} - \mathcal{L}^*(\mathbf{R}_{\text{task}}) - \frac{\epsilon}{4} \\
    &=  \mathcal{L}^*(\mathbf{R'}_{\text{task}})- \mathcal{L}^*(\mathbf{R}^*_{\text{task}}) + \mathcal{L}^*(\mathbf{R}^*_{\text{task}}) - \mathcal{L}^*(\mathbf{R}_{\text{task}})  - \frac{\epsilon}{2} \\
    &> \epsilon - \frac{\epsilon}{4} - \frac{\epsilon}{2} = \frac{\epsilon}{4}
\end{align*}
where the first inequality follows from \cref{eq:proof:uniform} and the last from \cref{eq:proof:epsilon} and \cref{eq:proof:epsilon2}. Since \cref{eq:proof:epsilon3} ensures that the difference in the bias term can at most differ by $\epsilon / 4$, we find $\mathcal{L}_{\text{full}}^{(n)}(D^{(n)}, \mathbf{R''}^{(n)}) < \mathcal{L}_{\text{full}}^{(n)}(D^{(n)}, \mathbf{R'}^{(n)})$. Therefore, $\mathbf{R'}^{(n)}_{\text{task}}$ cannot be the optimal solution, which is a contradiction to the optimality of $\mathbf{R'}^{(n)}$. Therefore, $\mathbf{R'}_{\text{task}}$ must converge to $\mathbf{R}_{\text{task}}^*$.

\end{proof}
