# Supplementary material for: CreDes: Causal Reasoning Enhancement and Dual-End Searching for Solving Long-Range Reasoning Problems using LLMs
Source: arXiv:2410.01696 source file (2024-10-02)
Supplement: Supplementary file 6 [file appendix-results.tex]

\newpage
\begin{table}[!ht]
    \centering
    \footnotesize
    \caption{Fitted coefficients for the biases and their average influence on the ratings of the models for both human and LLM-based evaluation. The functional form of $f_{\text{bias}}$ used for each bias can be found in \cref{app:details}. The influence is computed as $\mathbb{E}_g(\alpha_{\text{bias}} \cdot |f_{\text{bias}}(g, 0) - f_{\text{bias}}(g, 1)|)$ and indicates the average influence the bias has on the rating of models for specific games. Errors shown are $95\%$ pivot intervals computed using bootstrapping.}
    \label{tab:biases-full}
    \begin{subtable}[t]{0.48\textwidth}
        \centering
        \caption{Human Evaluation}
        \label{tab:biases:human-full}
        {
        
        \begin{tabular}{lll}
            \toprule
            Bias & {Coefficient $(\alpha)$} & {Influence $(\mathbb{E})$} \\
            \midrule
            
            Length & $\phantom{-}130.74_{-7.3}^{+7.9}$ & $\phantom{-}40.84_{-2.3}^{+2.5}$ \\
            Position & $\phantom{-00}2.70_{-2.4}^{+2.3}$ & $\phantom{-0}2.70_{-2.4}^{+2.3}$ \\
            Formality & $-119.89_{-11.4}^{+11.6}$
 & $-15.17_{-1.4}^{+1.5}$ \\
            Sentiment & $\phantom{-0}57.42_{-10.9}^{+10.1}$ & $\phantom{-0}7.90_{-1.5}^{+1.4}$ \\
            Repetitiveness & $- \phantom{0} 22.10_{-8.4}^{+8.5}$ & $-\phantom{0}4.64_{-1.8}^{+1.8}$ \\
            Readability & $\phantom{-0}72.93_{-11.6}^{+11.0}$ & $\phantom{-}10.75_{-1.7}^{+1.6}$ \\
            
            \bottomrule
        \end{tabular}
        }
    \end{subtable}
    \hfill
    \begin{subtable}[t]{0.48\textwidth}
        \centering
        \caption{LLM-based Evaluation}
        \label{tab:biases:llm-full}
        {
        
        \begin{tabular}{lll}
            \toprule
            Bias & {Coefficient $(\alpha)$} & {Influence $(\mathbb{E})$} \\
            \midrule
            Length & $\phantom{-}251.87_{-6.8}^{+7.3}$ & $\phantom{-}48.48_{-1.3}^{+1.4}$ \\
            Position & $\phantom{-0}37.53_{-1.2}^{+1.1}$ & $\phantom{-}37.53_{-1.2}^{+1.1}$ \\
            Formality & $-\phantom{0}37.56_{-7.2}^{+6.7}$ & $-\phantom{0}4.31_{-0.8}^{+0.8}$ \\
            Sentiment & $\phantom{-00}4.31_{-6.7}^{+6.1}$ & $\phantom{-0}0.43_{-0.7}^{+0.6}$ \\
            Repetitiveness &  $\phantom{-0}75.04_{-7.3}^{+8.8}$ & $\phantom{-0}9.12_{-0.9}^{+1.1}$ \\
            Readability & $-\phantom{0}32.56_{-7.9}^{+8.1}$ & $-\phantom{0}3.92_{-0.9}^{+1.0}$ \\
            \bottomrule
        \end{tabular}
        }
        
    \end{subtable}
    
\end{table}
\newpage
\section{Detailed Results}\label{app:results}

In \cref{tab:biases-full}, we show \cref{tab:biases} with the adjusted confidence intervals computed using pivot intervals instead of $2\sigma$ intervals.

The full multidimensional leaderboard fitted using \tool on Chatbot Arena data \citep{chatbot_arena} can be found in \cref{tab:leaderboard}. The full leaderboard fitted using a unidimensional approach can be found in \cref{tab:leaderboard-single}.

\begin{footnotesize}
    {
    
    \begin{longtable}[t]{lllllll}
        \caption{Leaderboard of human evaluation with modifiers fitted with \tool. Indicated deviations are $95\%$ pivot intervals determined using bootstrapping.} \label{tab:leaderboard} \\
        
        \toprule
        Rank & Model Name & Rating & English & Chinese & Hardness & Code \\
        \midrule
        \endfirsthead
    
        \caption[]{(continued)} \\
        \toprule
        Rank & Model Name & Rating & English & Chinese & Hardness & Code \\
        \midrule
        \endhead
    
        \bottomrule
        \endfoot
    
        \bottomrule
        \endlastfoot
    
        1 & gpt-4o-2024-05-13 & $1297_{-4.2}^{+4.5} $ & $-13_{-10.3}^{+4.3} $ & $-\phantom{00}3_{-8.2}^{+8.8} $ & $\phantom{-} 13_{-4.8}^{+10.0} $ & $\phantom{-} 15_{-5.7}^{+10.4} $ \\
        2 & claude-3-5-sonnet-20240620 & $1286_{-7.4}^{+6.7} $ & $-29_{-13.9}^{+8.2} $ & $-\phantom{0}19_{-12.9}^{+15.0} $ & $\phantom{-} 14_{-8.5}^{+13.6} $ & $\phantom{-} 44_{-10.6}^{+14.9} $ \\
        3 & gemini-advanced-0514 & $1285_{-5.1}^{+4.5} $ & $-26_{-10.7}^{+4.5} $ & $\phantom{-} \phantom{00}8_{-9.4}^{+9.2} $ & $\phantom{-} \phantom{0}3_{-5.6}^{+10.3} $ & $\phantom{-} \phantom{0}2_{-6.9}^{+11.2} $ \\
        4 & gemini-1.5-pro-api-0514 & $1273_{-4.5}^{+4.8} $ & $-20_{-10.5}^{+4.8} $ & $\phantom{-} \phantom{0}19_{-8.6}^{+10.0} $ & $\phantom{-} 15_{-4.8}^{+10.0} $ & $\phantom{-} 11_{-5.8}^{+11.3} $ \\
        5 & claude-3-opus-20240229 & $1273_{-2.7}^{+3.0} $ & $-39_{-9.2}^{+2.5} $ & $\phantom{-} \phantom{00}1_{-5.1}^{+6.0} $ & $\phantom{-} 15_{-2.9}^{+8.4} $ & $\phantom{-} 12_{-3.7}^{+8.4} $ \\
        6 & bard-jan-24-gemini-pro & $1271_{-12.6}^{+12.4} $ & $-48_{-16.9}^{+11.7} $ & $-\phantom{0}25_{-25.8}^{+25.6} $ & $-45_{-11.7}^{+16.9} $ & $-11_{-13.4}^{+19.0} $ \\
        7 & gpt-4-1106-preview & $1265_{-4.0}^{+3.7} $ & $-11_{-9.7}^{+3.5} $ & $-\phantom{00}3_{-7.2}^{+8.0} $ & $\phantom{-} \phantom{0}9_{-3.5}^{+8.7} $ & $\phantom{-} 11_{-4.8}^{+9.3} $ \\
        8 & gemini-1.5-pro-api-0409-preview & $1264_{-4.4}^{+4.6} $ & $-\phantom{0}2_{-10.1}^{+4.1} $ & $\phantom{-} \phantom{00}5_{-8.5}^{+7.9} $ & $-\phantom{0}4_{-4.8}^{+9.8} $ & $-12_{-5.5}^{+10.8} $ \\
        9 & gpt-4-turbo-2024-04-09 & $1258_{-3.4}^{+3.8} $ & $\phantom{-} \phantom{0}3_{-9.8}^{+3.6} $ & $\phantom{-} \phantom{00}4_{-6.6}^{+7.4} $ & $\phantom{-} 11_{-3.8}^{+8.9} $ & $\phantom{-} 15_{-4.9}^{+9.6} $ \\
        10 & gpt-4-0125-preview & $1255_{-3.6}^{+3.6} $ & $-\phantom{0}5_{-9.6}^{+3.5} $ & $\phantom{-} \phantom{00}1_{-6.1}^{+7.3} $ & $\phantom{-} 14_{-3.9}^{+9.0} $ & $\phantom{-} \phantom{0}2_{-4.7}^{+9.5} $ \\
        11 & gemini-1.5-flash-api-0514 & $1243_{-4.5}^{+4.7} $ & $-21_{-10.5}^{+4.5} $ & $\phantom{-} \phantom{00}8_{-9.7}^{+9.5} $ & $\phantom{-} \phantom{0}9_{-5.5}^{+10.4} $ & $\phantom{-} 15_{-6.7}^{+10.8} $ \\
        12 & yi-large-preview & $1237_{-4.4}^{+4.4} $ & $-\phantom{0}4_{-10.6}^{+4.1} $ & $\phantom{-} \phantom{0}37_{-8.6}^{+8.8} $ & $\phantom{-} 17_{-4.8}^{+10.5} $ & $\phantom{-} 11_{-5.8}^{+11.0} $ \\
        13 & gemma-2-27b-it & $1232_{-11.4}^{+11.7} $ & $-10_{-17.6}^{+12.2} $ & $-\phantom{00}1_{-19.6}^{+23.2} $ & $-15_{-13.6}^{+18.0} $ & $\phantom{-} \phantom{0}7_{-15.7}^{+19.9} $ \\
        14 & yi-large & $1222_{-7.7}^{+8.8} $ & $-\phantom{0}3_{-15.5}^{+8.5} $ & $\phantom{-} \phantom{00}9_{-16.5}^{+17.9} $ & $\phantom{-} 11_{-10.4}^{+15.4} $ & $\phantom{-} 21_{-12.5}^{+18.2} $ \\
        15 & nemotron-4-340b-instruct & $1222_{-7.2}^{+6.5} $ & $-13_{-13.1}^{+7.6} $ & $\phantom{-} \phantom{00}7_{-12.4}^{+13.9} $ & $\phantom{-} \phantom{0}9_{-8.5}^{+13.2} $ & $-\phantom{0}6_{-9.4}^{+14.7} $ \\
        16 & claude-3-sonnet-20240229 & $1220_{-3.2}^{+3.3} $ & $-26_{-9.4}^{+2.8} $ & $-\phantom{0}15_{-5.5}^{+5.9} $ & $\phantom{-} \phantom{0}6_{-3.6}^{+8.3} $ & $\phantom{-} 26_{-3.7}^{+9.2} $ \\
        17 & command-r-plus & $1214_{-3.5}^{+3.9} $ & $-18_{-9.4}^{+3.4} $ & $\phantom{-} \phantom{00}6_{-6.4}^{+6.7} $ & $-\phantom{0}7_{-3.7}^{+9.0} $ & $-14_{-4.4}^{+9.3} $ \\
        18 & gpt-4-0314 & $1213_{-4.5}^{+4.5} $ & $-29_{-10.4}^{+4.3} $ & $-\phantom{0}13_{-7.9}^{+8.7} $ & $\phantom{-} 23_{-4.6}^{+9.7} $ & $\phantom{-} \phantom{0}9_{-4.9}^{+10.5} $ \\
        19 & reka-core-20240501 & $1212_{-3.9}^{+3.6} $ & $-11_{-9.8}^{+3.7} $ & $\phantom{-} \phantom{00}9_{-7.6}^{+8.1} $ & $\phantom{-} \phantom{0}6_{-4.7}^{+9.3} $ & $-\phantom{0}2_{-4.6}^{+10.4} $ \\
        20 & claude-3-haiku-20240307 & $1209_{-3.4}^{+3.5} $ & $-30_{-9.2}^{+3.2} $ & $-\phantom{0}36_{-5.2}^{+6.0} $ & $\phantom{-} 10_{-3.4}^{+8.4} $ & $\phantom{-} 16_{-3.6}^{+9.0} $ \\
        21 & gemma-2-9b-it & $1204_{-10.7}^{+11.0} $ & $-17_{-17.5}^{+12.6} $ & $-\phantom{00}1_{-22.1}^{+21.4} $ & $\phantom{-} \phantom{0}3_{-12.6}^{+18.6} $ & $-14_{-16.3}^{+20.3} $ \\
        22 & glm-4-0520 & $1202_{-9.6}^{+10.0} $ & $\phantom{-} \phantom{0}8_{-15.8}^{+10.8} $ & $\phantom{-} \phantom{0}49_{-17.7}^{+17.8} $ & $\phantom{-} 19_{-11.1}^{+15.7} $ & $\phantom{-} 12_{-12.5}^{+17.4} $ \\
        23 & gpt-4-0613 & $1191_{-3.7}^{+3.8} $ & $-22_{-9.5}^{+3.6} $ & $-\phantom{0}41_{-6.5}^{+7.6} $ & $\phantom{-} 18_{-3.7}^{+8.5} $ & $\phantom{-} \phantom{0}1_{-4.2}^{+9.5} $ \\
        24 & claude-1 & $1190_{-8.2}^{+8.3} $ & $-30_{-14.5}^{+7.9} $ & $-\phantom{0}18_{-17.0}^{+16.9} $ & $-19_{-7.6}^{+13.3} $ & $\phantom{-} \phantom{0}4_{-9.4}^{+14.8} $ \\
        25 & reka-flash-preview-20240611 & $1188_{-7.6}^{+7.7} $ & $-15_{-13.8}^{+7.3} $ & $-\phantom{00}5_{-15.0}^{+14.1} $ & $-10_{-9.0}^{+13.8} $ & $\phantom{-} \phantom{0}7_{-10.6}^{+15.4} $ \\
        26 & llama-3-70b-instruct & $1187_{-2.7}^{+3.0} $ & $\phantom{-} 67_{-9.0}^{+2.3} $ & $-\phantom{0}51_{-5.0}^{+5.7} $ & $-\phantom{0}1_{-2.5}^{+7.8} $ & $-10_{-3.3}^{+8.6} $ \\
        27 & qwen-max-0428 & $1187_{-5.1}^{+5.4} $ & $\phantom{-} \phantom{0}3_{-11.6}^{+5.4} $ & $\phantom{-} \phantom{0}62_{-11.3}^{+12.9} $ & $\phantom{-} 11_{-7.1}^{+11.2} $ & $\phantom{-} \phantom{0}8_{-7.9}^{+12.3} $ \\
        28 & qwen2-72b-instruct & $1182_{-6.0}^{+6.0} $ & $\phantom{-} \phantom{0}9_{-12.9}^{+5.4} $ & $\phantom{-} \phantom{0}68_{-11.0}^{+11.9} $ & $\phantom{-} 13_{-6.8}^{+11.6} $ & $-\phantom{0}3_{-7.6}^{+13.4} $ \\
        29 & gemini-pro-dev-api & $1182_{-7.2}^{+8.1} $ & $-38_{-13.6}^{+7.2} $ & $-\phantom{0}23_{-14.0}^{+15.1} $ & $-11_{-8.7}^{+13.3} $ & $-23_{-9.2}^{+14.3} $ \\
        30 & deepseek-coder-v2 & $1181_{-9.3}^{+9.4} $ & $-34_{-15.6}^{+9.6} $ & $\phantom{-} \phantom{0}16_{-17.5}^{+17.3} $ & $\phantom{-} 43_{-11.0}^{+15.5} $ & $\phantom{-} 64_{-11.5}^{+18.1} $ \\
        31 & reka-flash-21b-20240226-online & $1176_{-7.1}^{+6.9} $ & $-12_{-13.3}^{+6.9} $ & $-\phantom{0}10_{-12.1}^{+13.3} $ & $-\phantom{0}2_{-8.1}^{+13.0} $ & $\phantom{-} \phantom{0}1_{-9.4}^{+13.4} $ \\
        32 & command-r & $1175_{-3.9}^{+4.2} $ & $-15_{-9.9}^{+3.9} $ & $\phantom{-} \phantom{0}12_{-6.8}^{+7.5} $ & $-23_{-4.6}^{+9.3} $ & $-\phantom{0}9_{-5.3}^{+10.6} $ \\
        33 & reka-flash-21b-20240226 & $1170_{-5.2}^{+5.6} $ & $-16_{-11.7}^{+5.2} $ & $-\phantom{0}12_{-11.7}^{+10.1} $ & $-\phantom{0}6_{-6.4}^{+11.7} $ & $\phantom{-} \phantom{0}5_{-7.2}^{+11.5} $ \\
        34 & claude-2.0 & $1164_{-10.4}^{+10.8} $ & $-26_{-15.8}^{+9.9} $ & $-\phantom{00}8_{-23.1}^{+24.1} $ & $\phantom{-} \phantom{0}3_{-10.9}^{+15.1} $ & $\phantom{-} 12_{-13.0}^{+17.6} $ \\
        35 & mistral-large-2402 & $1163_{-4.2}^{+4.0} $ & $\phantom{-} \phantom{0}2_{-10.0}^{+3.8} $ & $-\phantom{0}32_{-7.1}^{+7.7} $ & $\phantom{-} 20_{-4.2}^{+9.0} $ & $\phantom{-} 10_{-5.3}^{+9.9} $ \\
        36 & gpt-3.5-turbo-0314 & $1162_{-21.0}^{+19.5} $ & $-56_{-25.0}^{+19.3} $ & $\phantom{-} \phantom{00}9_{-32.4}^{+31.9} $ & $\phantom{-} 22_{-18.2}^{+22.7} $ & $\phantom{-} 14_{-21.9}^{+27.5} $ \\
        37 & qwen1.5-110b-chat & $1161_{-5.0}^{+4.9} $ & $\phantom{-} 12_{-11.0}^{+4.9} $ & $\phantom{-} \phantom{0}58_{-10.5}^{+11.1} $ & $\phantom{-} 10_{-7.2}^{+10.8} $ & $\phantom{-} 11_{-7.8}^{+12.5} $ \\
        38 & gpt-3.5-turbo-0613 & $1161_{-6.3}^{+6.2} $ & $-41_{-11.3}^{+4.9} $ & $-\phantom{0}37_{-14.5}^{+16.2} $ & $\phantom{-} 13_{-6.0}^{+10.5} $ & $\phantom{-} 21_{-7.9}^{+12.1} $ \\
        39 & claude-2.1 & $1156_{-5.7}^{+6.3} $ & $-40_{-11.6}^{+5.3} $ & $-\phantom{0}45_{-11.8}^{+12.2} $ & $\phantom{-} 10_{-5.3}^{+10.8} $ & $\phantom{-} 22_{-6.9}^{+11.8} $ \\
        40 & mistral-next & $1153_{-10.6}^{+11.0} $ & $-20_{-15.2}^{+9.7} $ & $-\phantom{0}50_{-19.4}^{+20.2} $ & $\phantom{-} 14_{-10.4}^{+14.9} $ & $\phantom{-} \phantom{0}8_{-13.2}^{+17.7} $ \\
        41 & mistral-medium & $1153_{-6.0}^{+6.1} $ & $\phantom{-} \phantom{0}9_{-11.4}^{+5.2} $ & $-\phantom{0}24_{-10.7}^{+11.1} $ & $\phantom{-} \phantom{0}5_{-5.8}^{+11.4} $ & $\phantom{-} 11_{-7.2}^{+13.2} $ \\
        42 & mixtral-8x22b-instruct-v0.1 & $1152_{-4.5}^{+4.9} $ & $\phantom{-} \phantom{0}5_{-10.3}^{+4.3} $ & $-\phantom{00}7_{-9.0}^{+8.6} $ & $\phantom{-} 12_{-4.6}^{+10.3} $ & $\phantom{-} \phantom{0}8_{-5.9}^{+10.9} $ \\
        43 & llama-3-8b-instruct & $1150_{-3.4}^{+3.5} $ & $\phantom{-} 48_{-9.3}^{+3.3} $ & $-\phantom{0}41_{-6.0}^{+6.9} $ & $-16_{-3.4}^{+8.5} $ & $-\phantom{0}4_{-4.1}^{+8.7} $ \\
        44 & glm-4-0116 & $1149_{-10.7}^{+9.2} $ & $\phantom{-} 45_{-15.8}^{+10.5} $ & $\phantom{-} \phantom{0}76_{-18.7}^{+19.5} $ & $\phantom{-} 21_{-11.6}^{+17.4} $ & $\phantom{-} 12_{-14.0}^{+18.5} $ \\
        45 & qwen1.5-72b-chat & $1148_{-4.6}^{+5.4} $ & $\phantom{-} 11_{-10.6}^{+4.7} $ & $\phantom{-} \phantom{0}58_{-9.2}^{+9.0} $ & $-\phantom{0}1_{-4.7}^{+10.2} $ & $\phantom{-} 19_{-6.3}^{+11.5} $ \\
        46 & gpt-3.5-turbo-0125 & $1147_{-3.8}^{+4.1} $ & $-38_{-10.1}^{+3.5} $ & $-\phantom{0}46_{-7.1}^{+7.3} $ & $\phantom{-} 11_{-4.4}^{+9.2} $ & $\phantom{-} 19_{-4.5}^{+10.2} $ \\
        47 & zephyr-orpo-141b-A35b-v0.1 & $1143_{-12.2}^{+11.7} $ & $\phantom{-} \phantom{0}4_{-19.4}^{+12.2} $ & $-\phantom{0}27_{-22.2}^{+21.3} $ & $-\phantom{0}2_{-16.2}^{+21.5} $ & $-\phantom{0}1_{-18.9}^{+22.5} $ \\
        48 & gemini-pro & $1139_{-14.6}^{+14.4} $ & $-\phantom{0}7_{-20.4}^{+14.6} $ & $\phantom{-} \phantom{00}2_{-29.5}^{+29.9} $ & $-23_{-14.0}^{+18.7} $ & $-\phantom{0}7_{-17.3}^{+22.2} $ \\
        49 & claude-instant-1 & $1134_{-8.7}^{+8.1} $ & $-13_{-14.0}^{+8.1} $ & $-\phantom{0}15_{-19.0}^{+18.8} $ & $\phantom{-} \phantom{0}7_{-7.8}^{+13.3} $ & $\phantom{-} \phantom{0}3_{-10.7}^{+14.7} $ \\
        50 & wizardlm-70b & $1129_{-13.0}^{+12.7} $ & $\phantom{-} \phantom{0}5_{-17.3}^{+12.8} $ & $-\phantom{0}30_{-28.0}^{+30.0} $ & $-19_{-13.6}^{+17.7} $ & $-26_{-16.3}^{+20.1} $ \\
        51 & snowflake-arctic-instruct & $1126_{-5.0}^{+5.3} $ & $-13_{-11.1}^{+5.2} $ & $-\phantom{00}3_{-9.4}^{+9.8} $ & $-13_{-5.7}^{+10.7} $ & $-11_{-6.7}^{+12.1} $ \\
        52 & qwen1.5-32b-chat & $1126_{-6.0}^{+5.8} $ & $\phantom{-} \phantom{0}5_{-11.7}^{+5.8} $ & $\phantom{-} \phantom{0}69_{-10.4}^{+11.1} $ & $\phantom{-} \phantom{0}8_{-7.1}^{+11.7} $ & $\phantom{-} 22_{-8.9}^{+13.3} $ \\
        53 & yi-1.5-34b-chat & $1126_{-5.9}^{+6.4} $ & $\phantom{-} 63_{-12.2}^{+6.9} $ & $\phantom{-} 103_{-11.4}^{+12.1} $ & $\phantom{-} \phantom{0}5_{-7.6}^{+12.6} $ & $\phantom{-} \phantom{0}1_{-8.9}^{+13.5} $ \\
        54 & phi-3-medium-4k-instruct & $1126_{-7.4}^{+7.3} $ & $\phantom{-} 12_{-13.8}^{+7.9} $ & $-\phantom{00}7_{-13.0}^{+13.0} $ & $\phantom{-} 21_{-8.6}^{+13.5} $ & $\phantom{-} \phantom{0}5_{-11.1}^{+15.2} $ \\
        55 & tulu-2-dpo-70b & $1122_{-13.7}^{+13.4} $ & $-\phantom{0}4_{-19.0}^{+12.4} $ & $-\phantom{0}72_{-28.7}^{+29.7} $ & $\phantom{-} \phantom{0}8_{-12.9}^{+18.6} $ & $-\phantom{0}6_{-16.3}^{+21.1} $ \\
        56 & mixtral-8x7b-instruct-v0.1 & $1114_{-3.8}^{+4.1} $ & $\phantom{-} 25_{-10.2}^{+3.4} $ & $-\phantom{0}37_{-6.9}^{+7.4} $ & $\phantom{-} 10_{-4.0}^{+9.3} $ & $-\phantom{0}4_{-4.8}^{+10.2} $ \\
        57 & openchat-3.5-0106 & $1114_{-8.4}^{+8.7} $ & $-\phantom{0}3_{-14.5}^{+8.5} $ & $-\phantom{00}3_{-14.4}^{+17.0} $ & $-11_{-9.4}^{+14.0} $ & $\phantom{-} 17_{-11.5}^{+15.9} $ \\
        58 & qwen1.5-14b-chat & $1112_{-6.5}^{+6.4} $ & $\phantom{-} 10_{-12.5}^{+6.6} $ & $\phantom{-} \phantom{0}57_{-10.3}^{+11.2} $ & $\phantom{-} \phantom{0}8_{-8.1}^{+12.4} $ & $\phantom{-} 11_{-9.0}^{+14.2} $ \\
        59 & llama2-70b-steerlm-chat & $1111_{-20.2}^{+20.6} $ & $-\phantom{0}3_{-25.7}^{+19.4} $ & $-\phantom{0}28_{-33.8}^{+36.7} $ & $-13_{-19.7}^{+25.0} $ & $-52_{-21.6}^{+25.8} $ \\
        60 & starling-lm-7b-beta & $1111_{-7.1}^{+7.7} $ & $\phantom{-} 19_{-14.1}^{+7.6} $ & $\phantom{-} \phantom{0}35_{-11.3}^{+12.7} $ & $\phantom{-} \phantom{0}1_{-7.7}^{+13.0} $ & $\phantom{-} 18_{-10.5}^{+13.7} $ \\
        61 & llama-2-70b-chat & $1108_{-4.9}^{+5.8} $ & $\phantom{-} 24_{-10.3}^{+4.7} $ & $-\phantom{0}78_{-10.4}^{+10.8} $ & $-18_{-5.8}^{+10.3} $ & $-15_{-7.0}^{+11.1} $ \\
        62 & gpt-3.5-turbo-1106 & $1106_{-8.8}^{+8.7} $ & $-36_{-14.7}^{+8.6} $ & $-\phantom{0}62_{-21.8}^{+22.6} $ & $\phantom{-} 33_{-8.4}^{+14.7} $ & $\phantom{-} 20_{-11.5}^{+15.3} $ \\
        63 & vicuna-33b & $1105_{-7.9}^{+8.2} $ & $\phantom{-} 17_{-12.9}^{+6.6} $ & $-\phantom{0}27_{-14.4}^{+16.3} $ & $-18_{-7.8}^{+12.6} $ & $-18_{-8.9}^{+14.1} $ \\
        64 & phi-3-small-8k-instruct & $1103_{-6.7}^{+7.0} $ & $\phantom{-} 27_{-12.6}^{+7.6} $ & $-\phantom{0}16_{-12.0}^{+12.9} $ & $\phantom{-} 13_{-8.0}^{+13.5} $ & $-\phantom{0}5_{-9.4}^{+15.1} $ \\
        65 & openchat-3.5 & $1101_{-12.9}^{+13.2} $ & $-\phantom{0}5_{-18.3}^{+12.1} $ & $\phantom{-} \phantom{00}2_{-28.3}^{+26.4} $ & $\phantom{-} \phantom{0}2_{-11.6}^{+17.2} $ & $-23_{-16.2}^{+20.5} $ \\
        66 & dbrx-instruct-preview & $1101_{-5.3}^{+5.3} $ & $\phantom{-} 25_{-10.8}^{+4.9} $ & $-\phantom{00}4_{-9.4}^{+9.6} $ & $\phantom{-} \phantom{0}5_{-5.4}^{+10.5} $ & $\phantom{-} 17_{-6.8}^{+12.4} $ \\
        67 & yi-34b-chat & $1101_{-7.9}^{+8.1} $ & $\phantom{-} 36_{-14.4}^{+7.5} $ & $\phantom{-} \phantom{0}94_{-16.5}^{+16.5} $ & $-\phantom{0}6_{-9.8}^{+14.0} $ & $-\phantom{0}6_{-10.0}^{+14.5} $ \\
        68 & starling-lm-7b-alpha & $1099_{-10.4}^{+11.0} $ & $\phantom{-} 17_{-15.8}^{+10.5} $ & $-\phantom{0}17_{-19.9}^{+20.0} $ & $-12_{-11.9}^{+16.3} $ & $-\phantom{0}3_{-12.6}^{+18.1} $ \\
        69 & gemma-1.1-7b-it & $1097_{-6.0}^{+6.0} $ & $\phantom{-} 14_{-11.4}^{+5.9} $ & $-\phantom{00}2_{-10.2}^{+10.4} $ & $-\phantom{0}9_{-6.5}^{+12.2} $ & $\phantom{-} \phantom{0}3_{-8.5}^{+12.7} $ \\
        70 & pplx-70b-online & $1095_{-15.4}^{+12.8} $ & $\phantom{-} 11_{-19.4}^{+15.2} $ & $\phantom{-} \phantom{0}13_{-29.1}^{+31.4} $ & $-39_{-13.8}^{+20.3} $ & $-32_{-16.0}^{+19.9} $ \\
        71 & deepseek-llm-67b-chat & $1092_{-17.2}^{+15.8} $ & $\phantom{-} \phantom{0}0_{-21.6}^{+16.4} $ & $\phantom{-} \phantom{0}46_{-30.4}^{+34.4} $ & $-10_{-16.0}^{+23.9} $ & $\phantom{-} 10_{-20.2}^{+22.9} $ \\
        72 & nous-hermes-2-mixtral-8x7b-dpo & $1090_{-18.6}^{+20.2} $ & $\phantom{-} 25_{-24.8}^{+18.3} $ & $-\phantom{0}26_{-37.1}^{+35.4} $ & $-42_{-16.5}^{+21.5} $ & $\phantom{-} 17_{-21.5}^{+23.0} $ \\
        73 & qwen1.5-7b-chat & $1086_{-13.7}^{+13.4} $ & $-\phantom{0}4_{-19.7}^{+13.7} $ & $\phantom{-} \phantom{0}72_{-22.7}^{+26.1} $ & $-\phantom{0}8_{-15.3}^{+19.6} $ & $\phantom{-} 24_{-18.0}^{+22.5} $ \\
        74 & wizardlm-13b & $1083_{-14.1}^{+14.8} $ & $\phantom{-} \phantom{0}5_{-19.6}^{+12.4} $ & $-\phantom{0}10_{-27.5}^{+26.1} $ & $-41_{-15.9}^{+19.6} $ & $-13_{-19.1}^{+23.0} $ \\
        75 & llama-2-13b-chat & $1081_{-7.9}^{+7.3} $ & $\phantom{-} 12_{-12.7}^{+7.3} $ & $-\phantom{0}58_{-15.9}^{+17.3} $ & $-10_{-7.7}^{+12.9} $ & $-\phantom{0}9_{-10.4}^{+15.0} $ \\
        76 & qwen-14b-chat & $1081_{-16.1}^{+15.3} $ & $-35_{-20.3}^{+16.2} $ & $\phantom{-} \phantom{0}11_{-31.7}^{+35.3} $ & $-17_{-17.9}^{+22.0} $ & $\phantom{-} 33_{-20.4}^{+25.2} $ \\
        77 & vicuna-13b & $1077_{-8.9}^{+8.7} $ & $-15_{-12.9}^{+8.2} $ & $\phantom{-} \phantom{00}7_{-16.9}^{+16.5} $ & $-15_{-9.1}^{+13.8} $ & $\phantom{-} \phantom{0}1_{-10.7}^{+15.2} $ \\
        78 & openhermes-2.5-mistral-7b & $1075_{-14.8}^{+15.1} $ & $\phantom{-} 28_{-20.9}^{+14.7} $ & $-\phantom{0}13_{-29.5}^{+31.0} $ & $\phantom{-} \phantom{0}3_{-16.8}^{+19.7} $ & $-17_{-18.4}^{+23.8} $ \\
        79 & phi-3-mini-128k-instruct & $1072_{-6.3}^{+6.2} $ & $\phantom{-} \phantom{0}0_{-11.9}^{+6.4} $ & $-\phantom{00}2_{-11.6}^{+12.1} $ & $\phantom{-} \phantom{0}0_{-6.9}^{+12.7} $ & $-23_{-8.7}^{+13.4} $ \\
        80 & codellama-34b-instruct & $1070_{-13.1}^{+12.0} $ & $-\phantom{0}5_{-19.1}^{+12.3} $ & $-\phantom{0}57_{-30.6}^{+29.8} $ & $-13_{-13.2}^{+19.3} $ & $\phantom{-} \phantom{0}5_{-17.3}^{+22.4} $ \\
        81 & phi-3-mini-4k-instruct & $1068_{-5.7}^{+6.2} $ & $\phantom{-} 28_{-12.5}^{+6.2} $ & $-\phantom{0}24_{-13.0}^{+13.5} $ & $\phantom{-} 15_{-7.5}^{+12.2} $ & $\phantom{-} 10_{-8.0}^{+13.5} $ \\
        82 & solar-10.7b-instruct-v1.0 & $1064_{-17.8}^{+18.2} $ & $\phantom{-} 27_{-22.0}^{+17.9} $ & $-\phantom{0}23_{-33.3}^{+33.4} $ & $\phantom{-} \phantom{0}2_{-17.3}^{+22.4} $ & $-15_{-21.3}^{+27.7} $ \\
        83 & dolphin-2.2.1-mistral-7b & $1060_{-24.5}^{+25.1} $ & $\phantom{-} 30_{-29.4}^{+24.6} $ & $\phantom{-} \phantom{0}15_{-37.3}^{+37.1} $ & $\phantom{-} \phantom{0}0_{-23.2}^{+29.8} $ & $-31_{-28.0}^{+33.5} $ \\
        84 & vicuna-7b & $1058_{-16.7}^{+16.1} $ & $-36_{-21.5}^{+15.7} $ & $-\phantom{0}37_{-27.6}^{+28.8} $ & $-\phantom{0}3_{-14.6}^{+19.3} $ & $-18_{-18.8}^{+21.4} $ \\
        85 & falcon-180b-chat & $1056_{-29.4}^{+29.7} $ & $\phantom{-} \phantom{0}3_{-34.2}^{+26.8} $ & $-\phantom{0}22_{-34.5}^{+35.1} $ & $-25_{-28.4}^{+32.1} $ & $-\phantom{0}4_{-34.0}^{+40.6} $ \\
        86 & mistral-7b-instruct-v0.2 & $1054_{-7.4}^{+7.9} $ & $\phantom{-} 55_{-12.6}^{+7.4} $ & $-\phantom{00}6_{-12.7}^{+14.3} $ & $-\phantom{0}3_{-8.3}^{+12.4} $ & $\phantom{-} \phantom{0}0_{-9.0}^{+14.1} $ \\
        87 & zephyr-7b-alpha & $1051_{-26.8}^{+24.4} $ & $\phantom{-} 22_{-28.7}^{+26.7} $ & $-\phantom{0}14_{-37.1}^{+39.1} $ & $-18_{-25.8}^{+34.8} $ & $-\phantom{0}2_{-30.5}^{+33.6} $ \\
        88 & zephyr-7b-beta & $1049_{-11.0}^{+11.4} $ & $\phantom{-} 39_{-16.5}^{+10.7} $ & $-\phantom{0}42_{-24.8}^{+25.7} $ & $-22_{-11.5}^{+15.8} $ & $-13_{-12.9}^{+18.7} $ \\
        89 & gemma-1.1-2b-it & $1044_{-8.6}^{+9.0} $ & $\phantom{-} \phantom{0}2_{-15.2}^{+8.4} $ & $\phantom{-} \phantom{00}9_{-16.0}^{+16.3} $ & $-19_{-11.0}^{+16.0} $ & $\phantom{-} 25_{-12.3}^{+16.4} $ \\
        90 & mpt-30b-chat & $1041_{-21.3}^{+20.5} $ & $\phantom{-} 31_{-27.2}^{+20.8} $ & $-\phantom{0}14_{-37.3}^{+38.9} $ & $\phantom{-} 12_{-22.5}^{+29.1} $ & $-20_{-30.0}^{+31.8} $ \\
        91 & codellama-70b-instruct & $1039_{-23.2}^{+24.2} $ & $\phantom{-} 29_{-30.3}^{+26.1} $ & $\phantom{-} \phantom{0}25_{-34.2}^{+36.5} $ & $\phantom{-} \phantom{0}8_{-28.6}^{+33.3} $ & $-\phantom{0}1_{-28.9}^{+36.0} $ \\
        92 & pplx-7b-online & $1038_{-14.6}^{+15.2} $ & $\phantom{-} 35_{-21.0}^{+15.6} $ & $\phantom{-} \phantom{0}21_{-27.8}^{+32.7} $ & $-17_{-15.4}^{+21.6} $ & $-21_{-18.3}^{+22.7} $ \\
        93 & llama-2-7b-chat & $1036_{-8.6}^{+9.3} $ & $\phantom{-} 45_{-15.3}^{+7.9} $ & $-\phantom{0}28_{-19.2}^{+19.0} $ & $-22_{-9.6}^{+14.4} $ & $-31_{-12.3}^{+16.4} $ \\
        94 & guanaco-33b & $1035_{-21.6}^{+20.7} $ & $\phantom{-} 30_{-25.9}^{+21.7} $ & $-\phantom{0}17_{-31.7}^{+33.1} $ & $-12_{-21.4}^{+25.7} $ & $-53_{-27.0}^{+28.1} $ \\
        95 & gemma-7b-it & $1029_{-11.0}^{+11.3} $ & $\phantom{-} 28_{-16.5}^{+10.3} $ & $\phantom{-} \phantom{0}38_{-16.5}^{+18.7} $ & $\phantom{-} 11_{-11.6}^{+17.5} $ & $\phantom{-} \phantom{0}7_{-13.6}^{+16.7} $ \\
        96 & stripedhyena-nous-7b & $1028_{-13.6}^{+15.3} $ & $\phantom{-} 21_{-20.5}^{+14.1} $ & $-\phantom{0}16_{-32.9}^{+35.2} $ & $-19_{-16.2}^{+19.2} $ & $-10_{-18.6}^{+24.2} $ \\
        97 & qwen1.5-4b-chat & $1026_{-10.7}^{+13.0} $ & $-23_{-18.2}^{+11.9} $ & $\phantom{-} \phantom{0}36_{-19.0}^{+19.6} $ & $-13_{-13.2}^{+17.2} $ & $\phantom{-} \phantom{0}4_{-15.4}^{+19.3} $ \\
        98 & mistral-7b-instruct & $1008_{-12.6}^{+11.9} $ & $\phantom{-} 32_{-18.0}^{+11.5} $ & $-\phantom{0}26_{-27.6}^{+26.9} $ & $-\phantom{0}4_{-11.6}^{+18.1} $ & $\phantom{-} \phantom{0}0_{-16.8}^{+19.2} $ \\
        99 & palm-2 & $\phantom{0}997_{-14.4}^{+14.6} $ & $\phantom{-} 43_{-18.9}^{+14.4} $ & $-\phantom{0}69_{-29.6}^{+29.4} $ & $\phantom{-} \phantom{0}0_{-13.2}^{+17.9} $ & $-18_{-16.6}^{+21.7} $ \\
        100 & gemma-2b-it & $\phantom{0}995_{-14.7}^{+13.9} $ & $\phantom{-} 20_{-20.9}^{+15.2} $ & $\phantom{-} \phantom{0}33_{-24.6}^{+26.1} $ & $-\phantom{0}7_{-17.1}^{+19.9} $ & $\phantom{-} \phantom{0}7_{-19.7}^{+25.0} $ \\
        101 & olmo-7b-instruct & $\phantom{0}995_{-13.3}^{+13.4} $ & $\phantom{-} 59_{-18.3}^{+12.6} $ & $\phantom{-} \phantom{0}54_{-21.8}^{+23.7} $ & $-30_{-14.0}^{+18.8} $ & $\phantom{-} \phantom{0}8_{-18.7}^{+21.9} $ \\
        102 & RWKV-4-Raven-14B & $\phantom{0}971_{-19.5}^{+17.6} $ & $-30_{-23.4}^{+17.5} $ & $-\phantom{0}28_{-29.6}^{+30.0} $ & $-23_{-17.6}^{+23.6} $ & $-\phantom{0}7_{-21.3}^{+24.5} $ \\
        103 & koala-13b & $\phantom{0}967_{-17.4}^{+16.6} $ & $\phantom{-} 31_{-22.0}^{+16.6} $ & $-\phantom{0}44_{-24.0}^{+25.5} $ & $-36_{-15.0}^{+19.5} $ & $-\phantom{0}5_{-18.9}^{+21.8} $ \\
        104 & alpaca-13b & $\phantom{0}955_{-17.7}^{+19.8} $ & $-11_{-24.9}^{+18.2} $ & $-\phantom{0}96_{-28.4}^{+28.1} $ & $-62_{-15.3}^{+21.3} $ & $-78_{-21.8}^{+27.9} $ \\
        105 & chatglm3-6b & $\phantom{0}946_{-17.0}^{+16.3} $ & $\phantom{-} 33_{-22.0}^{+17.3} $ & $\phantom{-} 113_{-32.1}^{+30.0} $ & $\phantom{-} \phantom{0}4_{-17.8}^{+21.8} $ & $-\phantom{0}7_{-21.6}^{+25.3} $ \\
        106 & mpt-7b-chat & $\phantom{0}944_{-20.3}^{+20.8} $ & $\phantom{-} \phantom{0}8_{-25.7}^{+20.6} $ & $\phantom{-} \phantom{0}37_{-30.1}^{+30.5} $ & $-25_{-22.6}^{+24.7} $ & $-\phantom{0}7_{-26.0}^{+31.2} $ \\
        107 & chatglm2-6b & $\phantom{0}930_{-19.2}^{+20.7} $ & $\phantom{-} 30_{-25.2}^{+21.2} $ & $\phantom{-} \phantom{0}67_{-37.8}^{+42.2} $ & $-\phantom{0}2_{-24.8}^{+30.3} $ & $-38_{-27.1}^{+31.0} $ \\
        108 & gpt4all-13b-snoozy & $\phantom{0}924_{-27.3}^{+25.1} $ & $\phantom{-} 39_{-29.2}^{+26.6} $ & $-\phantom{00}8_{-31.9}^{+31.0} $ & $\phantom{-} 10_{-24.2}^{+28.9} $ & $-21_{-32.2}^{+33.1} $ \\
        109 & oasst-pythia-12b & $\phantom{0}912_{-18.1}^{+17.6} $ & $\phantom{-} 10_{-21.2}^{+16.6} $ & $-\phantom{0}63_{-25.1}^{+26.3} $ & $-\phantom{0}4_{-18.4}^{+21.3} $ & $-12_{-20.0}^{+26.1} $ \\
        110 & fastchat-t5-3b & $\phantom{0}879_{-19.6}^{+20.8} $ & $\phantom{-} 42_{-24.8}^{+18.6} $ & $-108_{-26.6}^{+28.6} $ & $-36_{-18.6}^{+23.6} $ & $-90_{-24.5}^{+28.8} $ \\
        111 & chatglm-6b & $\phantom{0}874_{-19.1}^{+19.3} $ & $\phantom{-} 11_{-24.3}^{+18.1} $ & $\phantom{-} 199_{-28.7}^{+29.8} $ & $\phantom{-} 18_{-19.5}^{+22.4} $ & $\phantom{-} 11_{-23.1}^{+24.4} $ \\
        112 & dolly-v2-12b & $\phantom{0}856_{-24.2}^{+22.7} $ & $-15_{-27.6}^{+21.9} $ & $\phantom{-} \phantom{00}8_{-30.9}^{+31.1} $ & $\phantom{-} \phantom{0}4_{-22.0}^{+26.2} $ & $-58_{-24.2}^{+30.8} $ \\
        113 & llama-13b & $\phantom{0}853_{-25.8}^{+24.0} $ & $-26_{-28.6}^{+24.4} $ & $-\phantom{00}8_{-27.7}^{+33.2} $ & $-36_{-27.0}^{+28.9} $ & $-89_{-25.1}^{+32.6} $ \\
        114 & stablelm-tuned-alpha-7b & $\phantom{0}843_{-22.2}^{+19.6} $ & $\phantom{-} 19_{-24.7}^{+22.2} $ & $\phantom{-} \phantom{0}30_{-28.5}^{+29.1} $ & $-13_{-20.5}^{+24.0} $ & $\phantom{-} 32_{-23.9}^{+27.9} $ \\
    
    \end{longtable}
    }
    
    \end{footnotesize}

\begin{footnotesize}
    {
    
\begin{longtable}[t]{lllllll}
    \caption{Leaderboard of human evaluation with modifiers when all fitted separately using a unidimensional approach. For the four tasks, modifiers are shown to indicate the deviation from the main rating to make comparison with \tool easier. Indicated deviations are $95\%$ confidence intervals determined using bootstrapping.} \label{tab:leaderboard-single} \\
    
    \toprule
    Rank & Model Name & Rating & English & Chinese & Hardness & Code \\
    \midrule
    \endfirsthead

    \caption[]{(continued)} \\
    \toprule
    Rank & Model Name & Rating & English & Chinese & Hardness & Code \\
    \midrule
    \endhead

    \bottomrule
    \endfoot

    \bottomrule
    \endlastfoot

    1 & gpt-4o-2024-05-13 & $1283_{-2.8}^{+2.7} $ & $-19_{-4.4}^{+4.3} $ & $\phantom{-} \phantom{0}52_{-9.2}^{+9.0} $ & $\phantom{-} \phantom{0}5_{-5.4}^{+5.6} $ & $\phantom{-} 13_{-6.7}^{+6.3} $ \\
2 & claude-3-5-sonnet-20240620 & $1267_{-4.2}^{+4.1} $ & $-23_{-6.9}^{+6.9} $ & $\phantom{-} \phantom{0}45_{-12.1}^{+12.1} $ & $\phantom{-} 11_{-8.8}^{+8.5} $ & $\phantom{-} 35_{-10.0}^{+9.1} $ \\
3 & gemini-advanced-0514 & $1261_{-2.9}^{+2.8} $ & $-28_{-5.1}^{+4.8} $ & $\phantom{-} \phantom{0}69_{-8.9}^{+8.7} $ & $-\phantom{0}8_{-6.1}^{+6.2} $ & $-\phantom{0}4_{-7.5}^{+7.0} $ \\
4 & gemini-1.5-pro-api-0514 & $1259_{-2.9}^{+2.7} $ & $-25_{-4.9}^{+4.8} $ & $\phantom{-} \phantom{0}76_{-8.7}^{+8.5} $ & $\phantom{-} \phantom{0}5_{-5.8}^{+6.1} $ & $\phantom{-} \phantom{0}8_{-7.0}^{+6.8} $ \\
5 & gpt-4-turbo-2024-04-09 & $1252_{-2.3}^{+2.3} $ & $-12_{-4.0}^{+3.7} $ & $\phantom{-} \phantom{0}50_{-7.1}^{+7.4} $ & $\phantom{-} \phantom{0}5_{-4.7}^{+5.1} $ & $\phantom{-} 14_{-5.8}^{+6.0} $ \\
6 & gpt-4-1106-preview & $1248_{-2.3}^{+2.3} $ & $-17_{-3.9}^{+3.4} $ & $\phantom{-} \phantom{0}52_{-7.9}^{+7.5} $ & $\phantom{-} \phantom{0}0_{-5.2}^{+4.9} $ & $\phantom{-} \phantom{0}8_{-5.9}^{+5.6} $ \\
7 & gemini-1.5-pro-api-0409-preview & $1247_{-2.6}^{+2.6} $ & $-16_{-4.0}^{+4.3} $ & $\phantom{-} \phantom{0}55_{-8.5}^{+8.3} $ & $-15_{-5.8}^{+5.5} $ & $-15_{-6.0}^{+6.3} $ \\
8 & claude-3-opus-20240229 & $1245_{-2.1}^{+2.1} $ & $-31_{-3.4}^{+3.4} $ & $\phantom{-} \phantom{0}70_{-6.6}^{+6.6} $ & $\phantom{-} \phantom{0}3_{-4.3}^{+4.3} $ & $\phantom{-} \phantom{0}6_{-5.3}^{+5.1} $ \\
9 & gpt-4-0125-preview & $1243_{-2.4}^{+2.2} $ & $-16_{-3.6}^{+3.7} $ & $\phantom{-} \phantom{0}53_{-7.4}^{+7.2} $ & $\phantom{-} \phantom{0}2_{-5.0}^{+5.1} $ & $\phantom{-} \phantom{0}3_{-6.2}^{+6.0} $ \\
10 & yi-large-preview & $1233_{-2.8}^{+2.8} $ & $-19_{-4.4}^{+4.7} $ & $\phantom{-} \phantom{0}84_{-8.8}^{+8.9} $ & $\phantom{-} \phantom{0}7_{-6.0}^{+6.1} $ & $\phantom{-} 11_{-7.1}^{+6.7} $ \\
11 & gemini-1.5-flash-api-0514 & $1226_{-3.0}^{+3.0} $ & $-25_{-4.7}^{+5.0} $ & $\phantom{-} \phantom{0}66_{-9.3}^{+9.4} $ & $\phantom{-} \phantom{0}1_{-6.3}^{+6.0} $ & $\phantom{-} \phantom{0}9_{-7.3}^{+7.3} $ \\
12 & yi-large & $1215_{-4.5}^{+4.4} $ & $-16_{-8.2}^{+8.3} $ & $\phantom{-} \phantom{0}58_{-15.1}^{+15.3} $ & $\phantom{-} \phantom{0}6_{-10.2}^{+10.2} $ & $\phantom{-} 18_{-11.9}^{+11.9} $ \\
13 & gemma-2-27b-it & $1210_{-6.0}^{+5.9} $ & $-20_{-11.0}^{+10.1} $ & $\phantom{-} \phantom{0}54_{-20.1}^{+20.1} $ & $-18_{-12.5}^{+11.7} $ & $-\phantom{0}5_{-14.0}^{+14.6} $ \\
14 & bard-jan-24-gemini-pro & $1207_{-4.5}^{+4.7} $ & $-25_{-7.0}^{+7.0} $ & $\phantom{-} \phantom{0}59_{-22.5}^{+24.1} $ & $-51_{-10.6}^{+10.6} $ & $-35_{-13.3}^{+13.1} $ \\
15 & glm-4-0520 & $1206_{-5.1}^{+5.0} $ & $-15_{-8.7}^{+8.2} $ & $\phantom{-} \phantom{0}90_{-16.0}^{+17.2} $ & $\phantom{-} 10_{-10.9}^{+10.7} $ & $\phantom{-} 13_{-12.4}^{+12.7} $ \\
16 & nemotron-4-340b-instruct & $1204_{-3.9}^{+3.6} $ & $-22_{-6.4}^{+6.4} $ & $\phantom{-} \phantom{0}62_{-12.4}^{+12.3} $ & $-\phantom{0}4_{-8.2}^{+8.3} $ & $-\phantom{0}7_{-9.9}^{+11.2} $ \\
17 & llama-3-70b-instruct & $1202_{-2.1}^{+2.1} $ & $\phantom{-} 22_{-3.4}^{+3.3} $ & $-\phantom{0}32_{-6.6}^{+6.5} $ & $-\phantom{0}5_{-4.5}^{+4.5} $ & $\phantom{-} \phantom{0}0_{-5.3}^{+5.3} $ \\
18 & claude-3-sonnet-20240229 & $1198_{-2.2}^{+2.2} $ & $-23_{-3.4}^{+3.5} $ & $\phantom{-} \phantom{0}48_{-6.6}^{+6.1} $ & $\phantom{-} \phantom{0}1_{-4.7}^{+4.4} $ & $\phantom{-} 17_{-5.1}^{+5.4} $ \\
19 & reka-core-20240501 & $1194_{-2.4}^{+2.4} $ & $-20_{-4.3}^{+4.0} $ & $\phantom{-} \phantom{0}63_{-8.5}^{+8.3} $ & $-\phantom{0}6_{-5.8}^{+5.2} $ & $-\phantom{0}4_{-5.9}^{+6.2} $ \\
20 & command-r-plus & $1188_{-2.3}^{+2.2} $ & $-25_{-3.7}^{+3.6} $ & $\phantom{-} \phantom{0}63_{-7.0}^{+6.9} $ & $-20_{-4.8}^{+5.1} $ & $-21_{-5.9}^{+5.9} $ \\
21 & gpt-4-0314 & $1188_{-2.6}^{+2.5} $ & $-23_{-4.1}^{+4.2} $ & $\phantom{-} \phantom{0}54_{-8.3}^{+8.3} $ & $\phantom{-} \phantom{0}9_{-5.6}^{+5.5} $ & $\phantom{-} 10_{-6.7}^{+6.5} $ \\
22 & qwen-max-0428 & $1185_{-2.9}^{+2.7} $ & $-17_{-4.9}^{+5.1} $ & $\phantom{-} 105_{-11.4}^{+11.3} $ & $\phantom{-} \phantom{0}3_{-7.1}^{+7.1} $ & $\phantom{-} \phantom{0}7_{-8.3}^{+7.8} $ \\
23 & qwen2-72b-instruct & $1184_{-3.2}^{+3.3} $ & $-17_{-5.3}^{+5.5} $ & $\phantom{-} 106_{-10.4}^{+10.6} $ & $\phantom{-} \phantom{0}1_{-6.9}^{+7.2} $ & $-\phantom{0}1_{-8.6}^{+8.6} $ \\
24 & claude-3-haiku-20240307 & $1181_{-2.2}^{+2.2} $ & $-23_{-3.8}^{+3.6} $ & $\phantom{-} \phantom{0}33_{-7.0}^{+6.4} $ & $\phantom{-} \phantom{0}1_{-4.6}^{+4.7} $ & $\phantom{-} 10_{-5.7}^{+5.6} $ \\
25 & gemma-2-9b-it & $1180_{-6.0}^{+6.0} $ & $-24_{-10.1}^{+10.5} $ & $\phantom{-} \phantom{0}56_{-19.5}^{+19.9} $ & $-10_{-13.3}^{+12.7} $ & $-17_{-15.1}^{+14.8} $ \\
26 & deepseek-coder-v2 & $1177_{-4.9}^{+4.6} $ & $-28_{-8.1}^{+8.3} $ & $\phantom{-} \phantom{0}80_{-16.2}^{+16.2} $ & $\phantom{-} 37_{-10.8}^{+10.3} $ & $\phantom{-} 61_{-11.8}^{+11.4} $ \\
27 & glm-4-0116 & $1173_{-5.3}^{+5.1} $ & $\phantom{-} \phantom{0}2_{-9.1}^{+9.0} $ & $\phantom{-} \phantom{0}99_{-17.9}^{+18.5} $ & $\phantom{-} 14_{-11.3}^{+10.6} $ & $\phantom{-} 19_{-13.0}^{+12.7} $ \\
28 & qwen1.5-110b-chat & $1165_{-3.1}^{+3.1} $ & $-13_{-5.1}^{+4.8} $ & $\phantom{-} \phantom{0}96_{-10.1}^{+10.4} $ & $\phantom{-} \phantom{0}4_{-6.4}^{+6.3} $ & $\phantom{-} 10_{-7.9}^{+8.1} $ \\
29 & gpt-4-0613 & $1165_{-2.4}^{+2.2} $ & $-18_{-3.8}^{+3.5} $ & $\phantom{-} \phantom{0}25_{-7.8}^{+7.6} $ & $\phantom{-} \phantom{0}3_{-5.0}^{+4.8} $ & $\phantom{-} \phantom{0}3_{-6.0}^{+5.7} $ \\
30 & reka-flash-preview-20240611 & $1164_{-4.1}^{+4.3} $ & $-22_{-7.7}^{+7.7} $ & $\phantom{-} \phantom{0}52_{-13.5}^{+13.4} $ & $-14_{-8.5}^{+8.6} $ & $-\phantom{0}3_{-9.8}^{+10.1} $ \\
31 & yi-1.5-34b-chat & $1158_{-3.4}^{+3.3} $ & $\phantom{-} \phantom{0}5_{-5.8}^{+5.7} $ & $\phantom{-} 110_{-11.1}^{+11.0} $ & $\phantom{-} \phantom{0}2_{-8.0}^{+7.0} $ & $\phantom{-} \phantom{0}6_{-9.0}^{+8.7} $ \\
32 & reka-flash-21b-20240226-online & $1155_{-3.7}^{+3.6} $ & $-19_{-6.7}^{+6.1} $ & $\phantom{-} \phantom{0}46_{-10.9}^{+11.0} $ & $-12_{-8.8}^{+8.5} $ & $-\phantom{0}6_{-8.9}^{+8.4} $ \\
33 & mistral-large-2402 & $1155_{-2.4}^{+2.5} $ & $-\phantom{0}9_{-4.2}^{+4.0} $ & $\phantom{-} \phantom{0}18_{-7.8}^{+7.9} $ & $\phantom{-} 10_{-5.3}^{+5.5} $ & $\phantom{-} 14_{-6.2}^{+6.2} $ \\
34 & llama-3-8b-instruct & $1154_{-2.3}^{+2.2} $ & $\phantom{-} 11_{-3.7}^{+3.6} $ & $-\phantom{0}15_{-6.8}^{+6.7} $ & $-16_{-4.6}^{+4.6} $ & $-\phantom{0}6_{-5.5}^{+5.8} $ \\
35 & qwen1.5-72b-chat & $1151_{-2.6}^{+2.4} $ & $-16_{-4.3}^{+4.3} $ & $\phantom{-} \phantom{0}94_{-9.1}^{+9.0} $ & $-\phantom{0}4_{-5.9}^{+5.8} $ & $\phantom{-} 11_{-7.4}^{+6.8} $ \\
36 & claude-1 & $1150_{-3.8}^{+3.7} $ & $-21_{-5.8}^{+5.8} $ & $\phantom{-} \phantom{0}49_{-13.7}^{+14.4} $ & $-25_{-8.5}^{+7.9} $ & $-12_{-10.4}^{+10.5} $ \\
37 & command-r & $1149_{-2.5}^{+2.5} $ & $-26_{-4.3}^{+4.2} $ & $\phantom{-} \phantom{0}66_{-7.5}^{+7.2} $ & $-30_{-5.6}^{+5.5} $ & $-23_{-6.0}^{+6.4} $ \\
38 & reka-flash-21b-20240226 & $1147_{-3.3}^{+3.1} $ & $-20_{-5.1}^{+5.1} $ & $\phantom{-} \phantom{0}46_{-9.9}^{+10.2} $ & $-13_{-6.3}^{+7.1} $ & $-\phantom{0}4_{-8.1}^{+7.3} $ \\
39 & mistral-medium & $1146_{-2.8}^{+2.9} $ & $-\phantom{0}9_{-4.9}^{+4.7} $ & $\phantom{-} \phantom{0}20_{-10.4}^{+9.9} $ & $-\phantom{0}1_{-6.3}^{+6.0} $ & $\phantom{-} \phantom{0}8_{-7.2}^{+7.6} $ \\
40 & mixtral-8x22b-instruct-v0.1 & $1146_{-2.7}^{+2.7} $ & $-10_{-4.2}^{+4.4} $ & $\phantom{-} \phantom{0}40_{-9.0}^{+8.5} $ & $\phantom{-} \phantom{0}3_{-6.2}^{+5.9} $ & $\phantom{-} \phantom{0}9_{-6.9}^{+6.4} $ \\
41 & gemini-pro-dev-api & $1136_{-3.7}^{+3.6} $ & $-26_{-5.8}^{+6.3} $ & $\phantom{-} \phantom{0}51_{-12.6}^{+12.6} $ & $-27_{-8.9}^{+8.8} $ & $-31_{-10.0}^{+10.0} $ \\
42 & claude-2.0 & $1133_{-4.5}^{+4.7} $ & $-19_{-6.8}^{+6.9} $ & $\phantom{-} \phantom{0}58_{-21.0}^{+21.8} $ & $-\phantom{0}5_{-10.1}^{+10.6} $ & $\phantom{-} \phantom{0}4_{-13.1}^{+13.5} $ \\
43 & qwen1.5-32b-chat & $1132_{-3.4}^{+3.3} $ & $-21_{-5.2}^{+5.5} $ & $\phantom{-} 104_{-9.8}^{+9.6} $ & $\phantom{-} \phantom{0}4_{-7.4}^{+7.5} $ & $\phantom{-} 16_{-8.7}^{+8.6} $ \\
44 & zephyr-orpo-141b-A35b-v0.1 & $1128_{-6.0}^{+6.3} $ & $-\phantom{0}9_{-10.6}^{+11.4} $ & $\phantom{-} \phantom{0}22_{-18.1}^{+18.8} $ & $-11_{-15.1}^{+14.5} $ & $-\phantom{0}5_{-17.2}^{+16.6} $ \\
45 & mistral-next & $1127_{-4.5}^{+4.5} $ & $-16_{-6.9}^{+6.5} $ & $\phantom{-} \phantom{0}12_{-17.8}^{+17.2} $ & $\phantom{-} \phantom{0}3_{-9.1}^{+9.8} $ & $\phantom{-} \phantom{0}7_{-11.8}^{+12.1} $ \\
46 & phi-3-medium-4k-instruct & $1125_{-4.1}^{+4.1} $ & $-\phantom{0}7_{-6.6}^{+7.0} $ & $\phantom{-} \phantom{0}36_{-11.9}^{+12.2} $ & $\phantom{-} \phantom{0}9_{-9.0}^{+8.8} $ & $\phantom{-} 10_{-9.2}^{+9.9} $ \\
47 & gpt-3.5-turbo-0613 & $1120_{-2.9}^{+2.9} $ & $-21_{-4.5}^{+4.5} $ & $\phantom{-} \phantom{0}40_{-13.3}^{+13.5} $ & $\phantom{-} \phantom{0}4_{-6.6}^{+6.8} $ & $\phantom{-} 16_{-8.3}^{+8.6} $ \\
48 & qwen1.5-14b-chat & $1119_{-3.7}^{+3.4} $ & $-19_{-6.1}^{+6.0} $ & $\phantom{-} \phantom{0}89_{-9.7}^{+9.8} $ & $\phantom{-} \phantom{0}1_{-7.4}^{+7.4} $ & $\phantom{-} \phantom{0}9_{-9.1}^{+8.8} $ \\
49 & starling-lm-7b-beta & $1119_{-4.0}^{+3.7} $ & $-12_{-6.3}^{+6.4} $ & $\phantom{-} \phantom{0}66_{-10.3}^{+10.5} $ & $-\phantom{0}1_{-8.1}^{+7.8} $ & $\phantom{-} 13_{-9.2}^{+9.1} $ \\
50 & claude-2.1 & $1118_{-2.9}^{+3.0} $ & $-22_{-4.5}^{+4.6} $ & $\phantom{-} \phantom{0}32_{-11.8}^{+10.9} $ & $\phantom{-} \phantom{0}2_{-6.5}^{+6.4} $ & $\phantom{-} 15_{-8.7}^{+8.0} $ \\
51 & yi-34b-chat & $1116_{-3.8}^{+3.9} $ & $-\phantom{0}9_{-6.3}^{+6.5} $ & $\phantom{-} 116_{-14.3}^{+14.7} $ & $-12_{-9.2}^{+8.8} $ & $-\phantom{0}9_{-10.7}^{+10.5} $ \\
52 & gemini-pro & $1115_{-6.1}^{+6.2} $ & $-16_{-9.4}^{+9.6} $ & $\phantom{-} \phantom{0}52_{-30.2}^{+29.4} $ & $-30_{-13.5}^{+14.4} $ & $-19_{-19.3}^{+17.3} $ \\
53 & mixtral-8x7b-instruct-v0.1 & $1114_{0.0}^{+0.0} $ & $\phantom{-} \phantom{0}0_{0.0}^{+0.0} $ & $\phantom{-} \phantom{00}0_{0.0}^{+0.0} $ & $\phantom{-} \phantom{0}0_{0.0}^{+0.0} $ & $\phantom{-} \phantom{0}0_{0.0}^{+0.0} $ \\
54 & gpt-3.5-turbo-0125 & $1113_{-2.2}^{+2.4} $ & $-24_{-4.0}^{+4.0} $ & $\phantom{-} \phantom{0}29_{-7.7}^{+7.6} $ & $\phantom{-} \phantom{0}1_{-5.1}^{+5.4} $ & $\phantom{-} 12_{-6.5}^{+6.1} $ \\
55 & claude-instant-1 & $1112_{-3.9}^{+3.9} $ & $-16_{-5.8}^{+6.1} $ & $\phantom{-} \phantom{0}38_{-17.2}^{+17.5} $ & $-\phantom{0}4_{-8.7}^{+8.7} $ & $-\phantom{0}2_{-10.8}^{+11.3} $ \\
56 & wizardlm-70b & $1110_{-5.6}^{+5.4} $ & $-11_{-8.7}^{+8.2} $ & $\phantom{-} \phantom{0}10_{-27.7}^{+27.5} $ & $-31_{-12.2}^{+12.9} $ & $-38_{-15.3}^{+15.7} $ \\
57 & gpt-3.5-turbo-0314 & $1110_{-7.2}^{+7.3} $ & $-26_{-11.8}^{+11.2} $ & $\phantom{-} \phantom{0}95_{-30.5}^{+30.4} $ & $\phantom{-} \phantom{0}9_{-20.6}^{+18.4} $ & $\phantom{-} \phantom{0}8_{-24.1}^{+24.3} $ \\
58 & dbrx-instruct-preview & $1106_{-3.1}^{+2.8} $ & $-\phantom{0}2_{-4.7}^{+4.7} $ & $\phantom{-} \phantom{0}30_{-8.5}^{+8.2} $ & $\phantom{-} \phantom{0}2_{-6.4}^{+6.2} $ & $\phantom{-} 15_{-7.4}^{+7.4} $ \\
59 & phi-3-small-8k-instruct & $1104_{-3.8}^{+3.9} $ & $\phantom{-} \phantom{0}2_{-6.7}^{+6.9} $ & $\phantom{-} \phantom{0}21_{-11.6}^{+11.7} $ & $\phantom{-} \phantom{0}3_{-8.1}^{+8.6} $ & $\phantom{-} \phantom{0}3_{-10.0}^{+9.4} $ \\
60 & tulu-2-dpo-70b & $1103_{-6.1}^{+6.2} $ & $-11_{-9.3}^{+8.5} $ & $-\phantom{0}33_{-31.3}^{+29.0} $ & $-\phantom{0}5_{-13.9}^{+14.3} $ & $-\phantom{0}8_{-18.0}^{+17.0} $ \\
61 & snowflake-arctic-instruct & $1099_{-2.8}^{+2.9} $ & $-20_{-4.6}^{+4.7} $ & $\phantom{-} \phantom{0}53_{-9.6}^{+9.2} $ & $-23_{-6.1}^{+6.2} $ & $-19_{-8.1}^{+7.3} $ \\
62 & openchat-3.5-0106 & $1099_{-4.1}^{+4.2} $ & $-15_{-6.7}^{+6.3} $ & $\phantom{-} \phantom{0}48_{-13.0}^{+14.0} $ & $-13_{-8.5}^{+8.7} $ & $\phantom{-} \phantom{0}6_{-11.4}^{+11.5} $ \\
63 & llama-2-70b-chat & $1097_{-2.8}^{+2.7} $ & $\phantom{-} \phantom{0}1_{-4.7}^{+4.4} $ & $-\phantom{0}39_{-9.4}^{+9.5} $ & $-25_{-5.8}^{+6.0} $ & $-22_{-7.7}^{+7.7} $ \\
64 & vicuna-33b & $1095_{-3.4}^{+3.6} $ & $-\phantom{0}7_{-5.5}^{+5.2} $ & $\phantom{-} \phantom{00}9_{-12.9}^{+13.1} $ & $-27_{-8.2}^{+7.8} $ & $-28_{-9.7}^{+9.8} $ \\
65 & starling-lm-7b-alpha & $1093_{-4.7}^{+4.9} $ & $-\phantom{0}7_{-7.8}^{+7.4} $ & $\phantom{-} \phantom{0}20_{-17.1}^{+17.5} $ & $-17_{-10.6}^{+10.8} $ & $-10_{-12.9}^{+12.6} $ \\
66 & gemma-1.1-7b-it & $1090_{-3.3}^{+3.3} $ & $-\phantom{0}8_{-5.4}^{+5.4} $ & $\phantom{-} \phantom{0}39_{-9.8}^{+9.9} $ & $-13_{-7.1}^{+7.2} $ & $-\phantom{0}3_{-8.0}^{+7.8} $ \\
67 & nous-hermes-2-mixtral-8x7b-dpo & $1087_{-6.8}^{+7.6} $ & $-\phantom{0}9_{-11.4}^{+11.4} $ & $-\phantom{00}9_{-48.2}^{+47.6} $ & $-35_{-15.5}^{+15.8} $ & $-\phantom{0}4_{-19.9}^{+18.7} $ \\
68 & llama2-70b-steerlm-chat & $1083_{-8.5}^{+7.9} $ & $-14_{-12.6}^{+12.9} $ & $\phantom{-} \phantom{0}14_{-35.5}^{+37.5} $ & $-35_{-20.0}^{+19.9} $ & $-59_{-23.0}^{+23.2} $ \\
69 & openchat-3.5 & $1080_{-5.3}^{+5.4} $ & $-14_{-8.7}^{+7.8} $ & $\phantom{-} \phantom{0}53_{-25.7}^{+26.8} $ & $-14_{-12.7}^{+12.1} $ & $-24_{-16.3}^{+15.4} $ \\
70 & deepseek-llm-67b-chat & $1080_{-7.0}^{+7.0} $ & $-15_{-10.8}^{+10.3} $ & $\phantom{-} 103_{-33.8}^{+34.8} $ & $-14_{-15.5}^{+15.3} $ & $\phantom{-} \phantom{0}2_{-19.7}^{+20.1} $ \\
71 & openhermes-2.5-mistral-7b & $1080_{-6.3}^{+6.4} $ & $-\phantom{0}6_{-9.9}^{+9.4} $ & $\phantom{-} \phantom{00}8_{-33.3}^{+34.6} $ & $-10_{-14.8}^{+15.1} $ & $-18_{-19.9}^{+20.2} $ \\
72 & qwen1.5-7b-chat & $1079_{-6.3}^{+6.3} $ & $-22_{-10.1}^{+10.1} $ & $\phantom{-} 122_{-23.3}^{+22.7} $ & $-10_{-13.7}^{+12.9} $ & $\phantom{-} 13_{-17.7}^{+18.0} $ \\
73 & pplx-70b-online & $1077_{-6.1}^{+5.9} $ & $-12_{-9.4}^{+9.2} $ & $\phantom{-} \phantom{0}54_{-30.5}^{+29.6} $ & $-49_{-13.7}^{+13.4} $ & $-49_{-15.5}^{+16.0} $ \\
74 & mistral-7b-instruct-v0.2 & $1075_{-3.5}^{+3.7} $ & $\phantom{-} \phantom{0}7_{-5.7}^{+5.7} $ & $\phantom{-} \phantom{00}8_{-10.7}^{+11.2} $ & $-\phantom{0}6_{-7.4}^{+7.9} $ & $\phantom{-} \phantom{0}0_{-9.6}^{+9.2} $ \\
75 & gpt-3.5-turbo-1106 & $1073_{-3.8}^{+3.9} $ & $-18_{-5.9}^{+6.2} $ & $\phantom{-} \phantom{0}10_{-19.0}^{+17.8} $ & $\phantom{-} 20_{-9.3}^{+9.0} $ & $\phantom{-} 25_{-10.3}^{+10.8} $ \\
76 & phi-3-mini-4k-instruct & $1072_{-3.7}^{+3.7} $ & $\phantom{-} \phantom{0}3_{-6.1}^{+6.1} $ & $\phantom{-} \phantom{0}12_{-11.5}^{+12.0} $ & $\phantom{-} \phantom{0}8_{-7.1}^{+7.1} $ & $\phantom{-} 16_{-8.7}^{+8.4} $ \\
77 & llama-2-13b-chat & $1068_{-3.8}^{+4.0} $ & $-\phantom{0}6_{-6.3}^{+5.8} $ & $-\phantom{0}17_{-15.4}^{+15.5} $ & $-19_{-8.7}^{+9.0} $ & $-16_{-10.8}^{+10.5} $ \\
78 & solar-10.7b-instruct-v1.0 & $1067_{-7.2}^{+7.2} $ & $-\phantom{0}5_{-11.1}^{+10.4} $ & $\phantom{-} \phantom{00}0_{-35.9}^{+37.2} $ & $-\phantom{0}9_{-16.7}^{+17.0} $ & $-16_{-21.1}^{+19.8} $ \\
79 & dolphin-2.2.1-mistral-7b & $1066_{-11.3}^{+11.4} $ & $-\phantom{0}5_{-17.2}^{+16.6} $ & $\phantom{-} \phantom{0}44_{-54.6}^{+56.3} $ & $-15_{-26.6}^{+27.3} $ & $-40_{-34.6}^{+34.2} $ \\
80 & wizardlm-13b & $1063_{-5.6}^{+6.0} $ & $-12_{-8.7}^{+8.9} $ & $\phantom{-} \phantom{0}28_{-26.0}^{+26.1} $ & $-49_{-14.3}^{+15.0} $ & $-37_{-17.3}^{+18.8} $ \\
81 & zephyr-7b-beta & $1057_{-5.0}^{+5.2} $ & $-\phantom{0}2_{-7.1}^{+7.6} $ & $-\phantom{0}31_{-24.3}^{+24.9} $ & $-29_{-11.5}^{+11.9} $ & $-24_{-13.8}^{+14.2} $ \\
82 & phi-3-mini-128k-instruct & $1054_{-3.4}^{+3.6} $ & $-15_{-5.4}^{+5.7} $ & $\phantom{-} \phantom{0}47_{-11.4}^{+11.1} $ & $-15_{-7.4}^{+7.6} $ & $-23_{-9.2}^{+8.7} $ \\
83 & vicuna-13b & $1050_{-3.9}^{+4.2} $ & $-19_{-6.2}^{+6.2} $ & $\phantom{-} \phantom{0}63_{-16.3}^{+15.5} $ & $-23_{-8.9}^{+9.2} $ & $-15_{-11.8}^{+11.6} $ \\
84 & mpt-30b-chat & $1050_{-9.4}^{+9.4} $ & $-\phantom{0}5_{-15.1}^{+14.0} $ & $-\phantom{00}3_{-48.3}^{+48.4} $ & $-\phantom{0}2_{-25.0}^{+25.1} $ & $-21_{-30.3}^{+28.5} $ \\
85 & codellama-34b-instruct & $1049_{-5.7}^{+6.0} $ & $-13_{-8.5}^{+8.5} $ & $-\phantom{0}17_{-29.4}^{+31.5} $ & $-19_{-13.2}^{+14.5} $ & $-\phantom{0}8_{-17.2}^{+16.9} $ \\
86 & zephyr-7b-alpha & $1048_{-10.9}^{+10.7} $ & $-\phantom{0}6_{-16.4}^{+16.1} $ & $\phantom{-} \phantom{00}1_{-68.4}^{+68.5} $ & $-27_{-28.5}^{+28.2} $ & $-14_{-32.8}^{+31.9} $ \\
87 & codellama-70b-instruct & $1047_{-13.5}^{+14.6} $ & $-\phantom{0}3_{-22.0}^{+22.8} $ & $\phantom{-} \phantom{0}62_{-37.2}^{+39.8} $ & $\phantom{-} \phantom{0}3_{-28.6}^{+29.9} $ & $\phantom{-} \phantom{0}2_{-36.9}^{+34.8} $ \\
88 & pplx-7b-online & $1045_{-6.6}^{+6.4} $ & $-\phantom{0}6_{-9.6}^{+10.2} $ & $\phantom{-} \phantom{0}47_{-31.8}^{+33.3} $ & $-28_{-14.4}^{+14.7} $ & $-30_{-17.1}^{+17.8} $ \\
89 & gemma-7b-it & $1043_{-5.2}^{+5.3} $ & $-\phantom{0}8_{-8.0}^{+8.3} $ & $\phantom{-} \phantom{0}64_{-15.6}^{+16.0} $ & $\phantom{-} \phantom{0}4_{-11.4}^{+11.8} $ & $\phantom{-} \phantom{0}7_{-12.8}^{+13.7} $ \\
90 & llama-2-7b-chat & $1043_{-4.1}^{+4.1} $ & $\phantom{-} \phantom{0}1_{-6.5}^{+6.3} $ & $-\phantom{0}11_{-15.6}^{+15.9} $ & $-32_{-9.2}^{+9.8} $ & $-38_{-11.7}^{+11.3} $ \\
91 & qwen-14b-chat & $1041_{-6.4}^{+6.8} $ & $-21_{-10.6}^{+10.3} $ & $\phantom{-} \phantom{0}94_{-36.5}^{+34.7} $ & $-16_{-16.8}^{+16.3} $ & $\phantom{-} 16_{-20.5}^{+19.6} $ \\
92 & falcon-180b-chat & $1039_{-13.3}^{+14.1} $ & $-12_{-21.2}^{+20.6} $ & $-\phantom{00}6_{-103.1}^{+79.9} $ & $-38_{-31.7}^{+32.2} $ & $-22_{-43.5}^{+42.0} $ \\
93 & guanaco-33b & $1037_{-9.4}^{+9.1} $ & $-\phantom{0}7_{-13.7}^{+13.0} $ & $-\phantom{00}8_{-37.8}^{+37.5} $ & $-35_{-23.0}^{+23.6} $ & $-69_{-27.9}^{+28.3} $ \\
94 & gemma-1.1-2b-it & $1034_{-4.7}^{+4.5} $ & $-15_{-8.0}^{+8.0} $ & $\phantom{-} \phantom{0}54_{-13.8}^{+13.9} $ & $-15_{-10.6}^{+10.2} $ & $\phantom{-} \phantom{0}8_{-11.1}^{+11.5} $ \\
95 & stripedhyena-nous-7b & $1024_{-6.8}^{+6.8} $ & $-\phantom{0}8_{-9.9}^{+9.9} $ & $\phantom{-} \phantom{0}11_{-36.7}^{+36.3} $ & $-26_{-14.3}^{+14.5} $ & $-21_{-17.9}^{+18.8} $ \\
96 & olmo-7b-instruct & $1021_{-6.0}^{+6.1} $ & $\phantom{-} \phantom{0}0_{-9.7}^{+9.9} $ & $\phantom{-} \phantom{0}62_{-18.5}^{+18.4} $ & $-26_{-13.2}^{+12.5} $ & $-\phantom{0}5_{-16.3}^{+17.3} $ \\
97 & mistral-7b-instruct & $1016_{-5.3}^{+5.6} $ & $-\phantom{0}4_{-8.4}^{+8.1} $ & $-\phantom{00}8_{-25.7}^{+26.1} $ & $-10_{-12.6}^{+11.6} $ & $-\phantom{0}5_{-14.5}^{+15.3} $ \\
98 & palm-2 & $1012_{-5.9}^{+5.7} $ & $-\phantom{0}1_{-8.2}^{+8.7} $ & $-\phantom{0}69_{-32.4}^{+30.6} $ & $-12_{-13.9}^{+14.4} $ & $-22_{-16.6}^{+16.5} $ \\
99 & vicuna-7b & $1012_{-6.2}^{+6.2} $ & $-20_{-9.2}^{+9.4} $ & $\phantom{-} \phantom{0}30_{-27.8}^{+25.6} $ & $-20_{-15.3}^{+15.6} $ & $-27_{-17.3}^{+17.8} $ \\
100 & qwen1.5-4b-chat & $1003_{-5.3}^{+5.5} $ & $-30_{-9.0}^{+9.2} $ & $\phantom{-} \phantom{0}92_{-16.5}^{+15.8} $ & $-21_{-11.5}^{+11.8} $ & $-11_{-14.3}^{+15.6} $ \\
101 & gemma-2b-it & $1000_{-6.8}^{+6.7} $ & $-11_{-11.2}^{+10.7} $ & $\phantom{-} \phantom{0}67_{-21.3}^{+20.8} $ & $-12_{-14.9}^{+14.8} $ & $\phantom{-} \phantom{0}0_{-18.4}^{+18.2} $ \\
102 & koala-13b & $\phantom{0}971_{-6.6}^{+6.5} $ & $-\phantom{0}6_{-9.5}^{+9.9} $ & $-\phantom{0}34_{-25.7}^{+25.9} $ & $-43_{-16.4}^{+16.8} $ & $-30_{-18.9}^{+18.7} $ \\
103 & chatglm3-6b & $\phantom{0}962_{-7.7}^{+7.9} $ & $-11_{-11.2}^{+11.6} $ & $\phantom{-} 159_{-35.2}^{+33.1} $ & $-\phantom{0}7_{-17.0}^{+17.2} $ & $-\phantom{0}9_{-22.3}^{+22.6} $ \\
104 & gpt4all-13b-snoozy & $\phantom{0}941_{-12.2}^{+11.6} $ & $-\phantom{0}4_{-17.0}^{+18.2} $ & $-\phantom{00}6_{-44.9}^{+48.8} $ & $-\phantom{0}6_{-28.5}^{+28.2} $ & $-28_{-37.5}^{+35.3} $ \\
105 & chatglm2-6b & $\phantom{0}936_{-9.8}^{+9.9} $ & $-\phantom{0}7_{-15.0}^{+14.9} $ & $\phantom{-} 120_{-46.3}^{+47.3} $ & $-19_{-23.1}^{+25.1} $ & $-43_{-30.5}^{+29.9} $ \\
106 & mpt-7b-chat & $\phantom{0}935_{-8.2}^{+8.0} $ & $-15_{-11.9}^{+11.4} $ & $\phantom{-} \phantom{0}73_{-32.0}^{+34.0} $ & $-36_{-18.5}^{+20.6} $ & $-28_{-24.7}^{+26.1} $ \\
107 & RWKV-4-Raven-14B & $\phantom{0}929_{-7.7}^{+8.0} $ & $-19_{-11.5}^{+11.4} $ & $\phantom{-} \phantom{0}29_{-30.9}^{+31.6} $ & $-36_{-18.2}^{+18.2} $ & $-30_{-22.2}^{+23.7} $ \\
108 & alpaca-13b & $\phantom{0}911_{-7.2}^{+7.0} $ & $-13_{-10.1}^{+10.3} $ & $-\phantom{0}65_{-30.9}^{+30.4} $ & $-88_{-17.7}^{+18.0} $ & $-117_{-24.0}^{+22.7} $ \\
109 & oasst-pythia-12b & $\phantom{0}902_{-6.8}^{+7.0} $ & $-\phantom{0}9_{-10.9}^{+11.5} $ & $-\phantom{0}41_{-26.6}^{+26.8} $ & $-18_{-16.4}^{+18.1} $ & $-26_{-21.6}^{+22.4} $ \\
110 & chatglm-6b & $\phantom{0}889_{-7.5}^{+7.9} $ & $-25_{-11.6}^{+10.8} $ & $\phantom{-} 252_{-30.3}^{+30.0} $ & $\phantom{-} \phantom{0}9_{-19.4}^{+19.0} $ & $\phantom{-} \phantom{0}1_{-23.3}^{+22.5} $ \\
111 & fastchat-t5-3b & $\phantom{0}879_{-7.9}^{+7.9} $ & $-\phantom{0}1_{-12.0}^{+11.7} $ & $\phantom{-} \phantom{0}22_{-250.3}^{+172.3} $ & $-66_{-19.0}^{+18.6} $ & $-117_{-25.2}^{+25.8} $ \\
112 & stablelm-tuned-alpha-7b & $\phantom{0}851_{-9.2}^{+9.7} $ & $-13_{-14.1}^{+13.3} $ & $\phantom{-} \phantom{0}52_{-31.8}^{+35.9} $ & $-17_{-22.6}^{+23.8} $ & $\phantom{-} 10_{-26.3}^{+27.3} $ \\
113 & dolly-v2-12b & $\phantom{0}828_{-9.3}^{+9.2} $ & $-20_{-13.5}^{+14.0} $ & $\phantom{-} \phantom{0}53_{-35.2}^{+35.2} $ & $-27_{-22.3}^{+23.2} $ & $-78_{-28.5}^{+27.3} $ \\
114 & llama-13b & $\phantom{0}806_{-10.6}^{+10.2} $ & $-23_{-16.7}^{+16.6} $ & $\phantom{-} \phantom{0}47_{-36.2}^{+35.7} $ & $-79_{-27.8}^{+28.7} $ & $-134_{-35.6}^{+35.4} $ \\

\end{longtable}
    }

\end{footnotesize}
